# Supplementary material for: InfoNCE Loss Provably Learns Cluster-Preserving Representations
Source: arXiv:2302.07920 source file (2023-02-15)
Supplement: Supplementary file 1 [file Appendix_SparseCoding.tex]

\section{A Generative Model: Sparse Coding}
In order to concretize our formulation and assumptions, we next study a similar sparse coding model as that used by \citet{wen2022mechanism} to analyze the feature-learning process of contrastive learning. More broadly, sparse coding is a generic generative model that has been employed to model natural image \cite{} and language \cite{arora2018linear} data. In our setting with image data, each image $x$ consists of a  combination of meaningful features plus noise. The combination of meaningful features is determined by a latent vector $z \in \{-1,0,1\}^d$ that has support at least 1, which gives the activation pattern for features in a dictionary $\mathbf{M}\in \mathbb{R}^{D \times d_z}$. For each fixed $\mathbf{z}$, images are generated as follows:
\begin{align}
    x = \mathbf{M} z + \xi, \; \xi \sim \mathcal{N}(0_D,\sigma_\xi^2 \mathbf{I}_D  ) \label{eq:sparsecode1}
\end{align}
% \cite{shi2022theoretical}.
where $\xi$ is white Gaussian noise with covariance $\sigma_\xi^2 = O(\frac{1}{{D} \log^2(D)} )$.
% $\mathcal{D}_z$ is a distribution over $\{-1,0,1\}^d$, 
We are most interested in the regime $D \gg d_z$, although our theory holds for all $D\geq d_z$. For simplicity, we assume the columns (features) of $\mathbf{M}$ are orthonormal. 
% The  and the support of $z$ is at least one.
% and $z$ is drawn drawn from a distribution $\mathcal{D}$
% $\mathcal{D}_z$ is a distribution over $\{-1,1\}^d$. 

Here the content of an image $x$ depends on the presence (or lack thereof) of the dictionary features in $x$. Specifically, the content of ${x}$ is the latent variable $z$ that minimizes the Euclidean distance from $\mathbf{M}z$ to $x$, namely 
% its projection onto the column space of $\mathbf{M}$, i.e. 
$\mathbf{c}(x) := \arg\min_{z\in \{-1,0,1\}^d_z}\|\mathbf{M}z-x\|_2$. Note that the noise covariance is small enough such that all natural images generated from the same latent vector have the same content with high probability.
On the other hand, the style of $x$ is its projection onto the space perpendicular to $\mathbf{Mc}(c)$: $\mathbf{s}(x):= (\mathbf{I}_D- uu^\top )x$ where $u\coloneqq \frac{1}{\|\mathbf{Mc}(x)\|_2}\mathbf{Mc}(x)$. Augmentations of $x$ are sampled such that they only affect the style of $x$, as follows:
% We sample a training dataset consisting of $2\leq n <\infty$ natural images images for each value of $z$. For each natural image, we sample its augmentations as follows:
\begin{align}
    q \sim \text{Unif}(\mathcal{B}_D( {0}_D, \sigma_+^2)), \quad 
    x^+ =  x +  (\mathbf{I}_D - {uu}^\top) q.
\end{align} %\mathbf{M}^\top x \tfrac{2 \sqrt{\log(D)}}{\sqrt{D}} 
where $\mathcal{B}_D( {0}_D, \sigma_+^2) \subset \mathbb{R}^D$ denotes the $D$-dimensional ball with mean $0_D$ and radius $\sigma_{+}^2 = \Theta(\frac{1}{{D} \log^2(D)})$. 
% and $u= \frac{1}{\|\mathbf{M}z\|_2}\mathbf{M}z$. 
In other words, each augmentation set is a disk orthogonal to the column space of $\mathbf{Mc}(x)$,
% $\text{span}(\mathbf{M}z)\subset \text{col}(\mathbf{M})$, 
so $\mathbf{c}(x^+) = \mathbf{c}(x)$ for all positive pairs, consistent with our formulation in Section \ref{section:formulation}. 

% Inspired by \citet{wen2021toward,saunshi2022understanding,haochen2022theoretical},
% who have used different coordinate-wise scaling methods for augmentations, 
% we augment with data via coordinate-wise scaling.
% We then augment images similarly as in  
% Specifically, for each image $x$, we sample augmentations as follows. 
% The $(2i)$-th and $(2i\!+\!1)$-th augmentations are equal to $x^+_{2i} = x - \tau_{i} e_i e_i^\top x$ and $x^+_{2i+1} = x + \tau_{i} e_i e_i^\top x$ where $\tau_i \sim \text{Unif}([0.5,1))$ for all $i\in [d]$. Thus $\mathcal{A}(x)= \{x^+_{j}\}_{j=1}^{2d}$ and a total of $2M d 2^d$ images are in the dataset.
% $m<\infty$ random augmentations sampled by first selecting $a \sim \text{Unif}(a' \in \{0,1\}^d: \|a'\|_1=D/2)$
% and  $v \sim \text{Unif}([0.1,1]^D)$. Then, we compute  $x^+ = a \circ v \circ x$, where $\circ$ denotes element-wise multiplication. 

We consider the classifier function class consisting of linear classifiers, namely $\mathcal{F}_{\text{lin}}\coloneqq \{ \text{sign}( \langle w, \cdot \rangle): w \in \mathbb{R}^D\}$. Thus the representation class is $\mathcal{G}_{\text{lin}}\coloneqq \{ \text{sign}(\mathbf{W}^\top \cdot): \mathbf{W} \in \mathbb{R}^{D\times d}\}$, where here $\text{sign}(\cdot)$ is element-wise. Downstream  tasks are binary classification problems in which labels are functions of the latent feature activation vector $z$, i.e. for task $y$, $y(x) = f_y(z)$. Clusters are determined by  values of ${z}$, with each cluster having mean $\mathbf{M}z$ for some unique $z$. 

% Since $\sigma_{\xi}^2 = O(\tfrac{1}{D \log^2(D)})$ and $\|\mathbf{M}z\|_2 = \Omega(1)$, the clusters are well-separated in $\mathbb{R}^D$.
% % \in \{e_1^N,\dots,e_N^N\}$ where $e_j^N$ is the $j$-th standard basis vector in $\mathbb{R}^N$. 
% In other words,  $\|\mathbf{c}(x)- \mathbf{c}(x')\|_2 = O(\tfrac{1}{{\log(D)}})$ implies $\mathbf{c}(x)\sim \mathbf{c}(x')$ with high probability. 

We would like to learn a representation that clusters images according to their latent variables, and maps these clusters uniformly on the hypercube. First, we show that a uniform and clean representation is realizable in this setting.

% As noted by \cite{wen2021toward}, 
% Without loss of generality we can consider that $\mathbf{M}= [\mathbf{1}_D, \mathbf{1}_D, \dots,  ]$. We aim to recover clusters determined by the values of $z$.
% In this simple setting, we show that 
\begin{lemma}\label{lemma:sc1}
   Consider a dataset in which the number of distinct latent variables is $2^d$ and for each latent variable, there are $n$ natural images sampled according to \eqref{eq:sparsecode1}. Then with high probability over the choice of natural images, there exists a representation $g^*\in \mathcal{G}_{\text{lin}}$ that is clean and uniform.
   % With high probability the clusters do not intersect the coordinate axes, so there exists a clean and uniform representation $\mathbf{W}_\ast = [{e}_1^D,\dots,{e}_d^D]$. 
\end{lemma}

\begin{proof} (Informal, will formalize soon)
Due to the noise variance and the radius of the augmentation disk, the clusters corresponding to each latent variable $z$ are linearly separable by hyperplanes through the origin with high probability over the noise in the natural images.  {\color{red} Next, what condition do the set of $z$'s in the dictionary need to satisfy in order for there to exist a set of hyperplanes that maps the clusters uniformly on $\mathcal{H}_d$? If we consider all $z \in \{-1,1\}^d$ then it is easy to show that a uniform representation exists, but in this case the model is not sparse.}
\end{proof}
{\color{blue} Note: we can make the setting deterministic by considering a fixed dataset in which the natural images are within some radius of the closest $\mathbf{M}z$ and each have distinct projection onto that $\mathbf{M}z$.}

Now we show that our regularity condition on the classification function class holds.
\begin{lemma}\label{lemma:sc2}
    Under the same conditions as in Lemma \ref{lemma:sc1},  $\mathcal{F}$ satisfies Assumption \ref{assump:spiky} with high probability over the choice of natural images.
\end{lemma}
\begin{proof} (Informal, will formalize soon)
    The radius of each augmentation disk is chosen large enough relative to the noise variance such that for each cluster with mean $\mathbf{M}z$, all disks in that cluster intersect the line passing through the origin and $\mathbf{M}z$ with high probability over the noise in each natural image. Therefore, any hyperplane through the origin that passes between two images from the same cluster must also pass through an augmentation disk within that cluster (with high probability over the noise in each natural image). 
\end{proof}
% can't have more than 4 

With these two lemmas in place, we can apply Theorem \ref{thm:uniformandclean}.
\begin{theorem} 
Under the same conditions as in Lemma \ref{lemma:sc1}, optimizing the InfoNCE loss  leads to a clean and uniform representation $g\in \mathcal{G}_{\text{lin}}$ with high probability over the sampling of natural images. 
\end{theorem}
\begin{proof}
    The proof immediately follows from Lemmas \eqref{lemma:sc1} and \eqref{lemma:sc2} and Theorem \ref{thm:uniformandclean}.
\end{proof}

Next we show that if we do not make any assumptions about the function class, we get $\Omega(1)$ downstream task error.
\begin{theorem}
    With unrestricted function class $\mathcal{F}:= \{f : \mathbb{R}^D \rightarrow \{-1,1\} \}$ and $\mathcal{G}:=\mathcal{F}^{\otimes M}$, there exists a representation $\tilde{g}\in \arg \min_{g \in \mathcal{G}} \mathcal{L}(g)$ with \begin{align}
        \max_{T \in \mathcal{T}} \min_{W \in \mathcal{W}} \mathcal{L}_{T}(g,W)  \geq 0.5.
    \end{align}
\end{theorem}
\begin{proof} (Informal, will formalize soon)
    The augmentation sets almost surely do not overlap, so there exists a representation that maps half the images in one cluster to the opposite vertex on the hypercube as the other half of the images in that cluster are mapped to. In fact there exists a representation that splits all clusters onto opposite vertices of the hypercube. Such a mapping entails a pairing of clusters according to the pairs of opposite vertices that they share. Consider the task that labels 1 images from exactly one of the clusters in each pair. It follows that any linear classifier can classify at most half of the images correctly for this task.
\end{proof}

% left off: can get same scaling as wen and li, just make small constant. d << D. just need to figure how to show that assumption spiky holds

% \textbf{}

% \textbf{One-layer neural network with $\pm1$ activation.} Consider 

% two options:
% 1. noise is small relative to elements of M
% 2. 
