# Supplementary material for: InfoNCE Loss Provably Learns Cluster-Preserving Representations
Source: arXiv:2302.07920 source file (2023-02-15)
Supplement: Supplementary file 2 [file notes.tex]

\begin{proof}
For all $v \in \mathcal{H}_d$, define the sets $A_v := \{x \in \mathcal{D}_\circ \cup \mathcal{D} : g(x)=v \}$. 
% $\bar{A}_{v} = \{j\mid g(x_j^-) = v\}$ with $n_{1,v} := |\bar{A}_v| $ (random), 
Note that $\|A_v\|_\circ = D_g(v)$. 

Since $g= [f_1,\dots,f_d]$ is not clean, there exists $j\in [d]$ such that $f_j$ is not clean. WLOG let this $j=1$. Let $S$ denote one of the clusters that $f_1$ intersects. 
Construct $g' =[f_1',f_2,\dots,f_d]$ where $f_1'(x) = f_1(x)$ for all $ x \notin S$. 
Define the set 
 $B := \{x \in \mathcal{D}_\circ \cup \mathcal{D}: f_1(x) \neq f_1'(x) \} \subset S$. 
Let  $f_1'(x) = 1$ or $f_1'(x) = -1$ for all $x \in S$, whichever induces smaller
$\max_v  \|A_v \cup B\|_\circ$.

We would like to show that $\mathcal{L}(g)- \mathcal{L}(g')>0$, where
\begin{align}
    \mathcal{L}(g)- \mathcal{L}(g') = \mathcal{L}_{\text{pos}}(g) - \mathcal{L}_{\text{pos}}(g') + \mathcal{L}_{\text{neg}}(g) - \mathcal{L}_{\text{neg}}(g').
\end{align}
For the positive losses, we have
\begin{align*}
\mathcal{L}_{\text{pos}}(g) - \mathcal{L}_{\text{pos}}(g') &= 
\beta \mathbb{E}_{x, x^+}\left[\left(g'(x)^\top g'(x^+) - g(x)^\top g(x^+)\right)\right] \nonumber \\
&= \beta \mathbb{E}_{x, x^+}\left[\left(f_1'(x) f_1'(x^+) - f_1(x) f_1(x^+)\right)\right] \nonumber \\
&= 2\beta \sum_{v \in \mathcal{A}_v}\left(\Pr\left[x\in A, x^+\in B\right]+\Pr\left[x\in B, x^+\in A\right]\right) 
\end{align*}

Now we consider the negative losses. For a batch of samples $\{x_{i}^-\}_{i=1}^\ell$ and a vertex $v\in \mathcal{H}_d$, let $n_{1,v}:= \sum_{i=1}^\ell \chi\{ x_{i}^- \in A_v \}$ and $n_{2}:= \sum_{i=1}^\ell \chi\{ x_{i}^- \in B \}$.

Recall that the negative loss is given by 
\begin{align*}
{L}_{\text{neg}}(g) 
&= \mathbb{E}_{x,x^+, \{x^-_i\}_{\ell}} \log\bigg({ e^{\beta g(x)^\top g(x^+)}\!+\!\sum_{i=1}^\ell e^{\beta g(x)^\top g(x^-_{i})}  } \bigg) \nonumber \\
&= \sum_{v \in \uH_{d}} \mathbb{E}_{x,x^+, \{x^-_i\}_{\ell}} \chi \{x \in A_v\}  \log\bigg({ e^{\beta g(x)^\top g(x^+)}\!+\!\sum_{i=1}^\ell e^{\beta g(x)^\top g(x^-_{i})}  } \bigg)  \nonumber \\
&= \sum_{v \in \uH_{d}} \mathcal{L}_{\text{neg},v}(g) 
\end{align*}
where $\mathcal{L}_{\text{neg},v}(g)  := \mathbb{E}_{x,x^+, \{x^-_i\}_{\ell}} \chi \{x \in A_v\}  \log\bigg({ e^{\beta g(x)^\top g(x^+)}\!+\!\sum_{i=1}^\ell e^{\beta g(x)^\top g(x^-_{i})}  } \bigg) $.
We need to upper bound $\mathcal{L}_{\text{neg}}(g') - \mathcal{L}_{\text{neg}}(g)$. 
% \begin{enumerate}
% \item In the event that $\{x\in A_v\}$, we have 
Using the notation above, we have
\begin{align*}
\mathcal{L}_{\text{neg,v}}(g) 
&= \mathbb{E}_{x,x^+, \{x^-_i\}_{\ell}}  \chi \{x \in A_v\}  \log\bigg({ e^{\beta g(x)^\top g(x^+)}\!+\!n_{1,v}e^{\beta d}+\sum_{x_i^{-}\not\in {A}_v} e^{\beta g(x)^\top g(x^-_{i})}  } \bigg) \\
&= \mathbb{E}_{x,x^+, \{x^-_i\}_{\ell}}  \chi \{x \in A_v\}  \log\bigg({ e^{\beta g(x)^\top g(x^+)}+n_{1,v}e^{\beta d}+ \sum_{x_i^{-} \in B}e^{\beta g(x)^\top g(x^-_{i})} 
 +\sum_{x_i^{-}\not\in {A}_v\cup B} e^{\beta g(x)^\top g(x^-_{i})}  } \bigg) \\
\end{align*}
\begin{align*}
\mathcal{L}_{\text{neg,v}}(g') & = \mathbb{E}_{x,x^+, \{x^-_i\}_{\ell}}  \chi \{x \in A_v\}  \log\bigg({ e^{\beta g'(x)^\top g'(x^+)}+ n_{1,v}e^{\beta d}+\sum_{x_i^{-}\not\in {A}_v} e^{\beta g'(x)^\top g'(x^-_{i})}  } \bigg) \nonumber \\
& =  \mathbb{E}_{x,x^+, \{x^-_i\}_{\ell}}  \chi \{x \in A_v\} \log\bigg({ e^{\beta g'(x)^\top g'(x^+)}+ n_{1,v}e^{\beta d}+ \sum_{x_i^{-}\in  B} e^{\beta g'(x)^\top g'(x^-_{i})}  +\sum_{x_i^{-}\not\in {A}_v\cup B} e^{\beta g(x)^\top g(x^-_{i})}  } \bigg) \nonumber \\
% &=\mathbb{E}_{x,x^+, \{x^-_i\}_{\ell}}  \chi \{x \in A_v\} \log\bigg({ e^{\beta g'(x)^\top g'(x^+)}+ (n_{1,v} + n_2)e^{\beta d}+\sum_{x_i^{-}\not\in {A}_v\cup B} e^{\beta g(x)^\top g(x^-_{i})}  } \bigg)
\end{align*}

For each $v \in \mathcal{H}_d$, we write
\begin{align}
    &\mathcal{L}_{\text{neg,v}}(g') - \mathcal{L}_{\text{neg,v}}(g) \nonumber \\
    &\leq  \mathbb{E}_{x,x^+, \{x^-_i\}_{\ell}}  \chi \{x \in A_v\}\chi\{n_2=0\} \log\bigg({ e^{\beta g'(x)^\top g'(x^+)}+ n_{1,v}e^{\beta d}+ \sum_{x_i^{-}\in  B} e^{\beta g'(x)^\top g'(x^-_{i})}  +\sum_{x_i^{-}\not\in {A}_v\cup B} e^{\beta g(x)^\top g(x^-_{i})}  } \bigg) \nonumber \\
    &\quad \quad  - \mathbb{E}_{x,x^+, \{x^-_i\}_{\ell}}  \chi \{x \in A_v\} \chi\{n_2=0\} \log\bigg({ e^{\beta g(x)^\top g(x^+)}+n_{1,v}e^{\beta d}+ \sum_{x_i^{-} \in B}e^{\beta g(x)^\top g(x^-_{i})} 
 +\sum_{x_i^{-}\not\in {A}_v\cup B} e^{\beta g(x)^\top g(x^-_{i})}  } \bigg) \nonumber \\
 &\quad +  \mathbb{E}_{x,x^+, \{x^-_i\}_{\ell}}  \chi \{x \in A_v\}\chi\{n_2>0,n_{1,v}=0\} \nonumber \\
 &\quad\quad\quad \log\bigg({ e^{\beta g'(x)^\top g'(x^+)}+ n_{1,v}e^{\beta d}+ \sum_{x_i^{-}\in  B} e^{\beta g'(x)^\top g'(x^-_{i})}  +\sum_{x_i^{-}\not\in {A}_v\cup B} e^{\beta g(x)^\top g(x^-_{i})}  } \bigg) \nonumber \\
    &\quad \quad  - \mathbb{E}_{x,x^+, \{x^-_i\}_{\ell}}  \chi \{x \in A_v\} \chi\{n_2>0,n_{1,v}=0\} \nonumber \\
    &\quad \quad \quad \log\bigg({ e^{\beta g(x)^\top g(x^+)}+n_{1,v}e^{\beta d}+ \sum_{x_i^{-} \in B}e^{\beta g(x)^\top g(x^-_{i})} 
 +\sum_{x_i^{-}\not\in {A}_v\cup B} e^{\beta g(x)^\top g(x^-_{i})}  } \bigg) \nonumber \\
 &\quad \quad +  \mathbb{E}_{x,x^+, \{x^-_i\}_{\ell}}  \chi \{x \in A_v\}\chi\{n_2>0,n_{1,v}>0\} \nonumber \\
 &\quad\quad \quad  \log\bigg({ e^{\beta g'(x)^\top g'(x^+)}+ n_{1,v}e^{\beta d}+ \sum_{x_i^{-}\in  B} e^{\beta g'(x)^\top g'(x^-_{i})}  +\sum_{x_i^{-}\not\in {A}_v\cup B} e^{\beta g(x)^\top g(x^-_{i})}  } \bigg) \nonumber \\
    &\quad \quad - \mathbb{E}_{x,x^+, \{x^-_i\}_{\ell}}  \chi \{x \in A_v\} \chi\{n_2>0,n_{1,v}>0\} \nonumber \\
    &\quad \quad \quad  \log\bigg({ e^{\beta g(x)^\top g(x^+)}+n_{1,v}e^{\beta d}+ \sum_{x_i^{-} \in B}e^{\beta g(x)^\top g(x^-_{i})} 
 +\sum_{x_i^{-}\not\in {A}_v\cup B} e^{\beta g(x)^\top g(x^-_{i})}  } \bigg) \nonumber 
\end{align}
and consider each of the three differences individually.
\begin{enumerate}
\item $n_2 = 0$. 

% increases by at most $2\beta $ due to positive pair, and that increase happens with total probability $\Delta_f^{new}$ after summing over all $v$. So we need to lower bound the other terms in the log. The bad case is if $n_{1,v}$ is zero, but this happens with small probability. Use:
In this case we have
\begin{align}
    % \tilde{L}_{\text{neg}}(g') -\tilde{L}_{\text{neg}}(g) 
    &\mathbb{E}_{x,x^+, \{x^-_i\}_{\ell}}  \chi \{x \in A_v\}\chi \{n_2 = 0\}  \log\bigg({ e^{\beta g'(x)^\top g'(x^+)}+ n_{1,v}e^{\beta d}  +\sum_{x_i^{-}\not\in {A}_v\cup B} e^{\beta g(x)^\top g(x^-_{i})}  } \bigg) \nonumber \\
    &\quad - \mathbb{E}_{x,x^+, \{x^-_i\}_{\ell}}  \chi \{x \in A_v\}\chi \{n_2 = 0\}   \log\bigg({ e^{\beta g(x)^\top g(x^+)}+n_{1,v}e^{\beta d}
 +\sum_{x_i^{-}\not\in {A}_v\cup B} e^{\beta g(x)^\top g(x^-_{i})}  } \bigg)  \label{dif1} \\
 &\leq \mathbb{E}_{x,x^+, \{x^-_i\}_{\ell}}  \chi \{x \in A_v\} \chi \{n_2 = 0\} \log\bigg({ e^{\beta g'(x)^\top g'(x^+)}+ n_{1,v}e^{\beta d}   } \bigg) \nonumber \\
 &\quad - \mathbb{E}_{x,x^+, \{x^-_i\}_{\ell}}  \chi \{x \in A_v\} \chi \{n_2 = 0\}  \log\bigg({ e^{\beta g(x)^\top g(x^+)}+n_{1,v}e^{\beta d}  } \bigg)  \label{subm} \\
  &= \mathbb{E}_{x,x^+, \{x^-_i\}_{\ell}}  \chi \{x \in A_v\}  \chi \{x^+ \in B\} \chi \{n_2 = 0\}  \log\bigg({ e^{2\beta }e^{\beta g(x)^\top g(x^+)}+ n_{1,v}e^{\beta d}   } \bigg) \nonumber \\
 &\quad - \mathbb{E}_{x,x^+, \{x^-_i\}_{\ell}}  \chi \{x \in A_v\} \chi \{x^+ \in B\} \chi \{n_2 = 0\} \log\bigg({ e^{\beta g(x)^\top g(x^+)}+n_{1,v}e^{\beta d}  } \bigg)  \nonumber \\
 &\leq \mathbb{E}_{x,x^+, \{x^-_i\}_{\ell}}  \chi \{x \in A_v\}\chi \{x^+ \in B\} \chi \{n_2 = 0\}  \log\bigg({ e^{\beta d}+ n_{1,v}e^{\beta d}   } \bigg) \nonumber \\
 &\quad - \mathbb{E}_{x,x^+, \{x^-_i\}_{\ell}}  \chi \{x \in A_v\} \chi \{x^+ \in B\} \chi \{n_2 = 0\}  \log\bigg({ e^{\beta (d-2)}+n_{1,v}e^{\beta d}  } \bigg) \label{hh} \\
 &= \mathbb{E}_{x,x^+, \{x^-_i\}_{\ell}}  \chi \{x \in A_v\} \chi \{x^+ \in B\} \chi \{n_2 = 0\}  \log\bigg(\frac{1+ n_{1,v}   }{e^{-2\beta }+n_{1,v}} \bigg) \nonumber \\
 &=  \mathbb{E}_{x,x^+, \{x^-_i\}_{\ell}}  \chi \{x \in A_v\} \chi \{x^+ \in B\} \chi \{n_2 = 0\}  \chi\{ n_{1,v}=0 \} \log\bigg(\frac{1+ n_{1,v}   }{e^{-2\beta }+n_{1,v}} \bigg) \nonumber \\
 &\quad + \mathbb{E}_{x,x^+, \{x^-_i\}_{\ell}}  \chi \{x \in A_v\} \chi \{x^+ \in B\} \chi \{n_2 = 0\}  \chi\{ n_{1,v}>0 \} \log\bigg(\frac{1+ n_{1,v}   }{e^{-2\beta }+n_{1,v}} \bigg) \nonumber \\
 &\leq 2 \beta \mathbb{E}_{x,x^+, \{x^-_i\}_{\ell}}  \chi \{x \in A_v\} \chi \{x^+ \in B\} \chi \{n_2 = 0\}  \chi\{ n_{1,v}=0 \} \nonumber \\
 &\quad + \log(2 ) \mathbb{E}_{x,x^+, \{x^-_i\}_{\ell}}  \chi \{x \in A_v\} \chi \{x^+ \in B\} \chi \{n_2 = 0\}  \chi\{ n_{1,v}>0 \}  \nonumber 
\end{align}
where \eqref{subm} follows by the submodularity of $\log$ and the fact that $g'(x)^\top g'(x^+)\geq g(x)^\top g(x^+)$ by construction of $g'$, and \eqref{hh} follows since $h(x):= \frac{yx+ c}{x+c}$ is monotonically increasing for $y> 1$.
Next, by the independence of $x_i^-$ from $x$ and $x^+$, 
\begin{align}
    &\mathbb{E}_{x,x^+, \{x^-_i\}_{\ell}}   \chi \{x \in A_v\} \chi \{x^+ \in B\}\chi \{n_2 = 0\} \chi\{ n_{1,v}=0 \}  \nonumber \\
    &=  \mathbb{P}(x \in A_v \cap x^+ \in B) \mathbb{P}(n_{1,v}=0) \\
    &= \mathbb{P}(x \in A_v \cap x^+ \in B) D_g(v)(1 - D_g(v) - \|B\|_0)^\ell \\
    & \mathbb{E}_{x,x^+, \{x^-_i\}_{\ell}}  \chi \{x \in A_v\}\chi \{x^+ \in B\} \chi \{n_2 = 0\}  \chi\{ n_{1,v}>0 \} \nonumber \\
    &= \mathbb{P}(x \in A_v \cap x^+ \in B) \mathbb{P}(n_{1,v}>0) \\
     &\leq \mathbb{P}(x \in A_v \cap x^+ \in B) D_g(v)
\end{align}
So in total, \eqref{dif1} is upper bounded by
\begin{align}
        \mathbb{P}(x \in A_v \cap x^+ \in B) ( 2 \beta D_g(v)(1 - D_g(v) - \|B\|_0)^\ell + \log(2) D_g(v)).
\end{align}
% which is fine.

\item $n_{1,v} = 0, n_2 > 0$ 

% then $\tilde{L}_{\text{neg}}$ increases by at most $2\beta$ (since each term in the argument of the $\log$ can increase by no more than a multiplicative factor of $2\beta$). This happens with probability $(1-D_g(i))^l l\Vert B\Vert_\circ$, that is, there is a probability $(1-D_g(i))^l$ that no negative sample is sampled from the same cluster, and a probability $l\delta$ that $n_2 > 0$.  

In this case we have:
    \begin{align}
    % \tilde{L}_{\text{neg}}(g') -\tilde{L}_{\text{neg}}(g) 
    &\mathbb{E}_{x,x^+, \{x^-_i\}_{\ell}}  \chi \{x \in A_v,n_{1,v} = 0,n_2 > 0\} \nonumber \\
    &\quad \log\bigg({ e^{\beta g'(x)^\top g'(x^+)}+ n_{1,v}e^{\beta d} + \sum_{x_i^{-} \in B}e^{\beta g'(x)^\top g'(x^-_{i})}  +\sum_{x_i^{-}\not\in {A}_v\cup B} e^{\beta g(x)^\top g(x^-_{i})}  } \bigg) \nonumber \\
    &\quad - \mathbb{E}_{x,x^+, \{x^-_i\}_{\ell}}  \chi \{x \in A_v,n_{1,v} = 0,n_2 > 0\}   \nonumber \\
    &\quad \quad \log\bigg({ e^{\beta g(x)^\top g(x^+)}+n_{1,v}e^{\beta d}
+ \sum_{x_i^{-} \in B}e^{\beta g(x)^\top g(x^-_{i})}  +\sum_{x_i^{-}\not\in {A}_v\cup B} e^{\beta g(x)^\top g(x^-_{i})}  } \bigg)  \label{dif2} \\
 &=  \mathbb{E}_{x,x^+, \{x^-_i\}_{\ell}}  \chi \{x \in A_v,n_{1,v} = 0,n_2 > 0\}  \log\bigg({ e^{\beta g'(x)^\top g'(x^+)} + \sum_{x_i^{-} \in B}e^{\beta g'(x)^\top g'(x^-_{i})} +\sum_{x_i^{-}\not\in {A}_v\cup B} e^{\beta g(x)^\top g(x^-_{i})}  } \bigg) \nonumber \\
    &\quad - \mathbb{E}_{x,x^+, \{x^-_i\}_{\ell}}  \chi \{x \in A_v,n_{1,v} = 0,n_2 > 0\}   \log\bigg({ e^{\beta g(x)^\top g(x^+)}
 + \sum_{x_i^{-} \in B}e^{\beta g(x)^\top g(x^-_{i})} +\sum_{x_i^{-}\not\in {A}_v\cup B} e^{\beta g(x)^\top g(x^-_{i})}  } \bigg)  \\
  &\leq  \mathbb{E}_{x,x^+, \{x^-_i\}_{\ell}}  \chi \{x \in A_v,n_{1,v} = 0,n_2 > 0\}  \log\bigg({ e^{\beta g'(x)^\top g'(x^+)} + \sum_{x_i^{-} \in B}e^{\beta g'(x)^\top g'(x^-_{i})} } \bigg) \nonumber \\
    &\quad - \mathbb{E}_{x,x^+, \{x^-_i\}_{\ell}}  \chi \{x \in A_v,n_{1,v} = 0,n_2 > 0\}   \log\bigg({ e^{\beta g(x)^\top g(x^+)}
 + \sum_{x_i^{-} \in B}e^{\beta g(x)^\top g(x^-_{i})}  } \bigg)  \\
 &\leq 2 \beta \log(\ell+1) \mathbb{P}(x \in A_v) \mathbb{E}_{ \{x^-_i\}_{\ell}}  [\chi \{n_{1,v} = 0\}\chi \{n_2 > 0\}] \nonumber \\
 &= 2 \beta \log(\ell+1) \mathbb{P}(x \in A_v) \mathbb{E}_{ \{x^-_i\}_{\ell}} [ \chi \{\cap_i x_{i}^- \notin A_v\}\chi \{\cup_i x_{i}^- \in B\} ] \nonumber \\
 &=  2 \beta \log(\ell+1) \mathbb{P}(x \in A_v) \mathbb{P} ( \cup_i x_{i}^- \in B | \cap_i x_{i}^- \notin A_v)\mathbb{P}(\cap_i x_{i}^- \notin A_v) \nonumber \\
 &\leq 2 \beta \log(\ell+1) \mathbb{P}(x \in A_v) \mathbb{P}(\cap_i x_{i}^- \notin A_v)  \sum_i \mathbb{P} ( x_{i}^- \in B |  x_{i}^- \notin A_v) \nonumber \\
 &= 2 \beta \ell \log(\ell+1) D_g(v) (1 - D_g(v))^\ell  \mathbb{P} ( x_{1}^- \in B |  x_{1}^- \notin A_v).
\end{align}
% where \eqref{}

\item $n_1, n_2 > 0$.

We have
\begin{align}
&\mathbb{E}  \bigg[\chi \{x \in A_v,n_{1,v} > 0,n_2 > 0\} \nonumber \\
&\quad \quad \quad \log\bigg({ e^{\beta g'(x)^\top g'(x^+)}+ n_{1,v}e^{\beta d} + \sum_{x_i^{-} \in B}e^{\beta g'(x)^\top g'(x^-_{i})}  +\sum_{x_i^{-}\not\in {A}_v\cup B} e^{\beta g(x)^\top g(x^-_{i})}  } \bigg) \bigg]\nonumber \\
    &\quad - \mathbb{E} \bigg[\chi \{x \in A_v,n_{1,v} > 0,n_2 > 0\} \nonumber \\
    &\quad \quad\quad \log\bigg({ e^{\beta g(x)^\top g(x^+)}+n_{1,v}e^{\beta d}
+ \sum_{x_i^{-} \in B}e^{\beta g(x)^\top g(x^-_{i})}  +\sum_{x_i^{-}\not\in {A}_v\cup B} e^{\beta g(x)^\top g(x^-_{i})}  } \bigg) \bigg] \label{dif3} \\
&\leq \mathbb{E}  \left[\chi \{x \in A_v,n_{1,v} > 0,n_2 > 0\}  \log\bigg({ e^{\beta g'(x)^\top g'(x^+)}+ n_{1,v}e^{\beta d} + \sum_{x_i^{-} \in B}e^{\beta g'(x)^\top g'(x^-_{i})}   } \bigg) \right]\nonumber \\
    &\quad - \mathbb{E} \left[\chi \{x \in A_v,n_{1,v} > 0,n_2 > 0\}   \log\bigg({ e^{\beta g(x)^\top g(x^+)}+n_{1,v}e^{\beta d}
+ \sum_{x_i^{-} \in B}e^{\beta g(x)^\top g(x^-_{i})}    } \bigg) \right] \\
&\leq \mathbb{E}  \left[\chi \{x \in A_v,n_{1,v} > 0,n_2 > 0\}  \log\bigg({ e^{\beta g'(x)^\top g'(x^+)}+ (n_{1,v}+n_2)e^{\beta d}  } \bigg) \right]\nonumber \\
    &\quad - \mathbb{E} \left[\chi \{x \in A_v,n_{1,v} > 0,n_2 > 0\}   \log\bigg({ e^{\beta g(x)^\top g(x^+)}+n_{1,v}e^{\beta d} + n_2e^{\beta (d-2)}
  } \bigg) \right] \\
  &= \mathbb{E}  \left[\chi \{x \in A_v,n_{1,v} > 0,n_2 > 0,  g'(x)^\top g'(x^+) =  g(x)^\top g(x^+) \}  \log\bigg({ e^{\beta g'(x)^\top g'(x^+)}+ (n_{1,v}+n_2)e^{\beta d}  } \bigg) \right]\nonumber \\
    &\quad - \mathbb{E} \left[\chi \{x \in A_v,n_{1,v} > 0,n_2 > 0,  g'(x)^\top g'(x^+) =  g(x)^\top g(x^+)\} \nonumber \\
    &\quad \quad \log\bigg({ e^{\beta g(x)^\top g(x^+)}+n_{1,v}e^{\beta d} + n_2e^{\beta (d-2)}
  } \bigg) \right] \\
  &\quad +  \mathbb{E}  \left[\chi \{x \in A_v,n_{1,v} > 0,n_2 > 0,  g'(x)^\top g'(x^+) \neq  g(x)^\top g(x^+) \} \nonumber \\
  &\quad \quad \log\bigg({ e^{\beta g'(x)^\top g'(x^+)}+ (n_{1,v}+n_2)e^{\beta d}  } \bigg) \right]\nonumber \\
    &\quad - \mathbb{E} \left[\chi \{x \in A_v,n_{1,v} > 0,n_2 > 0,  g'(x)^\top g'(x^+) \neq   g(x)^\top g(x^+)\}  \nonumber \\
    &\quad \quad \log\bigg({ e^{\beta g(x)^\top g(x^+)}+n_{1,v}e^{\beta d} + n_2e^{\beta (d-2)}
  } \bigg) \right] 
  \end{align}
  Denote by $(*)$ the expression in \eqref{dif3}. Continuing from above, we have
  \begin{align}
  (*) &\leq \mathbb{E}  \left[\chi \{x \in A_v,n_{1,v} > 0,n_2 > 0,  g'(x)^\top g'(x^+) =  g(x)^\top g(x^+) \}  \log\bigg({  \frac{n_{1,v}+n_2}{n_{1,v}} } \bigg) \right]\nonumber \\
    % &\quad - \mathbb{E} \left[\chi \{x \in A_v,n_{1,v} > 0,n_2 > 0,  g'(x)^\top g'(x^+) =  g(x)^\top g(x^+)\}   \log\bigg({ n_{1,v}e^{\beta d} + n_2e^{\beta (d-2)}
  % } \bigg) \right] \\
  &\quad +  \mathbb{E}  \left[\chi \{x \in A_v,n_{1,v} > 0,n_2 > 0,  g'(x)^\top g'(x^+) \neq  g(x)^\top g(x^+) \}  \log\bigg(\frac{  n_{1,v}+n_2+1  }{n_{1,v} } \bigg) \right]\nonumber \\
  &\leq  \mathbb{E}  \left[\chi \{x \in A_v,n_{1,v} > 0,n_2 > 0,  g'(x)^\top g'(x^+) =  g(x)^\top g(x^+) \}  \frac{2n_2}{n_{1,v}+1} \right]\nonumber \\
    % &\quad - \mathbb{E} \left[\chi \{x \in A_v,n_{1,v} > 0,n_2 > 0,  g'(x)^\top g'(x^+) =  g(x)^\top g(x^+)\}   \log\bigg({ n_{1,v}e^{\beta d} + n_2e^{\beta (d-2)}
  % } \bigg) \right] \\
  &\quad +  \mathbb{E}  \left[\chi \{x \in A_v,n_{1,v} > 0,n_2 > 0,  g'(x)^\top g'(x^+) \neq  g(x)^\top g(x^+) \}  \frac{  2n_2+2  }{n_{1,v}+1 } \right]\nonumber \\
  &= \mathbb{E}  \left[\chi \{x \in A_v,n_{1,v} > 0,n_2 > 0\}  \frac{2n_2}{n_{1,v}+1}  \right]\nonumber \\
    % &\quad - \mathbb{E} \left[\chi \{x \in A_v,n_{1,v} > 0,n_2 > 0,  g'(x)^\top g'(x^+) =  g(x)^\top g(x^+)\}   \log\bigg({ n_{1,v}e^{\beta d} + n_2e^{\beta (d-2)}
  % } \bigg) \right] \\
  &\quad +  \mathbb{E}  \left[\chi \{x \in A_v,n_{1,v} > 0,n_2 > 0,  g'(x)^\top g'(x^+) \neq  g(x)^\top g(x^+) \}  \frac{  2  }{n_{1,v}+1 } \right]\nonumber \\
  &= \mathbb{E}  \left[\chi \{x \in A_v,n_{1,v} > 0,n_2 > 0, A_v\cap B= \emptyset \}  \frac{2n_2}{n_{1,v}+1}  \right]\nonumber \\
  &\quad + \mathbb{E}  \left[\chi \{x \in A_v,n_{1,v} > 0,n_2 > 0, A_v\cap B\neq \emptyset \}  \frac{2n_2}{n_{1,v}+1}  \right]\nonumber \\
  &\quad +  \mathbb{E}  \left[\chi \{x \in A_v,n_{1,v} > 0,n_2 > 0,  g'(x)^\top g'(x^+) \neq  g(x)^\top g(x^+), A_v\cap B= \emptyset \}  \frac{  2  }{n_{1,v}+1 } \right]\nonumber \\
  &\quad +  \mathbb{E}  \left[\chi \{x \in A_v,n_{1,v} > 0,n_2 > 0,  g'(x)^\top g'(x^+) \neq  g(x)^\top g(x^+), A_v\cap B\neq \emptyset \}  \frac{  2  }{n_{1,v}+1 } \right]\label{4terms}
\end{align}
where the second inequality follows using the inequality $\log(1+x)\leq x$. 
Thus we are left with four terms in \eqref{4terms}.
For the first term  we have (there is notation overload: after the first line, $n_{1,v}$ and $n_2$ change from random variables to dummy variables):
% For the first term ,
\begin{align}
    &\mathbb{E}  \left[\chi \{x \in A_v,n_{1,v} > 0,n_2 > 0,A_v\cap B= \emptyset \}  \frac{2n_2}{n_{1,v}+1} \right] \nonumber \\
    &= \mathbb{P}(x \in A_v) \sum_{n_{1,v},n_2: n_{1,v}+n_2\leq \ell }  \chi \{n_{1,v} > 0,n_2 > 0\} \binom{l}{n_{1,v}~n_2~1\!-\!n_{1,v}\!-\!n_2} \nonumber \\
    &\quad \quad \quad \quad  \Vert A_v\Vert_\circ^{n_{1,v}}\Vert B\Vert_\circ^{n_2}\Vert 1-A_v-B\Vert_\circ^{1-n_{1,v}-n_2}\frac{2n_2}{n_{1,v}+1} \\
    &= 2\mathbb{P}(x \in A_v)\sum_{n_{1,v},n_2: n_{1,v},n_2>0, n_{1,v}+n_2\leq \ell}  \binom{l}{n_{1,v}~n_2~1\!-\!n_{1,v}\!-\!n_2} \nonumber \\
    &\quad \quad \quad \quad \Vert A_v\Vert_\circ^{n_{1,v}}\Vert B\Vert_\circ^{n_2}\Vert 1-A_v-B\Vert_\circ^{1-n_{1,v}-n_2}\frac{n_2}{n_{1,v}+1} \\
    &= 2 D_g(v) \frac{\|B\|_\circ}{\|A_v\|_\circ} \sum_{n_{1,v},n_2: n_{1,v},n_2>0, n_{1,v}+n_2\leq \ell}    \binom{l}{n_{1,v}+1~n_2-1~1\!-\!n_{1,v}\!-\!n_2} \nonumber \\
    &\quad \quad \quad \quad \Vert A_v\Vert_\circ^{n_{1,v}+1}\Vert B\Vert_\circ^{n_2-1}\Vert 1-A_v-B\Vert_\circ^{1- n_{1,v}-n_2} \\
    &\leq 2 D_g(v) \frac{\|B\|_\circ}{\|A_v\|_\circ} \!\sum_{n_{1,v}\!+\!1,n_2\!-\!1: n_{1,v}\!+\!1,n_2-\!1\!\geq\!0, n_{1,v}+1\!+\!n_2-1\!\leq\! \ell}   \binom{l}{n_{1,v}\!+\!1~n_2\!-\!1~1\!-(n_{1,v}\!+\!1) \!-\! (n_2\!-\!1)}\nonumber \\
    &\quad \quad \quad \quad \quad \quad \quad \quad \quad \quad \quad\quad \quad \quad \quad  \quad \quad \quad \quad  \quad \quad \quad \Vert A_v\Vert_\circ^{n_{1,v}\!+\!1}\Vert B\Vert_\circ^{n_2\!-\!1}\Vert 1\!-\!A_v\!-\!B\Vert_\circ^{1 \!-\! (n_{1,v}\!+\!1)\! -\! (n_2\!-\!1)}  \label{sq}\\
    &= 2{\|B\|_\circ} ( \Vert A_v\Vert_\circ + \Vert B\Vert_\circ + \Vert 1-A_v-B\Vert_\circ)^\ell  \nonumber \\
    &= {2 {\|B\|_\circ}}   \nonumber 
\end{align}
where in \eqref{sq} we have added terms to the sum to complete the trinomial expansion, and the last equality follows since $A_v$ and $B$ are disjoint.

For the second term in \eqref{4terms}, let $n_{3,v} := \sum_i \chi\{x_i^- \in A_v \cap B\}$, $n_{4,v} := \sum_i \chi\{x_i^- \in A_v \setminus B\}$, $n_{5,v} := \sum_i \chi\{x_i^- \in B \setminus A_v\}$ and let $n_{6,v} = 1 - n_{3,v}+n_{4,v}+n_{5,v}$. Note $n_{1,v} = n_{3,v} + n_{4,v}$, $n_2 = n_{3,v} + n_{5,v}$. 

Observe that at least one of  $\|A_v \cap B\|_\circ$, $\|A_v \setminus B\|_\circ$ has measure at least $1/2 \|A_v\|_\circ$. In particular $\{\|A_v \cap B\|_\circ > \|A_v \|_\circ /2\} \cap \{\|A_v \setminus B\|_\circ\geq \|A_v\|_\circ /2\} = \emptyset$ and $\{\|A_v \cap B\|_\circ > \|A_v \|_\circ /2\} \cup \{\|A_v \setminus B\|_\circ\geq \|A_v\|_\circ /2\} = U=$ Universal set. So we have
\begin{align}
    &\mathbb{E}  \left[\chi \{x \in A_v,n_{1,v} > 0,n_2 > 0,A_v\cap B\neq \emptyset \}  \frac{2n_2}{n_{1,v}+1} \right] \nonumber \\
    &=\mathbb{E}  \left[\chi \{x \in A_v,n_{1,v} > 0,n_2 > 0,A_v\cap B\neq \emptyset, \|A_v\setminus B\|_\circ \geq \|A_v\|_\circ/2 \}  \frac{2n_2}{n_{1,v}+1} \right] \nonumber \\
    &\quad + \mathbb{E}  \left[\chi \{x \in A_v,n_{1,v} > 0,n_2 > 0,A_v\cap B\neq \emptyset, \|A_v\cap B\|_\circ > \|A_v\|_\circ/2 \}  \frac{2n_2}{n_{1,v}+1} \right]  \label{onehalf}
    \end{align}

    For term 1 in \eqref{onehalf} we have
    \begin{align}
    &\mathbb{E}  \left[\chi \{x \in A_v,n_{1,v} > 0,n_2 > 0,A_v\cap B\neq \emptyset, \|A_v\setminus B\|_\circ \geq \|A_v\|_\circ/2 \}  \frac{2n_2}{n_{1,v}+1} \right] \nonumber \\
    &= D_g(v) \nonumber \\
    &\quad \sum_{n_{3,v}+n_{4,v}+n_{5,v}+n_{6,v}=\ell} \chi \{n_{3,v} +n_{4,v}> 0,n_{3,v} +n_{5,v}> 0, \|A_v\!\setminus\! B\|_\circ \geq \|A_v\|_\circ/2  \}  \binom{l}{n_{3,v}~n_{4,v}~n_{5,v}~n_{6,v}} \nonumber \\
    &\quad \quad \quad \quad  \quad \quad \quad \quad \Vert A_v\cap B\Vert_\circ^{n_{3,v}}\Vert A_v\setminus B\Vert_\circ^{n_{4,v}}\Vert B\setminus A_v\Vert_\circ^{n_{5,v}} (1-\Vert  B \cup A_v\Vert_\circ)^{n_{6,v}} \frac{2(n_{3,v} + n_{5,v})}{n_{3,v} + n_{4,v}+1} \nonumber \\
    &\leq  2 D_g(v) \nonumber \\
    &\quad \sum_{n_{3,v}+n_{4,v}+n_{5,v}+n_{6,v}=\ell} \chi \{n_{3,v} +n_{4,v}> 0,n_{3,v} +n_{5,v}> 0, \|A_v\!\setminus\! B\|_\circ \geq \|A_v\|_\circ/2\}  \binom{l}{n_{3,v}~n_{4,v}~n_{5,v}~n_{6,v}} \nonumber \\
    &\quad \quad \quad \quad  \quad \quad \quad \quad \Vert A_v\cap B\Vert_\circ^{n_{3,v}}\Vert A_v\setminus B\Vert_\circ^{n_{4,v}}\Vert B\setminus A_v\Vert_\circ^{n_{5,v}} (1-\Vert  B \cup A_v\Vert_\circ)^{n_{6,v}} \frac{n_{3,v} + n_{5,v}}{n_{4,v}+1}  \nonumber \\
    &= 2 D_g(v) \sum_{n_{3,v}+n_{4,v}+n_{5,v}+n_{6,v}=\ell} \chi \{n_{3,v}=0, n_{4,v}> 0, n_{5,v}> 0, \|A_v\!\setminus\! B\|_\circ \geq \|A_v\|_\circ/2\}  \binom{l}{n_{4,v}~n_{5,v}~n_{6,v}} \nonumber \\
    &\quad \quad \quad \quad  \quad \quad \quad \quad \Vert A_v\setminus B\Vert_\circ^{n_{4,v}}\Vert B\setminus A_v\Vert_\circ^{n_{5,v}} (1-\Vert  B \cup A_v\Vert_\circ)^{n_{6,v}} \frac{n_{5,v}}{n_{4,v}+1} \nonumber \\
    &\quad + 2 D_g(v) \sum_{n_{3,v}+n_{4,v}+n_{5,v}+n_{6,v}=\ell} \chi \{n_{3,v}>0,\|A_v\!\setminus\! B\|_\circ \geq \|A_v\|_\circ/2\}  \binom{l}{n_{3,v}~n_{4,v}~n_{5,v}~n_{6,v}} \nonumber \\
    &\quad \quad \quad \quad  \quad \quad \quad \quad \Vert A_v\cap B\Vert_\circ^{n_{3,v}}\Vert A_v\setminus B\Vert_\circ^{n_{4,v}}\Vert B\setminus A_v\Vert_\circ^{n_{5,v}} (1-\Vert  B \cup A_v\Vert_\circ)^{n_{6,v}} \frac{n_{3,v} + n_{5,v}}{n_{4,v}+1} \label{32}
\end{align}

For the first term above ($n_{3,v}=0$), we rearrange $ \frac{n_{5,v}}{n_{4,v}+1}$ and complete the multinomial.
\begin{align}
    &2 D_g(v) \sum_{n_{3,v}+n_{4,v}+n_{5,v}+n_{6,v}=\ell} \chi \{n_{3,v}=0, n_{4,v}> 0, n_{5,v}> 0,\|A_v\!\setminus\! B\|_\circ \geq \|A_v\|_\circ/2\}  \binom{l}{n_{4,v}~n_{5,v}~n_{6,v}} \nonumber \\
    &\quad \quad \quad \quad  \quad \quad \quad \quad \Vert A_v\setminus B\Vert_\circ^{n_{4,v}}\Vert B\setminus A_v\Vert_\circ^{n_{5,v}} (1-\Vert  B \cup A_v\Vert_\circ)^{n_{6,v}} \frac{n_{5,v}}{n_{4,v}+1} \\
    &= 2 D_g(v) \sum_{n_{4,v}+n_{5,v}+n_{6,v}=\ell, 0<n_{4,v}<\ell,0<n_{5,v}<\ell} \chi \{ \|A_v\!\setminus\! B\|_\circ \geq \|A_v\|_\circ/2\}  \binom{l}{n_{4,v}~n_{5,v}~n_{6,v}} \nonumber \\
    &\quad \quad \quad \quad  \quad \quad \quad \quad \Vert A_v\setminus B\Vert_\circ^{n_{4,v}}\Vert B\setminus A_v\Vert_\circ^{n_{5,v}} (1-\Vert  B \cup A_v\Vert_\circ)^{n_{6,v}} \frac{n_{5,v}}{n_{4,v}+1} \\
    &= 2 D_g(v) \chi\{\|A_v\!\setminus\! B\|_\circ \geq \|A_v\|_\circ/2\} \frac{\Vert B\setminus A_v\Vert_\circ}{\Vert A_v\setminus B\Vert_\circ} \nonumber \\
    &\quad \sum_{(n_{4,v}+1)\geq 2,(n_{5,v}-1)\geq 0, (n_{4,v}+1)+(n_{5,v}-1)\leq\ell, n_{4,v}+1\leq \ell, n_{5,v}-1\leq \ell-2}   \binom{l}{n_{4,v}+1~n_{5,v}-1~n_{6,v}} \nonumber \\
    &\quad \quad \quad \quad  \quad \quad \quad \quad\quad \quad \quad \quad \quad \quad \Vert A_v\setminus B\Vert_\circ^{n_{4,v}+1}\Vert B\setminus A_v\Vert_\circ^{n_{5,v}-1} (1-\Vert  B \cup A_v\Vert_\circ)^{n_{6,v}}  \\
    &\leq 2 D_g(v)\chi\{\|A_v\!\setminus\! B\|_\circ \geq \|A_v\|_\circ/2\} \frac{\Vert B\setminus A_v\Vert_\circ}{\Vert A_v\setminus B\Vert_\circ} \nonumber \\
    &\quad \sum_{(n_{4,v}+1)\geq 0,(n_{5,v}-1)\geq 0, (n_{4,v}+1)+(n_{5,v}-1)\leq\ell, n_{4,v}+1\leq \ell, n_{5,v}-1\leq \ell}   \binom{l}{n_{4,v}+1~n_{5,v}-1~n_{6,v}} \nonumber \\
    &\quad \quad \quad \quad  \quad \quad \quad \quad \quad \quad \quad \quad \quad \quad \Vert A_v\setminus B\Vert_\circ^{n_{4,v}+1}\Vert B\setminus A_v\Vert_\circ^{n_{5,v}-1} (1-\Vert  B \cup A_v\Vert_\circ)^{n_{6,v}}  \\
    &= 2 D_g(v)\chi\{\|A_v\!\setminus\! B\|_\circ \geq \|A_v\|_\circ/2\} \frac{\Vert B\setminus A_v\Vert_\circ}{\Vert A_v\setminus B\Vert_\circ} \big(  
 \Vert A_v\setminus B\Vert_\circ + \Vert B\setminus A_v\Vert_\circ + (1-\Vert  B \cup A_v\Vert_\circ)\big)^\ell \\
 &= 2 \chi\{\|A_v\!\setminus\! B\|_\circ \geq \|A_v\|_\circ/2\}D_g(v) \frac{\Vert B\setminus A_v\Vert_\circ}{\Vert A_v\setminus B\Vert_\circ} \big(1-\Vert  B \cap A_v\Vert_\circ\big)^\ell \label{rrr}
\end{align}
% note: the constraint $n_{4,v}>0$ and $n_{5,v}>0$ means that for all nonzero terms, $\max(n_{4,v},n_{5,v})\leq \ell - 1$.

We argue similarly for the second term ($n_{3,v}>0$). Here we separate $\frac{n_{3,v} + n_{5,v}}{n_{4,v}+1}$ into two separate terms, one with $\frac{n_{3,v}}{n_{4,v}+1}$ and one with $\frac{n_{5,v}}{n_{4,v}+1}$, and complete the multinomial as usual.
\begin{align}
    &2  D_g(v)  \sum_{n_{3,v}+n_{4,v}+n_{5,v}+n_{6,v}=\ell} \chi \{n_{3,v}>0,\|A_v\!\setminus\! B\|_\circ \geq \|A_v\|_\circ/2\}  \binom{l}{n_{3,v}~n_{4,v}~n_{5,v}~n_{6,v}} \nonumber \\
    &\quad \quad \quad \quad  \quad \quad \quad \quad \Vert A_v\cap B\Vert_\circ^{n_{3,v}}\Vert A_v\setminus B\Vert_\circ^{n_{4,v}}\Vert B\setminus A_v\Vert_\circ^{n_{5,v}} (1-\Vert  B \cup A_v\Vert_\circ)^{n_{6,v}} \frac{n_{3,v} + n_{5,v}}{n_{4,v}+1}  \nonumber \\
    &= 2 D_g(v) \sum_{n_{3,v}+n_{4,v}+n_{5,v}+n_{6,v}=\ell} \chi \{ n_{3,v}>0,\|A_v\!\setminus\! B\|_\circ \geq \|A_v\|_\circ/2\}  \binom{l}{n_{3,v}~n_{4,v}~n_{5,v}~n_{6,v}} \nonumber \\
    &\quad \quad \quad \quad  \quad \quad \quad \quad \Vert A_v\cap B\Vert_\circ^{n_{3,v}}\Vert A_v\setminus B\Vert_\circ^{n_{4,v}}\Vert B\setminus A_v\Vert_\circ^{n_{5,v}} (1-\Vert  B \cup A_v\Vert_\circ)^{n_{6,v}} \frac{n_{3,v}}{n_{4,v}+1}  \nonumber \\
    &\quad + 2 D_g(v) \sum_{n_{3,v}+n_{4,v}+n_{5,v}+n_{6,v}=\ell} \chi \{n_{3,v}>0, \|A_v\!\setminus\! B\|_\circ \geq \|A_v\|_\circ/2\}  \binom{l}{n_{3,v}~n_{4,v}~n_{5,v}~n_{6,v}} \nonumber \\
    &\quad \quad \quad \quad  \quad \quad \quad \quad \Vert A_v\cap B\Vert_\circ^{n_{3,v}}\Vert A_v\setminus B\Vert_\circ^{n_{4,v}}\Vert B\setminus A_v\Vert_\circ^{n_{5,v}} (1-\Vert  B \cup A_v\Vert_\circ)^{n_{6,v}} \frac{n_{5,v}}{n_{4,v}+1}  \nonumber \\
    &= 2 \chi\{\|A_v\!\setminus\! B\|_\circ \geq \|A_v\|_\circ/2\} D_g(v)\frac{\Vert A_v\cap B\Vert_\circ}{\Vert A_v\setminus B\Vert_\circ} \nonumber\\
    &\quad \sum_{(n_{3,v}-1)+(n_{4,v}+1)+n_{5,v}+n_{6,v}=\ell, 0 \leq n_{3,v}-1\leq \ell-1, 1\leq n_{4,v}+1\leq \ell  }  \binom{l}{n_{3,v}-1~n_{4,v}+1~n_{5,v}~n_{6,v}} \nonumber \\
    &\quad \quad \quad \quad  \quad \quad \quad \quad \Vert A_v\cap B\Vert_\circ^{n_{3,v}-1}\Vert A_v\setminus B\Vert_\circ^{n_{4,v}+1}\Vert B\setminus A_v\Vert_\circ^{n_{5,v}} (1-\Vert  B \cup A_v\Vert_\circ)^{n_{6,v}}  \nonumber \\
    &\quad + 2 \chi\{\|A_v\!\setminus\! B\|_\circ \geq \|A_v\|_\circ/2\} D_g(v) \frac{\Vert B\setminus A_v\Vert_\circ}{\Vert A_v\setminus B\Vert_\circ} \nonumber \\
    &\quad \sum_{n_{3,v}+n_{4,v}+n_{5,v}+n_{6,v}=\ell,1 \leq n_{4,v}+1\leq \ell, 0 \leq n_{5,v}-1\leq \ell-2}  \binom{l}{n_{3,v}~n_{4,v}+1~n_{5,v}-1~n_{6,v}} \nonumber \\
    &\quad \quad \quad \quad  \quad \quad \quad \quad \Vert A_v\cap B\Vert_\circ^{n_{3,v}}\Vert A_v\setminus B\Vert_\circ^{n_{4,v}+1}\Vert B\setminus A_v\Vert_\circ^{n_{5,v}-1} (1-\Vert  B \cup A_v\Vert_\circ)^{n_{6,v}} \nonumber \\
    &\leq 2 \chi\{\|A_v\!\setminus\! B\|_\circ \geq \|A_v\|_\circ/2\} D_g(v)\frac{\Vert A_v\cap B\Vert_\circ}{\Vert A_v\setminus B\Vert_\circ} ( \Vert A_v\cap B\Vert_\circ+ \Vert A_v\setminus B\Vert_\circ+ \Vert B\setminus A_v\Vert_\circ+  1-\Vert  B \cup A_v\Vert_\circ)^\ell  \nonumber \\
    &\quad + 2 \chi\{\|A_v\!\setminus\! B\|_\circ \geq \|A_v\|_\circ/2\} D_g(v) \frac{\Vert B\setminus A_v\Vert_\circ}{\Vert A_v\setminus B\Vert_\circ} (\Vert A_v\cap B\Vert_\circ + \Vert A_v\setminus B\Vert_\circ + \Vert B\setminus A_v\Vert_\circ + 1-\Vert  B \cup A_v\Vert_\circ)^{\ell} \nonumber \\
    &= 2 \chi\{\|A_v\!\setminus\! B\|_\circ \geq \|A_v\|_\circ/2\} D_g(v)\frac{\Vert A_v\cap B\Vert_\circ+ \Vert B\setminus A_v\Vert_\circ}{\Vert A_v\setminus B\Vert_\circ}   \label{rr}
\end{align}
Note: $n_{3,v}>0$ implies $n_{4,v}+1 \leq \ell$, so we have not subtracted any terms. 
Combining \eqref{rr} and \eqref{rrr} yields
\begin{align}
     &\mathbb{E}  \left[\chi \{x \in A_v,n_{1,v} > 0,n_2 > 0,A_v\cap B\neq \emptyset,\|A_v\!\setminus\! B\|_\circ \geq \|A_v\|_\circ/2 \}  \frac{2n_2}{n_{1,v}+1} \right] \nonumber \\
    &\leq 2 \chi\{\|A_v\!\setminus\! B\|_\circ \geq \|A_v\|_\circ/2\}D_g(v)\frac{\Vert A_v\cap B\Vert_\circ+ \Vert B\setminus A_v\Vert_\circ \left(1+ \big(1-\Vert  B \cap A_v\Vert_\circ\big)^\ell\right)}{\Vert A_v\setminus B\Vert_\circ} \nonumber \\
    &= 2 \chi\{\|A_v\!\setminus\! B\|_\circ \geq \|A_v\|_\circ/2\}({\Vert A_v\cap B\Vert_\circ+ \Vert B\setminus A_v\Vert_\circ \left(1+ \big(1-\Vert  B \cap A_v\Vert_\circ\big)^\ell\right)}) \nonumber \\
    &\quad +  2 \chi\{\|A_v\!\setminus\! B\|_\circ \geq \|A_v\|_\circ/2\}\| A_v\cap B\|_\circ\frac{\Vert A_v\cap B\Vert_\circ + \Vert B\setminus A_v\Vert_\circ \left(1+ \big(1-\Vert  B \cap A_v\Vert_\circ\big)^\ell\right)}{\Vert A_v\setminus B\Vert_\circ} \nonumber \\
    &\leq 2 \chi\{\|A_v\!\setminus\! B\|_\circ \geq \|A_v\|_\circ/2\}({\Vert A_v\cap B\Vert_\circ+ \Vert B\setminus A_v\Vert_\circ \left(1+ \big(1-\Vert  B \cap A_v\Vert_\circ\big)^\ell\right)}) \nonumber \\
    &\quad +  4\| A_v\cap B\|_\circ\frac{\Vert A_v\cap B\Vert_\circ + \Vert B\setminus A_v\Vert_\circ \left(1+ \big(1-\Vert  B \cap A_v\Vert_\circ\big)^\ell\right)}{\Vert A_v\Vert_\circ}
\end{align}
which scales as $O(\|B\|_\circ)$, as desired.
We follow the same procedure for term 2 in \eqref{onehalf}:
\begin{align}
   & \mathbb{E}  \left[\chi \{x \in A_v,n_{1,v} > 0,n_2 > 0,A_v\cap B\neq \emptyset, \|A_v\cap B\|_\circ > \|A_v\|_\circ/2 \}  \frac{2n_2}{n_{1,v}+1} \right]  \nonumber \\
    &= D_g(v) \nonumber \\
    &\quad \sum_{n_{3,v}+n_{4,v}+n_{5,v}+n_{6,v}=\ell} \chi \{n_{3,v} +n_{4,v}> 0,n_{3,v} +n_{5,v}> 0, \|A_v\!\cap\! B\|_\circ \geq \|A_v\|_\circ/2  \}  \binom{l}{n_{3,v}~n_{4,v}~n_{5,v}~n_{6,v}} \nonumber \\
    &\quad \quad \quad \quad  \quad \quad \quad \quad \Vert A_v\cap B\Vert_\circ^{n_{3,v}}\Vert A_v\setminus B\Vert_\circ^{n_{4,v}}\Vert B\setminus A_v\Vert_\circ^{n_{5,v}} (1-\Vert  B \cup A_v\Vert_\circ)^{n_{6,v}} \frac{2(n_{3,v} + n_{5,v})}{n_{3,v} + n_{4,v}+1} \\
    &\leq  2 D_g(v)\nonumber \\
    &\quad \sum_{n_{3,v}+n_{4,v}+n_{5,v}+n_{6,v}=\ell} \chi \{n_{3,v} +n_{4,v}> 0,n_{3,v} +n_{5,v}> 0, \|A_v\!\cap\! B\|_\circ \geq \|A_v\|_\circ/2\}  \binom{l}{n_{3,v}~n_{4,v}~n_{5,v}~n_{6,v}} \nonumber \\
    &\quad \quad \quad \quad  \quad \quad \quad \quad \Vert A_v\cap B\Vert_\circ^{n_{3,v}}\Vert A_v\setminus B\Vert_\circ^{n_{4,v}}\Vert B\setminus A_v\Vert_\circ^{n_{5,v}} (1-\Vert  B \cup A_v\Vert_\circ)^{n_{6,v}} \frac{n_{3,v} + n_{5,v}}{n_{3,v}+1} \\
    &= 2 D_g(v) \sum_{n_{3,v}+n_{4,v}+n_{5,v}+n_{6,v}=\ell} \chi \{n_{3,v}=0, n_{4,v}> 0, n_{5,v}> 0, \|A_v\!\cap\! B\|_\circ \geq \|A_v\|_\circ/2\}  \binom{l}{0~n_{4,v}~n_{5,v}~n_{6,v}} \nonumber \\
    &\quad \quad \quad \quad  \quad \quad \quad \quad \Vert A_v\setminus B\Vert_\circ^{n_{4,v}}\Vert B\setminus A_v\Vert_\circ^{n_{5,v}} (1-\Vert  B \cup A_v\Vert_\circ)^{n_{6,v}} {n_{5,v}} \\
    &\quad + 2 D_g(v) \sum_{n_{3,v}+n_{4,v}+n_{5,v}+n_{6,v}=\ell} \chi \{n_{3,v}>0,\|A_v\!\cap\! B\|_\circ \geq \|A_v\|_\circ/2\}  \binom{l}{n_{3,v}~n_{4,v}~n_{5,v}~n_{6,v}} \nonumber \\
    &\quad \quad \quad \quad  \quad \quad \quad \quad \Vert A_v\cap B\Vert_\circ^{n_{3,v}}\Vert A_v\setminus B\Vert_\circ^{n_{4,v}}\Vert B\setminus A_v\Vert_\circ^{n_{5,v}} (1-\Vert  B \cup A_v\Vert_\circ)^{n_{6,v}} \frac{n_{3,v} + n_{5,v}}{n_{3,v}+1} \label{32}
\end{align}
For the first term in \eqref{32},
\begin{align}
    & 2 D_g(v) \sum_{n_{3,v}+n_{4,v}+n_{5,v}+n_{6,v}=\ell} \chi \{n_{3,v}=0, n_{4,v}> 0, n_{5,v}> 0, \|A_v\!\cap\! B\|_\circ \geq \|A_v\|_\circ/2\}  \binom{l}{0~n_{4,v}~n_{5,v}~n_{6,v}} \nonumber \\
    &\quad \quad \quad \quad  \quad \quad \quad \quad \Vert A_v\setminus B\Vert_\circ^{n_{4,v}}\Vert B\setminus A_v\Vert_\circ^{n_{5,v}} (1-\Vert  B \cup A_v\Vert_\circ)^{n_{6,v}} {n_{5,v}} \nonumber \\
    &= 2 D_g(v)\frac{\Vert B\setminus A_v\Vert_\circ}{1-\Vert  B \cup A_v\Vert_\circ} \nonumber \\
    &\quad \sum_{n_{4,v}+n_{5,v}\leq \ell} \chi \{ n_{4,v}> 0, n_{5,v}> 0, \|A_v\!\cap\! B\|_\circ \geq \|A_v\|_\circ/2\}  \binom{l}{n_{4,v}~n_{5,v}\!-\!1~(\ell- n_{4,v}-n_{5,v})} \nonumber \\
    &\quad \quad \quad \quad  \quad \quad \quad \quad \Vert A_v\setminus B\Vert_\circ^{n_{4,v}}\Vert B\setminus A_v\Vert_\circ^{n_{5,v}-1} (1-\Vert  B \cup A_v\Vert_\circ)^{\ell - n_{4,v} -(n_{5,v}-1)} \nonumber \\
    &= 2 D_g(v)\frac{\Vert B\setminus A_v\Vert_\circ}{1-\Vert  B \cup A_v\Vert_\circ} \nonumber \\
    &\quad \sum_{n_{4,v}+n_{5,v}\leq \ell, 1\leq n_{5,v}\leq \ell-1 } \chi \{ n_{4,v}> 0, n_{5,v}> 0, \|A_v\!\cap\! B\|_\circ \geq \|A_v\|_\circ/2\}  \binom{l}{n_{4,v}~n_{5,v}\!-\!1~(\ell- n_{4,v}-n_{5,v})} \nonumber \\
    &\quad \quad \quad \quad  \quad \quad \quad \quad \Vert A_v\setminus B\Vert_\circ^{n_{4,v}}\Vert B\setminus A_v\Vert_\circ^{n_{5,v}-1} (1-\Vert  B \cup A_v\Vert_\circ)^{\ell - n_{4,v} -(n_{5,v}-1)} \nonumber \\
    &\leq 2 \ell D_g(v)\frac{\Vert B\setminus A_v\Vert_\circ}{1-\Vert  B \cup A_v\Vert_\circ} \sum_{n_{4,v}+(n_{5,v}-1)\leq \ell} \chi \{  \|A_v\!\cap\! B\|_\circ \geq \|A_v\|_\circ/2\}  \binom{l}{n_{4,v}~n_{5,v}\!-\!1~(\ell- n_{4,v}-(n_{5,v}-1))} \nonumber \\
    &\quad \quad \quad \quad  \quad \quad \quad \quad \Vert A_v\setminus B\Vert_\circ^{n_{4,v}}\Vert B\setminus A_v\Vert_\circ^{n_{5,v}-1} (1-\Vert  B \cup A_v\Vert_\circ)^{\ell - n_{4,v} -(n_{5,v}-1)} \nonumber \\
    &= 2 \ell D_g(v)\frac{\Vert B\setminus A_v\Vert_\circ}{1-\Vert  B \cup A_v\Vert_\circ} \chi \{ \|A_v\!\cap\! B\|_\circ \geq \|A_v\|_\circ/2\}  ( \Vert A_v\setminus B\Vert_\circ+\Vert B\setminus A_v\Vert_\circ + 1-\Vert  B \cup A_v\Vert_\circ)^{\ell} \nonumber \\
 &= 2 \ell D_g(v)\frac{\Vert B\setminus A_v\Vert_\circ}{1-\Vert  B \cup A_v\Vert_\circ} \chi \{ \|A_v\!\cap\! B\|_\circ \geq \|A_v\|_\circ/2\}  ( 1-\Vert  B \cap A_v\Vert_\circ)^{\ell} \nonumber \\
 &\leq 2 \ell \Vert  A_v\Vert_\circ\frac{\Vert B\setminus A_v\Vert_\circ}{1-\Vert  B \cup A_v\Vert_\circ}   (1 - \Vert  A_v\Vert_\circ/2)^{\ell} \chi \{ \|A_v\!\cap\! B\|_\circ \geq \|A_v\|_\circ/2\}
\end{align}
Note: $\Vert  B \cup A_v\Vert_\circ$ is 1 only if $g$ is clean. so $\Vert  B \cup A_v\Vert_\circ < 1$. We will further upper bound $\Vert  B \cup A_v\Vert_\circ \leq 1/2$ by choice of $g'$.
% Also the sum for $n_{5,v}-1$ only adds (two) positive terms, so the upper bound with with the compressed polynomial is kosher.
Next for the second term in \eqref{32}. We split it into two terms, one with $n_{3,v}$ the other with $n_{5,v}$. For the $n_{3,v}$ term we have:
\begin{align}
    &2 D_g(v) \sum_{n_{3,v}+n_{4,v}+n_{5,v}+n_{6,v}=\ell} \chi \{n_{3,v}>0,\|A_v\!\cap\! B\|_\circ \geq \|A_v\|_\circ/2\}  \binom{l}{n_{3,v}~n_{4,v}~n_{5,v}~n_{6,v}} \nonumber \\
    &\quad \quad \quad \quad  \quad \quad \quad \quad \Vert A_v\cap B\Vert_\circ^{n_{3,v}}\Vert A_v\setminus B\Vert_\circ^{n_{4,v}}\Vert B\setminus A_v\Vert_\circ^{n_{5,v}} (1-\Vert  B \cup A_v\Vert_\circ)^{n_{6,v}} \frac{n_{3,v}}{n_{3,v}+1} \nonumber \\
    &\leq 2 \|A_v\|_\circ \chi \{\|A_v\!\cap\! B\|_\circ \geq \|A_v\|_\circ/2\}  \sum_{n_{3,v}+n_{4,v}+n_{5,v}+n_{6,v}=\ell}  \binom{l}{n_{3,v}~n_{4,v}~n_{5,v}~n_{6,v}} \nonumber \\
    &\quad \quad \quad \quad  \quad \quad \quad \quad \Vert A_v\cap B\Vert_\circ^{n_{3,v}}\Vert A_v\setminus B\Vert_\circ^{n_{4,v}}\Vert B\setminus A_v\Vert_\circ^{n_{5,v}} (1-\Vert  B \cup A_v\Vert_\circ)^{n_{6,v}} \nonumber \\
    &\leq 2 \|A_v\|_\circ \chi \{\|A_v\!\cap\! B\|_\circ \geq \|A_v\|_\circ/2\}  \nonumber 
\end{align}
which is small enough because  $\|A_v\|_\circ = O(\|B\|_\circ)$ whenever the indicator is 1.

For the $n_{5,v}$ term, note that its summand is zero whenever $n_{5,v}$ is zero. So we only need to consider nonzero $n_{5,v}>0$.  We have:
\begin{align}
    &2 D_g(v) \sum_{n_{3,v}+n_{4,v}+n_{5,v}+n_{6,v}=\ell} \chi \{n_{3,v}>0,\|A_v\!\cap\! B\|_\circ \geq \|A_v\|_\circ/2\}  \binom{l}{n_{3,v}~n_{4,v}~n_{5,v}~n_{6,v}} \nonumber \\
    &\quad \quad \quad \quad  \quad \quad \quad \quad \Vert A_v\cap B\Vert_\circ^{n_{3,v}}\Vert A_v\setminus B\Vert_\circ^{n_{4,v}}\Vert B\setminus A_v\Vert_\circ^{n_{5,v}} (1-\Vert  B \cup A_v\Vert_\circ)^{n_{6,v}} \frac{n_{5,v}}{n_{3,v}+1} \nonumber \\
    &= 2 \|A_v\|_\circ\frac{\Vert B\setminus A_v\Vert_\circ}{\Vert A_v\cap B\Vert_\circ} \sum_{(n_{3,v}+1)+n_{4,v}+(n_{5,v}-1)+n_{6,v}=\ell} \chi \{n_{3,v}>0,n_{5,v}>0,\|A_v\!\cap\! B\|_\circ \geq \|A_v\|_\circ/2\} \nonumber \\
    &\quad \quad \quad \quad  \binom{l}{n_{3,v}+1~n_{4,v}~n_{5,v}-1~n_{6,v}}  \Vert A_v\cap B\Vert_\circ^{n_{3,v}+1}\Vert A_v\setminus B\Vert_\circ^{n_{4,v}}\Vert B\setminus A_v\Vert_\circ^{n_{5,v}-1} (1-\Vert  B \cup A_v\Vert_\circ)^{n_{6,v}} \nonumber \\
    &\leq 2 \|A_v\|_\circ\frac{\Vert B\setminus A_v\Vert_\circ}{\Vert A_v\cap B\Vert_\circ}\chi \{\|A_v\!\cap\! B\|_\circ \geq \|A_v\|_\circ/2\}   \nonumber 
\end{align}
% note that $n_{5,v}>0$ implies that $n_{3,v}<\ell$, so we aren't subtracting a term (the $n_{3,v}+1=\ell+1$ term)  when compressing the polynomial.
Combining all terms, we can finally upper bound \eqref{onehalf}:
\begin{align}
    &\mathbb{E}  \left[\chi \{x \in A_v,n_{1,v} > 0,n_2 > 0,A_v\cap B\neq \emptyset \}  \frac{2n_2}{n_{1,v}+1} \right] \nonumber \\
    &\leq  2 \chi\{\|A_v\!\setminus\! B\|_\circ \geq \|A_v\|_\circ/2\}({\Vert A_v\cap B\Vert_\circ+ \Vert B\setminus A_v\Vert_\circ \left(1+ \big(1-\Vert  B \cap A_v\Vert_\circ\big)^\ell\right)}) \nonumber \\
    &\quad +  2 \chi\{\|A_v\!\setminus\! B\|_\circ \geq \|A_v\|_\circ/2\}\| A_v\cap B\|_\circ\frac{\Vert A_v\cap B\Vert_\circ + \Vert B\setminus A_v\Vert_\circ \left(1+ \big(1-\Vert  B \cap A_v\Vert_\circ\big)^\ell\right)}{\Vert A_v\setminus B\Vert_\circ} \nonumber \\
    &\quad + 2 \ell \Vert  A_v\Vert_\circ\frac{\Vert B\setminus A_v\Vert_\circ}{1-\Vert  B \cup A_v\Vert_\circ}   (1 - \Vert  A_v\Vert_\circ/2)^{\ell} \chi \{ \|A_v\!\cap\! B\|_\circ \geq \|A_v\|_\circ/2\} \nonumber \\
    &\quad +2 \|A_v\|_\circ \left(\frac{\Vert B\setminus A_v\Vert_\circ}{\Vert A_v\cap B\Vert_\circ}+1\right)\chi \{\|A_v\!\cap\! B\|_\circ \geq \|A_v\|_\circ/2\} 
    \end{align}
The first two lines are from $\{\|A_v\!\setminus\! B\|_\circ \geq \|A_v\|_\circ/2\}$, the others are 
from $\{\|A_v\!\cap\! B\|_\circ \geq \|A_v\|_\circ/2\} $, when $n_{3,v}=0$ (third line) and when it is nonzero. We can further upper bound:
\begin{align}
     &\mathbb{E}  \left[\chi \{x \in A_v,n_{1,v} > 0,n_2 > 0,A_v\cap B\neq \emptyset \}  \frac{2n_2}{n_{1,v}+1} \right] \nonumber \\
    &\leq 2 \chi\{\|A_v\!\setminus\! B\|_\circ \geq \|A_v\|_\circ/2\}({\Vert A_v\cap B\Vert_\circ+ 2\Vert B\setminus A_v\Vert_\circ }) \nonumber \\
    &\quad +  4 \chi\{\|A_v\!\setminus\! B\|_\circ \geq \|A_v\|_\circ/2\}\frac{\Vert A_v\cap B\Vert_\circ^2 + 2 \Vert A_v\cap B\Vert_\circ\Vert B\setminus A_v\Vert_\circ}{\Vert A_v\Vert_\circ} \nonumber \\
    &\quad + 4 \ell \Vert  A_v\cap B\Vert_\circ\frac{\Vert B\setminus A_v\Vert_\circ}{1-\Vert  B \cup A_v\Vert_\circ}   (1 - \Vert  A_v\Vert_\circ/2)^{\ell} \chi \{ \|A_v\!\cap\! B\|_\circ \geq \|A_v\|_\circ/2\} \nonumber \\
    &\quad +4 \|A_v\cap B\|_\circ \left(2\frac{\Vert B\setminus A_v\Vert_\circ}{\Vert A_v\Vert_\circ}+1\right)\chi \{\|A_v\!\cap\! B\|_\circ \geq \|A_v\|_\circ/2\} 
\end{align}
Note that all terms besides the third are $O(\|B\|_\circ)$ as desired.

% Concerns: do we have lower bound on $\|A_v\|_{\circ}$ when $A_v\cap B\neq \emptyset$? we don't need it.
% Do we have upper bound on $\Vert  B \cup A_v\Vert_\circ$?

Note that we can choose $g'$ such that $\|A_v\cup B\|\leq 1/2$ for all $v$.
% (which may require choosing the larger of two options for $B$). 
Argument: there are two options for $g'$. Each induces  $B,B'$, respectively. Let  $A_v,A_v'$ be the largest inverse sets that intersect with $B,\tilde{B}$, respectively. The sets $A_v \cup B$ and $\tilde{A}_v\cup \tilde{B}$ are disjoint. So $\|A_v \cup B\|_\circ + \| \tilde{A}_v\cup \tilde{B}\|_\circ \leq 1 \implies \min(\|A_v \cup B\|_\circ, \| \tilde{A}_v\cup \tilde{B}\|_\circ) \leq 1/2.$ It is easy to see that we can choose a $g'$ such that $\|A_v \cup B\|_\circ \leq 1/2$ for all $v$. Just choose $g'$ such that it is the opposite of the $g'$ that yields $\max_v  \|A_v \cup B\|_\circ$.
Thus we can further upper bound, using particular choice of $g'$ ($f_1'$),
\begin{align}
     &\mathbb{E}  \left[\chi \{x \in A_v,n_{1,v} > 0,n_2 > 0,A_v\cap B\neq \emptyset \}  \frac{2n_2}{n_{1,v}+1} \right] \nonumber \\
    &\leq 2 \chi\{\|A_v\!\setminus\! B\|_\circ \geq \|A_v\|_\circ/2\}({\Vert A_v\cap B\Vert_\circ+ 2\Vert B\setminus A_v\Vert_\circ }) \nonumber \\
    &\quad +  4 \chi\{\|A_v\!\setminus\! B\|_\circ \geq \|A_v\|_\circ/2\}\frac{\Vert A_v\cap B\Vert_\circ^2 + 2 \Vert A_v\cap B\Vert_\circ\Vert B\setminus A_v\Vert_\circ}{\Vert A_v\Vert_\circ} \nonumber \\
    &\quad + 8 \ell \Vert  A_v\cap B\Vert_\circ {\Vert B\setminus A_v\Vert_\circ}  (1 - \Vert  A_v\Vert_\circ/2)^{\ell} \chi \{ \|A_v\!\cap\! B\|_\circ \geq \|A_v\|_\circ/2\} \nonumber \\
    &\quad +4 \|A_v\cap B\|_\circ \left(2\frac{\Vert B\setminus A_v\Vert_\circ}{\Vert A_v\Vert_\circ}+1\right)\chi \{\|A_v\!\cap\! B\|_\circ \geq \|A_v\|_\circ/2\} 
\end{align}
Now we need to consider the last two terms in \eqref{4terms}, which correspond to the case wherein the positive inner products are not equal for $g$ and $g'$. For the third term, we simply have
{\begin{align}
&\mathbb{E}  \left[\chi \{x \in A_v,n_{1,v} > 0,n_2 > 0,  g'(x)^\top g'(x^+) \neq  g(x)^\top g(x^+), A_v\cap B= \emptyset \}  \frac{  2  }{n_{1,v}+1 } \right]\nonumber \\
  &\leq \chi\{A_v\cap B= \emptyset \} \mathbb{P}  \left[x \in A_v, x^+\in B\right]
\end{align}
}

For the fourth term in \eqref{4terms}, we have {
\begin{align}
&\mathbb{E}  \left[\chi \{x \in A_v,n_{1,v} > 0,n_2 > 0,  g'(x)^\top g'(x^+) \neq  g(x)^\top g(x^+), A_v\cap B\neq \emptyset \}  \frac{  2  }{n_{1,v}+1 } \right] \nonumber \\
&\leq \chi\{A_v\cap B\neq \emptyset \} \mathbb{P}  \left[x \in A_v \cap B, x^+ \notin B \right] 
\end{align}
}
In total, for the case $n_{1,v}>0,n_2>0$, we have
\begin{align}
    &\mathbb{E}  \left[\chi \{x \in A_v,n_{1,v} > 0,n_2 > 0\}  \log\bigg({ e^{\beta g'(x)^\top g'(x^+)}+ n_{1,v}e^{\beta d} + \sum_{x_i^{-} \in B}e^{\beta g'(x)^\top g'(x^-_{i})}  +\sum_{x_i^{-}\not\in {A}_v\cup B} e^{\beta g(x)^\top g(x^-_{i})}  } \bigg) \right]\nonumber \\
    &\quad - \mathbb{E} \bigg[\chi \{x \in A_v,n_{1,v} > 0,n_2 > 0\}  \nonumber \\
    &\quad \quad \quad \quad \log\bigg({ e^{\beta g(x)^\top g(x^+)}+n_{1,v}e^{\beta d}
+ \sum_{x_i^{-} \in B}e^{\beta g(x)^\top g(x^-_{i})}  +\sum_{x_i^{-}\not\in {A}_v\cup B} e^{\beta g(x)^\top g(x^-_{i})}  } \bigg) \bigg] \nonumber \\
&\leq 2 \|B\|_\circ \chi\{ A_v\cap B = \emptyset \} + 2 \chi\{\|A_v\!\setminus\! B\|_\circ \geq \|A_v\|_\circ/2\}({\Vert A_v\cap B\Vert_\circ+ 2\Vert B\setminus A_v\Vert_\circ }) \nonumber \\
    &\quad +  4 \chi\{\|A_v\!\setminus\! B\|_\circ \geq \|A_v\|_\circ/2\}\frac{\Vert A_v\cap B\Vert_\circ^2 + 2 \Vert A_v\cap B\Vert_\circ\Vert B\setminus A_v\Vert_\circ}{\Vert A_v\Vert_\circ} \nonumber \\
    &\quad + 8 \ell \Vert  A_v\cap B\Vert_\circ {\Vert B\setminus A_v\Vert_\circ}  (1 - \Vert  A_v\Vert_\circ/2)^{\ell} \chi \{ \|A_v\!\cap\! B\|_\circ \geq \|A_v\|_\circ/2\} \nonumber \\
    &\quad +4 \|A_v\cap B\|_\circ \left(2\frac{\Vert B\setminus A_v\Vert_\circ}{\Vert A_v\Vert_\circ}+1\right)\chi \{\|A_v\!\cap\! B\|_\circ \geq \|A_v\|_\circ/2\} \nonumber \\
    &\quad + \chi\{A_v\cap B= \emptyset \} \mathbb{P}  \left[x \in A_v, x^+\in B\right] + \chi\{A_v\cap B\neq \emptyset \} \mathbb{P}  \left[x \in A_v \cap B, x^+ \notin B \right] 
\end{align}
All of these terms are $O(\|B\|_\circ)$ and do not depend on $\beta$ so we can make $\beta$ large enough to dominate them.

% Aside: if $x\in A_v\setminus B$ and $A_v \cap B \neq \emptyset$ then the negative loss should not get worse going to $g'$ (easy to see with picture, note that if the intersection is nonzero then the remainder of $A_v$ has to be to the right of $g'$). We haven't used this, but maybe it doesn't matter.

% We have considered all the cases.

Combining all three cases and summing over $v\in \mathcal{H}_d$ yields 
\begin{align*}
\mathcal{L}_{\text{neg}}(g') -\mathcal{L}_{\text{neg}}(g)
&\le \sum_{v \in \mathcal{H}_d}  \mathbb{P}(x \in A_v,x^+ \in B) \bigg( 2 \beta \|A_v\|_\circ(1 - \|A_v\|_\circ - \|B\|_\circ)^\ell + \log(2) \|A_v\|_\circ\bigg) \nonumber \\
&\quad + 2 \beta \ell \log(\ell+1) \|A_v\|_\circ (1 - \|A_v\|_\circ)^\ell  \mathbb{P} ( x_{1}^- \in B |  x_{1}^- \notin A_v) \nonumber \\
&\quad + 2 \|B\|_\circ \chi\{ A_v\cap B = \emptyset \} + 2 \chi\{\|A_v\!\setminus\! B\|_\circ \geq \|A_v\|_\circ/2\}({\Vert A_v\cap B\Vert_\circ+ 2\Vert B\setminus A_v\Vert_\circ }) \nonumber \\
    &\quad +  4 \chi\{\|A_v\!\setminus\! B\|_\circ \geq \|A_v\|_\circ/2\}\frac{\Vert A_v\cap B\Vert_\circ^2 + 2 \Vert A_v\cap B\Vert_\circ\Vert B\setminus A_v\Vert_\circ}{\Vert A_v\Vert_\circ} \nonumber \\
    &\quad + 8 \ell \Vert  A_v\cap B\Vert_\circ {\Vert B\setminus A_v\Vert_\circ}  (1 - \Vert  A_v\Vert_\circ/2)^{\ell} \chi \{ \|A_v\!\cap\! B\|_\circ \geq \|A_v\|_\circ/2\} \nonumber \\
    &\quad +4 \|A_v\cap B\|_\circ \left(2\frac{\Vert B\setminus A_v\Vert_\circ}{\Vert A_v\Vert_\circ}+1\right)\chi \{\|A_v\!\cap\! B\|_\circ \geq \|A_v\|_\circ/2\} \nonumber \\
    &\quad + \chi\{A_v\cap B= \emptyset \} \mathbb{P}  \left[x \in A_v, x^+\in B\right] + \chi\{A_v\cap B\neq \emptyset \} \mathbb{P}  \left[x \in A_v \cap B, x^+ \notin B \right] \nonumber \\
    &\leq  \sum_{v \in \mathcal{H}_d}  \|A_v \cap B\|_\circ \|A_v\|_\circ\bigg( 2 \beta (1 - \|A_v\|_\circ - \|B\|_\circ)^\ell + \log(2) \bigg) \nonumber \\
&\quad + 2 \beta \ell \log(\ell+1)  \sum_{v \in \mathcal{H}_d} \|A_v\|_\circ (1 - \|A_v\|_\circ)^\ell  \mathbb{P} ( x_{1}^- \in B |  x_{1}^- \notin A_v) \nonumber \\
    &\quad + (2*2^{d} + 4*2^{d} + 4*2*2^d) \|B\|_\circ\nonumber \\
    &\quad + 8\ell \sum_{v \in \mathcal{H}_d} \Vert  A_v\cap B\Vert_\circ {\Vert B\setminus A_v\Vert_\circ}  (1 - \Vert  A_v\Vert_\circ/2)^{\ell} \chi\{\|A_v\!\cap\! B\|_\circ \geq \|A_v\|_\circ/2 \} \nonumber \\
    &\quad + 8 \sum_{v \in \mathcal{H}_d} \Vert B\setminus A_v\Vert_\circ \chi \{\|A_v\!\cap\! B\|_\circ \geq \|A_v\|_\circ/2\} \nonumber \\
    &\quad + 4 \sum_{v \in \mathcal{H}_d} \Vert  A_v \cap B\Vert_\circ \chi \{\|A_v\!\cap\! B\|_\circ \geq \|A_v\|_\circ/2\} \nonumber \\
    &\quad \sum_{v\in \mathcal{H}_d} \chi\{A_v\cap B= \emptyset \} \mathbb{P}  \left[x \in A_v, x^+\in B\right] + \chi\{A_v\cap B\neq \emptyset \} \mathbb{P}  \left[x \in A_v \cap B, x^+ \notin B \right] \nonumber \\
    &\leq 27*2^d \|B\|_\circ  + 2 \beta (\ell \log(\ell+1) +1) \|B\|_\circ  \sum_{v \in \mathcal{H}_d} \|A_v\|_\circ (1 - \|A_v\|_\circ)^\ell  \nonumber \\
    &\quad + 8\ell \|B\|_\circ \sum_{v \in \mathcal{H}_d} \Vert  A_v\Vert_\circ   (1 - \Vert  A_v\Vert_\circ/2)^{\ell}  \nonumber \\
    &\quad \underbrace{\sum_{v\in \mathcal{H}_d} \chi\{A_v\cap B= \emptyset \} \mathbb{P}  \left[x \in A_v, x^+\in B\right] + \chi\{A_v\cap B\neq \emptyset \} \mathbb{P}  \left[x \in A_v \cap B, x^+ \notin B \right]}_{\text{area of shaded region}} \nonumber %\\
    % &\leq 
    % \sum_{v \in \mathcal{H}_d}\chi\{\Vert B\setminus A_v\Vert_\circ \}
    % &\leq 27*2^d \|B\|_\circ  + 2 \beta (\ell \log(\ell+1) +1)  e^{-\ell 2^{-d} } \|B\|_\circ   + 8\ell  e^{-\ell 2^{-d-1} }  \|B\|_\circ \nonumber \\
    % &\quad \underbrace{\sum_{v\in \mathcal{H}_d} \chi\{A_v\cap B= \emptyset \} \mathbb{P}  \left[x \in A_v, x^+\in B\right] + \chi\{A_v\cap B\neq \emptyset \} \mathbb{P}  \left[x \in A_v \cap B, x^+ \notin B \right]}_{\text{area of shaded region}} \nonumber \\
\end{align*}

% If all $\|A_v\|_\circ \geq c 2^{-d}$ then:

We are done if we set  $\beta = \Omega(2^d)$, $\ell = \Omega(d 2^d)$, and upper bound $\|B_\circ\|$ in terms of shaded region.

Note that we cannot do the latter by some property of the closest $g'$ to $g$, since we have used a $g'$ that is not necessarily closest to $g$. Let $R$ be the shaded region.
Suppose that 
$\|B\|_\circ \leq \eta \|R\| $ for some $\eta>0$\footnote{Need to formalize this assumption}. Then if $\|A_v\|_\circ = 2^{-d}$ for all $v$, the upper bound on the difference of negative terms is
\begin{align}
  \mathcal{L}_{\text{neg}}(g') -\mathcal{L}_{\text{neg}}(g)
&\le   (27\eta*2^d+1) \|R\|  + 2 \beta \eta (\ell \log(\ell+1) +1)  e^{-\ell 2^{-d} } \|R\|   + 4\eta \ell  e^{-\ell 2^{-d-1} }  \|R\| \nonumber 
\end{align}
 Let $\ell = C d 2^d$ and $\beta = 4*28*\eta * 2^d$. Then 
 \begin{align}
  \mathcal{L}_{\text{neg}}(g') -\mathcal{L}_{\text{neg}}(g)
&\le  (27\eta*2^d+1) \|R\|   + 4\eta  \beta Cd^2  \log(Cd)  e^{-(C-1)d } \|R\|   + 4\eta Cd 2^d  e^{-Cd/2 }  \|R\| \nonumber \\
&\leq \beta \|R\| \left( \frac{1}{2}  + 4\eta   Cd^2  \log(Cd)  e^{-(C-1)d }    + \frac{\eta}{28} Cd  e^{-Cd/2 } \right) \nonumber \\
&\stackrel{*}{\leq} \beta \|R\|  \nonumber
\end{align}
where $*$ holds iff
\begin{align}
    &4\eta   Cd^2  \log(Cd)  e^{-(C-1)d }    + \frac{\eta}{28} Cd  e^{-Cd/2 }\leq 1/2 \nonumber
\end{align}
The worst case is $d=1$. Then
\begin{align}
    &4\eta   C  \log(C)  e^{-(C-1) }    + \frac{\eta}{28} C e^{-C/2 }\leq 1/2 \nonumber \\ 
\end{align}
One can check that $C\geq 6\log(\eta)$ is sufficient. 

Recall that for the positive gain we have $\mathcal{L}_{\text{pos}}(g') -\mathcal{L}_{\text{pos}}(g)\leq -2\beta \|R\|$, completing the proof.

{\color{blue}
The key is upper bounding $\sum_{v \in \mathcal{H}_d} \|A_v\|_\circ (1 - \|A_v\|_\circ)^\ell $.
The largest term scales as $\beta \ell \log(\ell)\sum_{v \in \mathcal{H}_d} \|A_v\|_\circ (1 - \|A_v\|_\circ)^\ell $, corresponding to the case $n_{1,v}=0$ and $n_2>0$.
As long as $\|A_v\|_\circ > \frac{\log(d)}{cd2^d}$ or $\|A_v\|_\circ \leq \frac{\log(d)}{C d^2 2^{2d}}$ for all $v\in \mathcal{H}_d$,\footnote{Corresponding to the cases that $A_v$ is large enough such that there are likely other $e^{\beta d}$ terms in the log to offset terms that may go from $e^{\beta(d-2)}$ to $e^{\beta d}$ for $x_{i}^-$, or $A_v$ is small enough such that it is highly unlikely that $x \in A_v$.} then $\sum_{v \in \mathcal{H}_d} \|A_v\|_\circ (1 - \|A_v\|_\circ)^\ell $ is sufficiently small, for some numerical constants $C,c$. Otherwise, there exists a scenario in which both of the two possible $f_1'$ adjacent to $f_1$ result in $g'$ that has larger loss than $g$. In this case the representation can be improved, but not by substituting one of two adjacent cleaner classifiers. The challenge is formalizing which $g'$ one should pick in all cases...

Alternatively, we can choose $\beta_2 = o(1)$ and $\beta_2 = \Omega(4^d)$ to show that the positive difference is larger than the negative difference. 
But this is not aligned with practice...
}

% Overall, for case $\circled{1}$, this gives a total 
% \begin{align*}
% 0\cdot\Pr[\circled{1a}]+2\beta \Pr[\circled{1b}] + \frac{\Vert B\Vert_\circ}{\Vert A\Vert_\circ} \Pr[\circled{1c}]=2\beta \sum_{i\in \uH^d} D_g(i)\left(1-D_g(i)\right)^ll\delta + 2\frac{\Vert B\Vert_\circ}{\Vert A\Vert_\circ}
% \end{align*}

\end{enumerate}

\end{proof}

For the second term in \eqref{4terms}, let $n_{3,v} := \sum_i \chi\{x_i^- \in A_v \cap B\}$, $n_{4,v} := \sum_i \chi\{x_i^- \in A_v \setminus B\}$, $n_{5,v} := \sum_i \chi\{x_i^- \in B \setminus A_v\}$ and let $n_{6,v} = 1 - n_{3,v}+n_{4,v}+n_{5,v}$. Note $n_{1,v} = n_{3,v} + n_{4,v}$, $n_2 = n_{3,v} + n_{5,v}$. 

Observe that at least one of  $\|A_v \cap B\|_\circ$, $\|A_v \setminus B\|_\circ$ has measure at least $1/2 \|A_v\|_\circ$. In particular $\{\|A_v \cap B\|_\circ > \|A_v \|_\circ /2\} \cap \{\|A_v \setminus B\|_\circ\geq \|A_v\|_\circ /2\} = \emptyset$ and $\{\|A_v \cap B\|_\circ > \|A_v \|_\circ /2\} \cup \{\|A_v \setminus B\|_\circ\geq \|A_v\|_\circ /2\} = U=$ Universal set. So we have
\begin{align}
    &\mathbb{E}  \left[\chi \{x \in A_v,n_{1,v} > 0,n_2 > 0,A_v\cap B\neq \emptyset \}  \frac{2n_2}{n_{1,v}+1} \right] \nonumber \\
    &=\mathbb{E}  \left[\chi \{x \in A_v,n_{1,v} > 0,n_2 > 0,A_v\cap B\neq \emptyset, \|A_v\setminus B\|_\circ \geq \|A_v\|_\circ/2 \}  \frac{2n_2}{n_{1,v}+1} \right] \nonumber \\
    &\quad + \mathbb{E}  \left[\chi \{x \in A_v,n_{1,v} > 0,n_2 > 0,A_v\cap B\neq \emptyset, \|A_v\cap B\|_\circ > \|A_v\|_\circ/2 \}  \frac{2n_2}{n_{1,v}+1} \right]  \label{onehalf}
    \end{align}

    For term 1 in \eqref{onehalf} we have
    \begin{align}
    &\mathbb{E}  \left[\chi \{x \in A_v,n_{1,v} > 0,n_2 > 0,A_v\cap B\neq \emptyset, \|A_v\setminus B\|_\circ \geq \|A_v\|_\circ/2 \}  \frac{2n_2}{n_{1,v}+1} \right] \nonumber \\
    &= D_g(v) \nonumber \\
    &\quad \sum_{n_{3,v}+n_{4,v}+n_{5,v}+n_{6,v}=\ell} \chi \{n_{3,v} +n_{4,v}> 0,n_{3,v} +n_{5,v}> 0, \|A_v\!\setminus\! B\|_\circ \geq \|A_v\|_\circ/2  \}  \binom{l}{n_{3,v}~n_{4,v}~n_{5,v}~n_{6,v}} \nonumber \\
    &\quad \quad \quad \quad  \quad \quad \quad \quad \Vert A_v\cap B\Vert_\circ^{n_{3,v}}\Vert A_v\setminus B\Vert_\circ^{n_{4,v}}\Vert B\setminus A_v\Vert_\circ^{n_{5,v}} (1-\Vert  B \cup A_v\Vert_\circ)^{n_{6,v}} \frac{2(n_{3,v} + n_{5,v})}{n_{3,v} + n_{4,v}+1} \nonumber \\
    &\leq  2 D_g(v) \nonumber \\
    &\quad \sum_{n_{3,v}+n_{4,v}+n_{5,v}+n_{6,v}=\ell} \chi \{n_{3,v} +n_{4,v}> 0,n_{3,v} +n_{5,v}> 0, \|A_v\!\setminus\! B\|_\circ \geq \|A_v\|_\circ/2\}  \binom{l}{n_{3,v}~n_{4,v}~n_{5,v}~n_{6,v}} \nonumber \\
    &\quad \quad \quad \quad  \quad \quad \quad \quad \Vert A_v\cap B\Vert_\circ^{n_{3,v}}\Vert A_v\setminus B\Vert_\circ^{n_{4,v}}\Vert B\setminus A_v\Vert_\circ^{n_{5,v}} (1-\Vert  B \cup A_v\Vert_\circ)^{n_{6,v}} \frac{n_{3,v} + n_{5,v}}{n_{4,v}+1}  \nonumber \\
    &= 2 D_g(v) \sum_{n_{3,v}+n_{4,v}+n_{5,v}+n_{6,v}=\ell} \chi \{n_{3,v}=0, n_{4,v}> 0, n_{5,v}> 0, \|A_v\!\setminus\! B\|_\circ \geq \|A_v\|_\circ/2\}  \binom{l}{n_{4,v}~n_{5,v}~n_{6,v}} \nonumber \\
    &\quad \quad \quad \quad  \quad \quad \quad \quad \Vert A_v\setminus B\Vert_\circ^{n_{4,v}}\Vert B\setminus A_v\Vert_\circ^{n_{5,v}} (1-\Vert  B \cup A_v\Vert_\circ)^{n_{6,v}} \frac{n_{5,v}}{n_{4,v}+1} \nonumber \\
    &\quad + 2 D_g(v) \sum_{n_{3,v}+n_{4,v}+n_{5,v}+n_{6,v}=\ell} \chi \{n_{3,v}>0,\|A_v\!\setminus\! B\|_\circ \geq \|A_v\|_\circ/2\}  \binom{l}{n_{3,v}~n_{4,v}~n_{5,v}~n_{6,v}} \nonumber \\
    &\quad \quad \quad \quad  \quad \quad \quad \quad \Vert A_v\cap B\Vert_\circ^{n_{3,v}}\Vert A_v\setminus B\Vert_\circ^{n_{4,v}}\Vert B\setminus A_v\Vert_\circ^{n_{5,v}} (1-\Vert  B \cup A_v\Vert_\circ)^{n_{6,v}} \frac{n_{3,v} + n_{5,v}}{n_{4,v}+1} \label{32}
\end{align}

For the first term above ($n_{3,v}=0$), we rearrange $ \frac{n_{5,v}}{n_{4,v}+1}$ and complete the multinomial.
\begin{align}
    &2 D_g(v) \sum_{n_{3,v}+n_{4,v}+n_{5,v}+n_{6,v}=\ell} \chi \{n_{3,v}=0, n_{4,v}> 0, n_{5,v}> 0,\|A_v\!\setminus\! B\|_\circ \geq \|A_v\|_\circ/2\}  \binom{l}{n_{4,v}~n_{5,v}~n_{6,v}} \nonumber \\
    &\quad \quad \quad \quad  \quad \quad \quad \quad \Vert A_v\setminus B\Vert_\circ^{n_{4,v}}\Vert B\setminus A_v\Vert_\circ^{n_{5,v}} (1-\Vert  B \cup A_v\Vert_\circ)^{n_{6,v}} \frac{n_{5,v}}{n_{4,v}+1} \\
    &= 2 D_g(v) \sum_{n_{4,v}+n_{5,v}+n_{6,v}=\ell, 0<n_{4,v}<\ell,0<n_{5,v}<\ell} \chi \{ \|A_v\!\setminus\! B\|_\circ \geq \|A_v\|_\circ/2\}  \binom{l}{n_{4,v}~n_{5,v}~n_{6,v}} \nonumber \\
    &\quad \quad \quad \quad  \quad \quad \quad \quad \Vert A_v\setminus B\Vert_\circ^{n_{4,v}}\Vert B\setminus A_v\Vert_\circ^{n_{5,v}} (1-\Vert  B \cup A_v\Vert_\circ)^{n_{6,v}} \frac{n_{5,v}}{n_{4,v}+1} \\
    &= 2 D_g(v) \chi\{\|A_v\!\setminus\! B\|_\circ \geq \|A_v\|_\circ/2\} \frac{\Vert B\setminus A_v\Vert_\circ}{\Vert A_v\setminus B\Vert_\circ} \nonumber \\
    &\quad \sum_{(n_{4,v}+1)\geq 2,(n_{5,v}-1)\geq 0, (n_{4,v}+1)+(n_{5,v}-1)\leq\ell, n_{4,v}+1\leq \ell, n_{5,v}-1\leq \ell-2}   \binom{l}{n_{4,v}+1~n_{5,v}-1~n_{6,v}} \nonumber \\
    &\quad \quad \quad \quad  \quad \quad \quad \quad\quad \quad \quad \quad \quad \quad \Vert A_v\setminus B\Vert_\circ^{n_{4,v}+1}\Vert B\setminus A_v\Vert_\circ^{n_{5,v}-1} (1-\Vert  B \cup A_v\Vert_\circ)^{n_{6,v}}  \\
    &\leq 2 D_g(v)\chi\{\|A_v\!\setminus\! B\|_\circ \geq \|A_v\|_\circ/2\} \frac{\Vert B\setminus A_v\Vert_\circ}{\Vert A_v\setminus B\Vert_\circ} \nonumber \\
    &\quad \sum_{(n_{4,v}+1)\geq 0,(n_{5,v}-1)\geq 0, (n_{4,v}+1)+(n_{5,v}-1)\leq\ell, n_{4,v}+1\leq \ell, n_{5,v}-1\leq \ell}   \binom{l}{n_{4,v}+1~n_{5,v}-1~n_{6,v}} \nonumber \\
    &\quad \quad \quad \quad  \quad \quad \quad \quad \quad \quad \quad \quad \quad \quad \Vert A_v\setminus B\Vert_\circ^{n_{4,v}+1}\Vert B\setminus A_v\Vert_\circ^{n_{5,v}-1} (1-\Vert  B \cup A_v\Vert_\circ)^{n_{6,v}}  \\
    &= 2 D_g(v)\chi\{\|A_v\!\setminus\! B\|_\circ \geq \|A_v\|_\circ/2\} \frac{\Vert B\setminus A_v\Vert_\circ}{\Vert A_v\setminus B\Vert_\circ} \big(  
 \Vert A_v\setminus B\Vert_\circ + \Vert B\setminus A_v\Vert_\circ + (1-\Vert  B \cup A_v\Vert_\circ)\big)^\ell \\
 &= 2 \chi\{\|A_v\!\setminus\! B\|_\circ \geq \|A_v\|_\circ/2\}D_g(v) \frac{\Vert B\setminus A_v\Vert_\circ}{\Vert A_v\setminus B\Vert_\circ} \big(1-\Vert  B \cap A_v\Vert_\circ\big)^\ell \label{rrr}
\end{align}
% note: the constraint $n_{4,v}>0$ and $n_{5,v}>0$ means that for all nonzero terms, $\max(n_{4,v},n_{5,v})\leq \ell - 1$.

We argue similarly for the second term ($n_{3,v}>0$). Here we separate $\frac{n_{3,v} + n_{5,v}}{n_{4,v}+1}$ into two separate terms, one with $\frac{n_{3,v}}{n_{4,v}+1}$ and one with $\frac{n_{5,v}}{n_{4,v}+1}$, and complete the multinomial as usual.
\begin{align}
    &2  D_g(v)  \sum_{n_{3,v}+n_{4,v}+n_{5,v}+n_{6,v}=\ell} \chi \{n_{3,v}>0,\|A_v\!\setminus\! B\|_\circ \geq \|A_v\|_\circ/2\}  \binom{l}{n_{3,v}~n_{4,v}~n_{5,v}~n_{6,v}} \nonumber \\
    &\quad \quad \quad \quad  \quad \quad \quad \quad \Vert A_v\cap B\Vert_\circ^{n_{3,v}}\Vert A_v\setminus B\Vert_\circ^{n_{4,v}}\Vert B\setminus A_v\Vert_\circ^{n_{5,v}} (1-\Vert  B \cup A_v\Vert_\circ)^{n_{6,v}} \frac{n_{3,v} + n_{5,v}}{n_{4,v}+1}  \nonumber \\
    &= 2 D_g(v) \sum_{n_{3,v}+n_{4,v}+n_{5,v}+n_{6,v}=\ell} \chi \{ n_{3,v}>0,\|A_v\!\setminus\! B\|_\circ \geq \|A_v\|_\circ/2\}  \binom{l}{n_{3,v}~n_{4,v}~n_{5,v}~n_{6,v}} \nonumber \\
    &\quad \quad \quad \quad  \quad \quad \quad \quad \Vert A_v\cap B\Vert_\circ^{n_{3,v}}\Vert A_v\setminus B\Vert_\circ^{n_{4,v}}\Vert B\setminus A_v\Vert_\circ^{n_{5,v}} (1-\Vert  B \cup A_v\Vert_\circ)^{n_{6,v}} \frac{n_{3,v}}{n_{4,v}+1}  \nonumber \\
    &\quad + 2 D_g(v) \sum_{n_{3,v}+n_{4,v}+n_{5,v}+n_{6,v}=\ell} \chi \{n_{3,v}>0, \|A_v\!\setminus\! B\|_\circ \geq \|A_v\|_\circ/2\}  \binom{l}{n_{3,v}~n_{4,v}~n_{5,v}~n_{6,v}} \nonumber \\
    &\quad \quad \quad \quad  \quad \quad \quad \quad \Vert A_v\cap B\Vert_\circ^{n_{3,v}}\Vert A_v\setminus B\Vert_\circ^{n_{4,v}}\Vert B\setminus A_v\Vert_\circ^{n_{5,v}} (1-\Vert  B \cup A_v\Vert_\circ)^{n_{6,v}} \frac{n_{5,v}}{n_{4,v}+1}  \nonumber \\
    &= 2 \chi\{\|A_v\!\setminus\! B\|_\circ \geq \|A_v\|_\circ/2\} D_g(v)\frac{\Vert A_v\cap B\Vert_\circ}{\Vert A_v\setminus B\Vert_\circ} \nonumber\\
    &\quad \sum_{(n_{3,v}-1)+(n_{4,v}+1)+n_{5,v}+n_{6,v}=\ell, 0 \leq n_{3,v}-1\leq \ell-1, 1\leq n_{4,v}+1\leq \ell  }  \binom{l}{n_{3,v}-1~n_{4,v}+1~n_{5,v}~n_{6,v}} \nonumber \\
    &\quad \quad \quad \quad  \quad \quad \quad \quad \Vert A_v\cap B\Vert_\circ^{n_{3,v}-1}\Vert A_v\setminus B\Vert_\circ^{n_{4,v}+1}\Vert B\setminus A_v\Vert_\circ^{n_{5,v}} (1-\Vert  B \cup A_v\Vert_\circ)^{n_{6,v}}  \nonumber \\
    &\quad + 2 \chi\{\|A_v\!\setminus\! B\|_\circ \geq \|A_v\|_\circ/2\} D_g(v) \frac{\Vert B\setminus A_v\Vert_\circ}{\Vert A_v\setminus B\Vert_\circ} \nonumber \\
    &\quad \sum_{n_{3,v}+n_{4,v}+n_{5,v}+n_{6,v}=\ell,1 \leq n_{4,v}+1\leq \ell, 0 \leq n_{5,v}-1\leq \ell-2}  \binom{l}{n_{3,v}~n_{4,v}+1~n_{5,v}-1~n_{6,v}} \nonumber \\
    &\quad \quad \quad \quad  \quad \quad \quad \quad \Vert A_v\cap B\Vert_\circ^{n_{3,v}}\Vert A_v\setminus B\Vert_\circ^{n_{4,v}+1}\Vert B\setminus A_v\Vert_\circ^{n_{5,v}-1} (1-\Vert  B \cup A_v\Vert_\circ)^{n_{6,v}} \nonumber \\
    &\leq 2 \chi\{\|A_v\!\setminus\! B\|_\circ \geq \|A_v\|_\circ/2\} D_g(v)\frac{\Vert A_v\cap B\Vert_\circ}{\Vert A_v\setminus B\Vert_\circ} ( \Vert A_v\cap B\Vert_\circ+ \Vert A_v\setminus B\Vert_\circ+ \Vert B\setminus A_v\Vert_\circ+  1-\Vert  B \cup A_v\Vert_\circ)^\ell  \nonumber \\
    &\quad + 2 \chi\{\|A_v\!\setminus\! B\|_\circ \geq \|A_v\|_\circ/2\} D_g(v) \frac{\Vert B\setminus A_v\Vert_\circ}{\Vert A_v\setminus B\Vert_\circ} (\Vert A_v\cap B\Vert_\circ + \Vert A_v\setminus B\Vert_\circ + \Vert B\setminus A_v\Vert_\circ + 1-\Vert  B \cup A_v\Vert_\circ)^{\ell} \nonumber \\
    &= 2 \chi\{\|A_v\!\setminus\! B\|_\circ \geq \|A_v\|_\circ/2\} D_g(v)\frac{\Vert A_v\cap B\Vert_\circ+ \Vert B\setminus A_v\Vert_\circ}{\Vert A_v\setminus B\Vert_\circ}   \label{rr}
\end{align}
Note: $n_{3,v}>0$ implies $n_{4,v}+1 \leq \ell$, so we have not subtracted any terms. 
Combining \eqref{rr} and \eqref{rrr} yields
\begin{align}
     &\mathbb{E}  \left[\chi \{x \in A_v,n_{1,v} > 0,n_2 > 0,A_v\cap B\neq \emptyset,\|A_v\!\setminus\! B\|_\circ \geq \|A_v\|_\circ/2 \}  \frac{2n_2}{n_{1,v}+1} \right] \nonumber \\
    &\leq 2 \chi\{\|A_v\!\setminus\! B\|_\circ \geq \|A_v\|_\circ/2\}D_g(v)\frac{\Vert A_v\cap B\Vert_\circ+ \Vert B\setminus A_v\Vert_\circ \left(1+ \big(1-\Vert  B \cap A_v\Vert_\circ\big)^\ell\right)}{\Vert A_v\setminus B\Vert_\circ} \nonumber \\
    &= 2 \chi\{\|A_v\!\setminus\! B\|_\circ \geq \|A_v\|_\circ/2\}({\Vert A_v\cap B\Vert_\circ+ \Vert B\setminus A_v\Vert_\circ \left(1+ \big(1-\Vert  B \cap A_v\Vert_\circ\big)^\ell\right)}) \nonumber \\
    &\quad +  2 \chi\{\|A_v\!\setminus\! B\|_\circ \geq \|A_v\|_\circ/2\}\| A_v\cap B\|_\circ\frac{\Vert A_v\cap B\Vert_\circ + \Vert B\setminus A_v\Vert_\circ \left(1+ \big(1-\Vert  B \cap A_v\Vert_\circ\big)^\ell\right)}{\Vert A_v\setminus B\Vert_\circ} \nonumber \\
    &\leq 2 \chi\{\|A_v\!\setminus\! B\|_\circ \geq \|A_v\|_\circ/2\}({\Vert A_v\cap B\Vert_\circ+ \Vert B\setminus A_v\Vert_\circ \left(1+ \big(1-\Vert  B \cap A_v\Vert_\circ\big)^\ell\right)}) \nonumber \\
    &\quad +  4\| A_v\cap B\|_\circ\frac{\Vert A_v\cap B\Vert_\circ + \Vert B\setminus A_v\Vert_\circ \left(1+ \big(1-\Vert  B \cap A_v\Vert_\circ\big)^\ell\right)}{\Vert A_v\Vert_\circ}
\end{align}
which scales as $O(\|B\|_\circ)$, as desired.
We follow the same procedure for term 2 in \eqref{onehalf}:
\begin{align}
   & \mathbb{E}  \left[\chi \{x \in A_v,n_{1,v} > 0,n_2 > 0,A_v\cap B\neq \emptyset, \|A_v\cap B\|_\circ > \|A_v\|_\circ/2 \}  \frac{2n_2}{n_{1,v}+1} \right]  \nonumber \\
    &= D_g(v) \nonumber \\
    &\quad \sum_{n_{3,v}+n_{4,v}+n_{5,v}+n_{6,v}=\ell} \chi \{n_{3,v} +n_{4,v}> 0,n_{3,v} +n_{5,v}> 0, \|A_v\!\cap\! B\|_\circ \geq \|A_v\|_\circ/2  \}  \binom{l}{n_{3,v}~n_{4,v}~n_{5,v}~n_{6,v}} \nonumber \\
    &\quad \quad \quad \quad  \quad \quad \quad \quad \Vert A_v\cap B\Vert_\circ^{n_{3,v}}\Vert A_v\setminus B\Vert_\circ^{n_{4,v}}\Vert B\setminus A_v\Vert_\circ^{n_{5,v}} (1-\Vert  B \cup A_v\Vert_\circ)^{n_{6,v}} \frac{2(n_{3,v} + n_{5,v})}{n_{3,v} + n_{4,v}+1} \\
    &\leq  2 D_g(v)\nonumber \\
    &\quad \sum_{n_{3,v}+n_{4,v}+n_{5,v}+n_{6,v}=\ell} \chi \{n_{3,v} +n_{4,v}> 0,n_{3,v} +n_{5,v}> 0, \|A_v\!\cap\! B\|_\circ \geq \|A_v\|_\circ/2\}  \binom{l}{n_{3,v}~n_{4,v}~n_{5,v}~n_{6,v}} \nonumber \\
    &\quad \quad \quad \quad  \quad \quad \quad \quad \Vert A_v\cap B\Vert_\circ^{n_{3,v}}\Vert A_v\setminus B\Vert_\circ^{n_{4,v}}\Vert B\setminus A_v\Vert_\circ^{n_{5,v}} (1-\Vert  B \cup A_v\Vert_\circ)^{n_{6,v}} \frac{n_{3,v} + n_{5,v}}{n_{3,v}+1} \\
    &= 2 D_g(v) \sum_{n_{3,v}+n_{4,v}+n_{5,v}+n_{6,v}=\ell} \chi \{n_{3,v}=0, n_{4,v}> 0, n_{5,v}> 0, \|A_v\!\cap\! B\|_\circ \geq \|A_v\|_\circ/2\}  \binom{l}{0~n_{4,v}~n_{5,v}~n_{6,v}} \nonumber \\
    &\quad \quad \quad \quad  \quad \quad \quad \quad \Vert A_v\setminus B\Vert_\circ^{n_{4,v}}\Vert B\setminus A_v\Vert_\circ^{n_{5,v}} (1-\Vert  B \cup A_v\Vert_\circ)^{n_{6,v}} {n_{5,v}} \\
    &\quad + 2 D_g(v) \sum_{n_{3,v}+n_{4,v}+n_{5,v}+n_{6,v}=\ell} \chi \{n_{3,v}>0,\|A_v\!\cap\! B\|_\circ \geq \|A_v\|_\circ/2\}  \binom{l}{n_{3,v}~n_{4,v}~n_{5,v}~n_{6,v}} \nonumber \\
    &\quad \quad \quad \quad  \quad \quad \quad \quad \Vert A_v\cap B\Vert_\circ^{n_{3,v}}\Vert A_v\setminus B\Vert_\circ^{n_{4,v}}\Vert B\setminus A_v\Vert_\circ^{n_{5,v}} (1-\Vert  B \cup A_v\Vert_\circ)^{n_{6,v}} \frac{n_{3,v} + n_{5,v}}{n_{3,v}+1} \label{32}
\end{align}
For the first term in \eqref{32},
\begin{align}
    & 2 D_g(v) \sum_{n_{3,v}+n_{4,v}+n_{5,v}+n_{6,v}=\ell} \chi \{n_{3,v}=0, n_{4,v}> 0, n_{5,v}> 0, \|A_v\!\cap\! B\|_\circ \geq \|A_v\|_\circ/2\}  \binom{l}{0~n_{4,v}~n_{5,v}~n_{6,v}} \nonumber \\
    &\quad \quad \quad \quad  \quad \quad \quad \quad \Vert A_v\setminus B\Vert_\circ^{n_{4,v}}\Vert B\setminus A_v\Vert_\circ^{n_{5,v}} (1-\Vert  B \cup A_v\Vert_\circ)^{n_{6,v}} {n_{5,v}} \nonumber \\
    &= 2 D_g(v)\frac{\Vert B\setminus A_v\Vert_\circ}{1-\Vert  B \cup A_v\Vert_\circ} \nonumber \\
    &\quad \sum_{n_{4,v}+n_{5,v}\leq \ell} \chi \{ n_{4,v}> 0, n_{5,v}> 0, \|A_v\!\cap\! B\|_\circ \geq \|A_v\|_\circ/2\}  \binom{l}{n_{4,v}~n_{5,v}\!-\!1~(\ell- n_{4,v}-n_{5,v})} \nonumber \\
    &\quad \quad \quad \quad  \quad \quad \quad \quad \Vert A_v\setminus B\Vert_\circ^{n_{4,v}}\Vert B\setminus A_v\Vert_\circ^{n_{5,v}-1} (1-\Vert  B \cup A_v\Vert_\circ)^{\ell - n_{4,v} -(n_{5,v}-1)} \nonumber \\
    &= 2 D_g(v)\frac{\Vert B\setminus A_v\Vert_\circ}{1-\Vert  B \cup A_v\Vert_\circ} \nonumber \\
    &\quad \sum_{n_{4,v}+n_{5,v}\leq \ell, 1\leq n_{5,v}\leq \ell-1 } \chi \{ n_{4,v}> 0, n_{5,v}> 0, \|A_v\!\cap\! B\|_\circ \geq \|A_v\|_\circ/2\}  \binom{l}{n_{4,v}~n_{5,v}\!-\!1~(\ell- n_{4,v}-n_{5,v})} \nonumber \\
    &\quad \quad \quad \quad  \quad \quad \quad \quad \Vert A_v\setminus B\Vert_\circ^{n_{4,v}}\Vert B\setminus A_v\Vert_\circ^{n_{5,v}-1} (1-\Vert  B \cup A_v\Vert_\circ)^{\ell - n_{4,v} -(n_{5,v}-1)} \nonumber \\
    &\leq 2 \ell D_g(v)\frac{\Vert B\setminus A_v\Vert_\circ}{1-\Vert  B \cup A_v\Vert_\circ} \sum_{n_{4,v}+(n_{5,v}-1)\leq \ell} \chi \{  \|A_v\!\cap\! B\|_\circ \geq \|A_v\|_\circ/2\}  \binom{l}{n_{4,v}~n_{5,v}\!-\!1~(\ell- n_{4,v}-(n_{5,v}-1))} \nonumber \\
    &\quad \quad \quad \quad  \quad \quad \quad \quad \Vert A_v\setminus B\Vert_\circ^{n_{4,v}}\Vert B\setminus A_v\Vert_\circ^{n_{5,v}-1} (1-\Vert  B \cup A_v\Vert_\circ)^{\ell - n_{4,v} -(n_{5,v}-1)} \nonumber \\
    &= 2 \ell D_g(v)\frac{\Vert B\setminus A_v\Vert_\circ}{1-\Vert  B \cup A_v\Vert_\circ} \chi \{ \|A_v\!\cap\! B\|_\circ \geq \|A_v\|_\circ/2\}  ( \Vert A_v\setminus B\Vert_\circ+\Vert B\setminus A_v\Vert_\circ + 1-\Vert  B \cup A_v\Vert_\circ)^{\ell} \nonumber \\
 &= 2 \ell D_g(v)\frac{\Vert B\setminus A_v\Vert_\circ}{1-\Vert  B \cup A_v\Vert_\circ} \chi \{ \|A_v\!\cap\! B\|_\circ \geq \|A_v\|_\circ/2\}  ( 1-\Vert  B \cap A_v\Vert_\circ)^{\ell} \nonumber \\
 &\leq 2 \ell \Vert  A_v\Vert_\circ\frac{\Vert B\setminus A_v\Vert_\circ}{1-\Vert  B \cup A_v\Vert_\circ}   (1 - \Vert  A_v\Vert_\circ/2)^{\ell} \chi \{ \|A_v\!\cap\! B\|_\circ \geq \|A_v\|_\circ/2\}
\end{align}
Note: $\Vert  B \cup A_v\Vert_\circ$ is 1 only if $g$ is clean. so $\Vert  B \cup A_v\Vert_\circ < 1$. We will further upper bound $\Vert  B \cup A_v\Vert_\circ \leq 1/2$ by choice of $g'$.
% Also the sum for $n_{5,v}-1$ only adds (two) positive terms, so the upper bound with with the compressed polynomial is kosher.
Next for the second term in \eqref{32}. We split it into two terms, one with $n_{3,v}$ the other with $n_{5,v}$. For the $n_{3,v}$ term we have:
\begin{align}
    &2 D_g(v) \sum_{n_{3,v}+n_{4,v}+n_{5,v}+n_{6,v}=\ell} \chi \{n_{3,v}>0,\|A_v\!\cap\! B\|_\circ \geq \|A_v\|_\circ/2\}  \binom{l}{n_{3,v}~n_{4,v}~n_{5,v}~n_{6,v}} \nonumber \\
    &\quad \quad \quad \quad  \quad \quad \quad \quad \Vert A_v\cap B\Vert_\circ^{n_{3,v}}\Vert A_v\setminus B\Vert_\circ^{n_{4,v}}\Vert B\setminus A_v\Vert_\circ^{n_{5,v}} (1-\Vert  B \cup A_v\Vert_\circ)^{n_{6,v}} \frac{n_{3,v}}{n_{3,v}+1} \nonumber \\
    &\leq 2 \|A_v\|_\circ \chi \{\|A_v\!\cap\! B\|_\circ \geq \|A_v\|_\circ/2\}  \sum_{n_{3,v}+n_{4,v}+n_{5,v}+n_{6,v}=\ell}  \binom{l}{n_{3,v}~n_{4,v}~n_{5,v}~n_{6,v}} \nonumber \\
    &\quad \quad \quad \quad  \quad \quad \quad \quad \Vert A_v\cap B\Vert_\circ^{n_{3,v}}\Vert A_v\setminus B\Vert_\circ^{n_{4,v}}\Vert B\setminus A_v\Vert_\circ^{n_{5,v}} (1-\Vert  B \cup A_v\Vert_\circ)^{n_{6,v}} \nonumber \\
    &\leq 2 \|A_v\|_\circ \chi \{\|A_v\!\cap\! B\|_\circ \geq \|A_v\|_\circ/2\}  \nonumber 
\end{align}
which is small enough because  $\|A_v\|_\circ = O(\|B\|_\circ)$ whenever the indicator is 1.

For the $n_{5,v}$ term, note that its summand is zero whenever $n_{5,v}$ is zero. So we only need to consider nonzero $n_{5,v}>0$.  We have:
\begin{align}
    &2 D_g(v) \sum_{n_{3,v}+n_{4,v}+n_{5,v}+n_{6,v}=\ell} \chi \{n_{3,v}>0,\|A_v\!\cap\! B\|_\circ \geq \|A_v\|_\circ/2\}  \binom{l}{n_{3,v}~n_{4,v}~n_{5,v}~n_{6,v}} \nonumber \\
    &\quad \quad \quad \quad  \quad \quad \quad \quad \Vert A_v\cap B\Vert_\circ^{n_{3,v}}\Vert A_v\setminus B\Vert_\circ^{n_{4,v}}\Vert B\setminus A_v\Vert_\circ^{n_{5,v}} (1-\Vert  B \cup A_v\Vert_\circ)^{n_{6,v}} \frac{n_{5,v}}{n_{3,v}+1} \nonumber \\
    &= 2 \|A_v\|_\circ\frac{\Vert B\setminus A_v\Vert_\circ}{\Vert A_v\cap B\Vert_\circ} \sum_{(n_{3,v}+1)+n_{4,v}+(n_{5,v}-1)+n_{6,v}=\ell} \chi \{n_{3,v}>0,n_{5,v}>0,\|A_v\!\cap\! B\|_\circ \geq \|A_v\|_\circ/2\} \nonumber \\
    &\quad \quad \quad \quad  \binom{l}{n_{3,v}+1~n_{4,v}~n_{5,v}-1~n_{6,v}}  \Vert A_v\cap B\Vert_\circ^{n_{3,v}+1}\Vert A_v\setminus B\Vert_\circ^{n_{4,v}}\Vert B\setminus A_v\Vert_\circ^{n_{5,v}-1} (1-\Vert  B \cup A_v\Vert_\circ)^{n_{6,v}} \nonumber \\
    &\leq 2 \|A_v\|_\circ\frac{\Vert B\setminus A_v\Vert_\circ}{\Vert A_v\cap B\Vert_\circ}\chi \{\|A_v\!\cap\! B\|_\circ \geq \|A_v\|_\circ/2\}   \nonumber 
\end{align}
% note that $n_{5,v}>0$ implies that $n_{3,v}<\ell$, so we aren't subtracting a term (the $n_{3,v}+1=\ell+1$ term)  when compressing the polynomial.
Combining all terms, we can finally upper bound \eqref{onehalf}:
\begin{align}
    &\mathbb{E}  \left[\chi \{x \in A_v,n_{1,v} > 0,n_2 > 0,A_v\cap B\neq \emptyset \}  \frac{2n_2}{n_{1,v}+1} \right] \nonumber \\
    &\leq  2 \chi\{\|A_v\!\setminus\! B\|_\circ \geq \|A_v\|_\circ/2\}({\Vert A_v\cap B\Vert_\circ+ \Vert B\setminus A_v\Vert_\circ \left(1+ \big(1-\Vert  B \cap A_v\Vert_\circ\big)^\ell\right)}) \nonumber \\
    &\quad +  2 \chi\{\|A_v\!\setminus\! B\|_\circ \geq \|A_v\|_\circ/2\}\| A_v\cap B\|_\circ\frac{\Vert A_v\cap B\Vert_\circ + \Vert B\setminus A_v\Vert_\circ \left(1+ \big(1-\Vert  B \cap A_v\Vert_\circ\big)^\ell\right)}{\Vert A_v\setminus B\Vert_\circ} \nonumber \\
    &\quad + 2 \ell \Vert  A_v\Vert_\circ\frac{\Vert B\setminus A_v\Vert_\circ}{1-\Vert  B \cup A_v\Vert_\circ}   (1 - \Vert  A_v\Vert_\circ/2)^{\ell} \chi \{ \|A_v\!\cap\! B\|_\circ \geq \|A_v\|_\circ/2\} \nonumber \\
    &\quad +2 \|A_v\|_\circ \left(\frac{\Vert B\setminus A_v\Vert_\circ}{\Vert A_v\cap B\Vert_\circ}+1\right)\chi \{\|A_v\!\cap\! B\|_\circ \geq \|A_v\|_\circ/2\} 
    \end{align}
The first two lines are from $\{\|A_v\!\setminus\! B\|_\circ \geq \|A_v\|_\circ/2\}$, the others are 
from $\{\|A_v\!\cap\! B\|_\circ \geq \|A_v\|_\circ/2\} $, when $n_{3,v}=0$ (third line) and when it is nonzero. We can further upper bound:
\begin{align}
     &\mathbb{E}  \left[\chi \{x \in A_v,n_{1,v} > 0,n_2 > 0,A_v\cap B\neq \emptyset \}  \frac{2n_2}{n_{1,v}+1} \right] \nonumber \\
    &\leq 2 \chi\{\|A_v\!\setminus\! B\|_\circ \geq \|A_v\|_\circ/2\}({\Vert A_v\cap B\Vert_\circ+ 2\Vert B\setminus A_v\Vert_\circ }) \nonumber \\
    &\quad +  4 \chi\{\|A_v\!\setminus\! B\|_\circ \geq \|A_v\|_\circ/2\}\frac{\Vert A_v\cap B\Vert_\circ^2 + 2 \Vert A_v\cap B\Vert_\circ\Vert B\setminus A_v\Vert_\circ}{\Vert A_v\Vert_\circ} \nonumber \\
    &\quad + 4 \ell \Vert  A_v\cap B\Vert_\circ\frac{\Vert B\setminus A_v\Vert_\circ}{1-\Vert  B \cup A_v\Vert_\circ}   (1 - \Vert  A_v\Vert_\circ/2)^{\ell} \chi \{ \|A_v\!\cap\! B\|_\circ \geq \|A_v\|_\circ/2\} \nonumber \\
    &\quad +4 \|A_v\cap B\|_\circ \left(2\frac{\Vert B\setminus A_v\Vert_\circ}{\Vert A_v\Vert_\circ}+1\right)\chi \{\|A_v\!\cap\! B\|_\circ \geq \|A_v\|_\circ/2\} 
\end{align}
Note that all terms besides the third are $O(\|B\|_\circ)$ as desired.

% Concerns: do we have lower bound on $\|A_v\|_{\circ}$ when $A_v\cap B\neq \emptyset$? we don't need it.
% Do we have upper bound on $\Vert  B \cup A_v\Vert_\circ$?

Note that we can choose $g'$ such that $\|A_v\cup B\|\leq 1/2$ for all $v$.
% (which may require choosing the larger of two options for $B$). 
Argument: there are two options for $g'$. Each induces  $B,B'$, respectively. Let  $A_v,A_v'$ be the largest inverse sets that intersect with $B,\tilde{B}$, respectively. The sets $A_v \cup B$ and $\tilde{A}_v\cup \tilde{B}$ are disjoint. So $\|A_v \cup B\|_\circ + \| \tilde{A}_v\cup \tilde{B}\|_\circ \leq 1 \implies \min(\|A_v \cup B\|_\circ, \| \tilde{A}_v\cup \tilde{B}\|_\circ) \leq 1/2.$ It is easy to see that we can choose a $g'$ such that $\|A_v \cup B\|_\circ \leq 1/2$ for all $v$. Just choose $g'$ such that it is the opposite of the $g'$ that yields $\max_v  \|A_v \cup B\|_\circ$.
Thus we can further upper bound, using particular choice of $g'$ ($f_1'$),
\begin{align}
     &\mathbb{E}  \left[\chi \{x \in A_v,n_{1,v} > 0,n_2 > 0,A_v\cap B\neq \emptyset \}  \frac{2n_2}{n_{1,v}+1} \right] \nonumber \\
    &\leq 2 \chi\{\|A_v\!\setminus\! B\|_\circ \geq \|A_v\|_\circ/2\}({\Vert A_v\cap B\Vert_\circ+ 2\Vert B\setminus A_v\Vert_\circ }) \nonumber \\
    &\quad +  4 \chi\{\|A_v\!\setminus\! B\|_\circ \geq \|A_v\|_\circ/2\}\frac{\Vert A_v\cap B\Vert_\circ^2 + 2 \Vert A_v\cap B\Vert_\circ\Vert B\setminus A_v\Vert_\circ}{\Vert A_v\Vert_\circ} \nonumber \\
    &\quad + 8 \ell \Vert  A_v\cap B\Vert_\circ {\Vert B\setminus A_v\Vert_\circ}  (1 - \Vert  A_v\Vert_\circ/2)^{\ell} \chi \{ \|A_v\!\cap\! B\|_\circ \geq \|A_v\|_\circ/2\} \nonumber \\
    &\quad +4 \|A_v\cap B\|_\circ \left(2\frac{\Vert B\setminus A_v\Vert_\circ}{\Vert A_v\Vert_\circ}+1\right)\chi \{\|A_v\!\cap\! B\|_\circ \geq \|A_v\|_\circ/2\} 
\end{align}

For the fourth term in \eqref{4terms}, we have {
\begin{align}
&\mathbb{E}  \left[\chi \{x \in A_v,n_{1,v} > 0,n_2 > 0,  g'(x)^\top g'(x^+) \neq  g(x)^\top g(x^+), A_v\cap B\neq \emptyset \}  \frac{  2  }{n_{1,v}+1 } \right] \nonumber \\
&\leq \chi\{A_v\cap B\neq \emptyset \} \mathbb{P}  \left[x \in A_v \cap B, x^+ \notin B \right] 
\end{align}
}
