# Supplementary material for: InfoNCE Loss Provably Learns Cluster-Preserving Representations
Source: arXiv:2302.07920 source file (2023-02-15)
Supplement: Supplementary file 9 [file old_Agnostic.tex]

\begin{proof}
We first compare the difference in the positive term between $\tilde{L}(g)$ and $\tilde{L}(g_c)$. This is just
\begin{equation*}
\underset{x, x^+}{E}[\beta \left(g_c(x)g_c(x^+) - g(x)g(x^+)\right)]
\end{equation*}
Note that $\underset{x, x^+}{E}[\beta g_c(x)g_c(x^+)] = \beta d$, since clean representations are such that $g(x) = g(x^+)$ always. Meanwhile 
\begin{align*}
\underset{x, x^+}{E}[\beta g_c(x)g_c(x^+)] &\le  \beta d \Pr[g(x)= g(x^+)] + \beta(d-2)\Pr[g(x)\ne g(x^+)] \\
&= \beta(d-2) + 2\beta\left(1-\left(\Pr\left[x\in A, x^+\in B\right]+\Pr\left[x\in B, x^+\in A\right]\right)\right)
\end{align*}
The difference is
$$\underset{x, x^+}{E}[\beta \left(g_c(x)g_c(x^+) - g(x)g(x^+)\right)] \le 2\beta\left(\Pr\left[x\in A, x^+\in B\right]+\Pr\left[x\in B, x^+\in A\right]\right).$$ 

Now for the negative terms. Consider a cluster corresponding to $i\in \uH^d$. Consider the set $A_{v} = \{j\mid g(x_j^-) = v\}$ with $|A_v| = n_{1,v}$, and suppose $n_2$ negative samples are drawn from $B$. 

Recall that the negative term, is given by 
\begin{align*}
\tilde{L}_{\text{neg}}(g) 
&= \mathbb{E}_{x,x^+, \{x^-_i\}_{\ell}} \log\bigg({ e^{\beta g(x)^\top g(x^+)}\!+\!\sum_{i=1}^\ell e^{\beta g(x)^\top g(x^-_{i})}  } \bigg)
\end{align*}
and we are trying to upper bound $\tilde{L}_{\text{neg}}(g_c) - \tilde{L}_{\text{neg}}(g)$. We have the following cases.
\begin{enumerate}
\item In the event that $\{x\in A\}$, we have 
\begin{align*}
\tilde{L}_{\text{neg}}(g) 
&= \mathbb{E}_{x,x^+, \{x^-_i\}_{\ell}} \log\bigg({ e^{\beta g(x)^\top g(x^+)}\!+\!n_1e^{\beta d}+\sum_{i\not\in A} e^{\beta g(x)^\top g(x^-_{i})}  } \bigg)
\end{align*}
Meanwhile we have 
\begin{align*}
\tilde{L}_{\text{neg}}(g_c) 
&{\color{red}\leq} \mathbb{E}_{x,x^+, \{x^-_i\}_{\ell}} \log\bigg({ e^{\beta g_c(x)^\top g_c(x^+)}\!+\!(n_1+n_2)e^{\beta d}+\sum_{i\not\in A\cup B} e^{\beta g_c(x)^\top g_c(x^-_{i})}  } \bigg)
\end{align*}
\begin{enumerate}
\item if $n_2 = 0$, then $\tilde{L}_{\text{neg}}$ does not change. {\color{red} increases by at most $2\beta $ due to positive pair}
\item if $n_1 = 0, n_2 > 0$, then $\tilde{L}_{\text{neg}}$ increases by at most $2\beta$ (since each term in the argument of the $\log$ can increase by no more than a multiplicative factor of $2\beta$). This happens with probability $(1-D_g(i))^l l\Vert B\Vert_\circ$, that is, there is a probability $(1-D_g(i))^l$ that no negative sample is sampled from the same cluster, and a probability $l\delta$ that $n_2 > 0$. 
\item $n_1, n_2 > 0$. We denote the conditional expectation under this case using the notation $\E\left[\cdot | \circled{1c}\right]$. Then $\tilde{L}_{\text{neg}}$ increases by at most 
\begin{align*}
&\mathbb{E}_{x,x^+, \{x^-_i\}_{\ell}} \log\bigg({ e^{\beta g(x)^\top g(x^+)}\!+\!(n_1+n_2)e^{\beta d}+\sum_{i\not\in A\cup B} e^{\beta g(x)^\top g(x^-_{i})}  } \bigg) \\
&\quad\quad- \log\bigg({ e^{\beta g(x)^\top g(x^+)}\!+\!n_1e^{\beta d}+\sum_{i\not\in A} e^{\beta g(x)^\top g(x^-_{i})}  } \bigg)|\circled{1c}\\
&\quad\le  \mathbb{E}_{x,x^+, \{x^-_i\}_{\ell}} \left[\log\bigg((n_1+n_2)e^{\beta d} \bigg) - \mathbb{E}_{x,x^+, \{x^-_i\}_{\ell}} \log\bigg( n_1e^{\beta d}\bigg)\mid \circled{1c}\right]\\
&\quad\le \E_{x, x^+, \{x^-_i\}_l}\left[\log\left(1+\frac{n_2}{n_1}\right)\mid \circled{1c}\right]\\
&=\quad\sum_{n_1, n_2\ne 0, n_3} \binom{l}{n_1~n_2~n_3} \Vert A\Vert_\circ^{n_1}\Vert B\Vert_\circ^{n_2}\Vert 1-A-B\Vert_\circ^{n_3}\log\left(1+\frac{n_2}{n_1}\right)\\
&\le\sum_{n_1\ne 0, n_2\ne 0, n_3} \binom{l}{n_1~n_2~n_3} \Vert A\Vert_\circ^{n_1}\Vert B\Vert_\circ^{n_2}\Vert 1-A-B\Vert_\circ^{n_3}\frac{2n_2}{n_1+1}\\
&\le 2\frac{\Vert B\Vert_\circ}{\Vert A\Vert_\circ}\sum_{n_1, n_2, n_3} \binom{l}{n_1+1~n_2-1~n_3} \Vert A\Vert_\circ^{n_1+1}\Vert B\Vert_\circ^{n_2-1}\Vert 1-A-B\Vert_\circ^{n_3}\le  2\frac{\Vert B\Vert_\circ}{\Vert A\Vert_\circ}
\end{align*}
\end{enumerate}
Overall, for case $\circled{1}$, this gives a total 
\begin{align*}
0\cdot\Pr[\circled{1a}]+2\beta \Pr[\circled{1b}] + \frac{\Vert B\Vert_\circ}{\Vert A\Vert_\circ} \Pr[\circled{1c}]=2\beta \sum_{i\in \uH^d} D_g(i)\left(1-D_g(i)\right)^ll\delta + 2\frac{\Vert B\Vert_\circ}{\Vert A\Vert_\circ}
\end{align*}
\item In the event that $\{x\in B\}$, we have 
\begin{enumerate}
\item if $n_1 = 0$, then $\tilde{L}_{\text{neg}}$ does not change.
\item if $n_2 = 0, n_1>0$, then similarly to case $\circled{1b}$, the loss increases by at most $2\beta$.
\item if $n_1, n_2 > 0$, similar to the case $\circled{1c}$, the loss increases by at most $\log\left(1+\frac{n_1}{n_2}\right)\le n_1$. Note that $n_2 > 0$ with probability no more than $l\Vert B\Vert_\circ$. Now we have
\begin{align*}
&=\sum_{n_1, n_2\ne 0, n_3} \binom{l}{n_1~n_2~n_3} \Vert A\Vert_\circ^{n_1}\Vert B\Vert_\circ^{n_2}\Vert 1-A-B\Vert_\circ^{n_3}\log\left(1+n_1\right)\\
&\le\sum_{n_1\ne 0, n_2\ne 0, n_3} \binom{l}{n_1~n_2~n_3} \Vert A\Vert_\circ^{n_1}\Vert B\Vert_\circ^{n_2}\Vert 1-A-B\Vert_\circ^{n_3}n_1\\
&\le \Vert A\Vert_\circ\sum_{n_1\ne l, n_2\ne 0, n_3} \binom{l}{n_1-1~n_2~n_3} \Vert A\Vert_\circ^{n_1-1}\Vert B\Vert_\circ^{n_2}\Vert 1-A-B\Vert_\circ^{n_3}\le  \Vert A\Vert_\circ
\end{align*}
\end{enumerate}
This gives a total increase, conditioned on $\circled{2}$ of $2\beta (1-\Vert B\Vert_\circ)^l + 2\Vert A\Vert_\circ l\Vert B \Vert_\circ$.
% \begin{align*}
% \tilde{L}_{\text{neg}(g)}-\tilde{L}_{\text{neg}(g_c)}
% &\le\sum_{n_1\ne 0, n_2, n_3} \binom{l}{n_1~n_2~n_3} \Vert A\Vert_\circ^{n_1}\Vert B\Vert_\circ^{n_2}\Vert C\Vert_\circ^{n_3}\log\left(1+\frac{n_1}{n_2+1}\right)\\
% &\le\sum_{n_1\ne 0, n_2, n_3} \binom{l}{n_1~n_2~n_3} \Vert A\Vert_\circ^{n_1}\Vert B\Vert_\circ^{n_2}\Vert C\Vert_\circ^{n_3}\frac{n_1}{n_2+1}\\
% &\le\frac{\Vert A\Vert_\circ}{\Vert B\Vert_\circ}\sum_{n_1, n_2, n_3} \binom{l}{n_1-1~n_2+1~n_3} \Vert A\Vert_\circ^{n_1-1}\Vert B\Vert_\circ^{n_2+1}\Vert C\Vert_\circ^{n_3}\le  \frac{\Vert A\Vert_\circ}{\Vert B\Vert_\circ}
% \end{align*}
\item In the event that $\{x\in C\}$, the negative loss cannot possibly increase. This is because $h(g_c(x'), g_c(x)) \ge h(g(x'), g(x))$, so each of the terms in the argument can only decrease.
\end{enumerate}
Over all, we have
\begin{align*}
\tilde{L}_{\text{neg}}(g_c) -\tilde{L}_{\text{neg}}(g)
&\le \Pr\left[\circled{1}\right] \left(2\beta \sum_{i\in \uH^d} D_g(i)\left(1-D_g(i)\right)^ll\delta + 2\frac{\Vert B\Vert_\circ}{\Vert A\Vert_\circ}\right)+ \Pr\left[\circled{2}\right]\left(2\beta (1-\Vert B\Vert_\circ)^l + 2\Vert A\Vert_\circ l\Vert B \Vert_\circ\right)\\
&\le \Vert A\Vert_\circ \left(2\beta \sum_{i\in \uH^d} \frac{1}{2^d}e^{-2^dl}l\delta + 2\frac{\Vert B\Vert_\circ}{\Vert A\Vert_\circ}\right)+ \Vert B\Vert_\circ\left(2\beta (1-\Vert B\Vert_\circ)^l + 2\Vert A\Vert_\circ l\Vert B \Vert_\circ\right)\\
&\le 2\beta \sum_{i\in \uH^d} \frac{1}{2^d}e^{-2^dl}l\delta + 2\Vert B\Vert_\circ+ 2\beta \Vert B\Vert_\circ(1-\Vert B\Vert_\circ)^l + 2\Vert A\Vert_\circ l\Vert B \Vert^2_\circ
\end{align*}

\end{proof}




If the distribution is close to uniform, then it makes sense to move to clean. but what if you move so much that you become non-uniform? 


this analysis should address case where number of clusters $\gg 2^d$.

In case with two clusters, can we show that optimal rep is clean

show that negative loss is submodular wrt d

greedy algorithm to minimize negative loss gives uniform solution

by submodularity the greedy solution is close to optimal , i.e. optimal is close to uniform

is full loss submodular? 

If one $\|A_v\|_\circ < c 2^{-d}$ then we need a whole new analysis because we need to choose a different $g_c$.

\subsection{$\|A_v\|_\circ < c 2^{-d}$ for some $v$}

We need to lower bound gain for $x\in C$. 

If any $A_v$ is that small, then its boundary must split a cluster.


Loss improves iff $x \in \{x \notin B : f_1(x)= f_1(x'), x'\in B\}$. 
% Select $g_c$ to maximize $ \sum_v \|A_v \setminus B\|_\circ$ for 

Define $C :=\{x \notin B : f_1(x)= f_1(B)\}$ where $f_1$ is the classifier that gets changed to $f_1'$. (note that $f_1$ is constant on $B$)

Note that either $A_v \cap C = A_v\setminus B$ or $A_v \cap C = \emptyset$.

\begin{align}
&\mathbb{E}  \left[\chi \{x \in A_v\cap C ,n_{1,v} > 0,n_2 > 0\}  \log\bigg({ e^{\beta g_c(x)^\top g_c(x^+)}+ n_{1,v}e^{\beta d} + \sum_{x_i^{-} \in B}e^{\beta g_c(x)^\top g_c(x^-_{i})}  +\sum_{x_i^{-}\not\in {A}_v\cup B} e^{\beta g(x)^\top g(x^-_{i})}  } \bigg) \right]\nonumber \\
    &\quad - \mathbb{E} \left[\chi \{x \in A_v\cap C,n_{1,v} > 0,n_2 > 0\}   \log\bigg({ e^{\beta g(x)^\top g(x^+)}+n_{1,v}e^{\beta d} + \sum_{x_i^{-} \in B}e^{\beta g(x)^\top g(x^-_{i})}  +\sum_{x_i^{-}\not\in {A}_v\cup B} e^{\beta g(x)^\top g(x^-_{i})}  } \bigg) \right] \label{dif4} \\
% &\leq \mathbb{E}  \left[\chi \{x \in A_v\cap C ,n_{1,v} > 0,n_2 > 0\}  \log\bigg({  n_{1,v}e^{\beta d} + e^{-2\beta} \sum_{x_i^{-} \in B}e^{\beta g(x)^\top g(x^-_{i})}    } \bigg) \right]\nonumber \\
%     &\quad - \mathbb{E} \left[\chi \{x \in A_v\cap C,n_{1,v} > 0,n_2 > 0\}   \log\bigg({ n_{1,v}e^{\beta d} + \sum_{x_i^{-} \in B}e^{\beta g(x)^\top g(x^-_{i})}   } \bigg) \right] \nonumber \\
    &= \mathbb{E}  \left[\chi \{x \in A_v\cap C ,n_{1,v} > 0,n_2 > 0\}  \log\bigg({ e^{\beta g(x)^\top g(x^+)}+ n_{1,v}e^{\beta d} + e^{-2\beta}\sum_{x_i^{-} \in B}e^{\beta g(x)^\top g(x^-_{i})}  +\sum_{x_i^{-}\not\in {A}_v\cup B} e^{\beta g(x)^\top g(x^-_{i})}  } \bigg) \right]\nonumber \\
    &\quad - \mathbb{E} \left[\chi \{x \in A_v\cap C,n_{1,v} > 0,n_2 > 0\}   \log\bigg({ e^{\beta g(x)^\top g(x^+)}+n_{1,v}e^{\beta d} + \sum_{x_i^{-} \in B}e^{\beta g(x)^\top g(x^-_{i})}  +\sum_{x_i^{-}\not\in {A}_v\cup B} e^{\beta g(x)^\top g(x^-_{i})}  } \bigg) \right] \nonumber \\
    &\leq 
\end{align}
note $x \in A_v\cap C \implies g_c(x^+) = g(x^+)$, likewise for $x$

note: $(N + x)/(N+y)\leq x/y$ inequality only holds if $x>y$.

so we want $e^{\beta g(x)^\top g(x^+)}+ n_{1,v}e^{\beta d}  +\sum_{x_i^{-}\not\in {A}_v\cup B} e^{\beta g(x)^\top g(x^-_{i})}  $ to be small relative to $\sum_{x_i^{-} \in B}e^{\beta g(x)^\top g(x^-_{i})}  $

note: $\sum_{x_i^{-}\not\in {A}_v\cup B} e^{\beta g(x)^\top g(x^-_{i})} \leq (\ell - n_{1,v} - n_2)e^{\beta(d-2)}$

and $e^{\beta g(x)^\top g(x^+)} \leq e^{\beta d}$ is tight.

How can we lower bound $\sum_{x_i^{-} \in B}e^{\beta g(x)^\top g(x^-_{i})}  $? by choice of $g_c$ we can ensure each of these is $e^{\beta d}$ - no.

Worst case they are $e^{-\beta(d-2)}$

but this is in an extreme case. can we show that in this case, you would choose a more uniform $g_c$?

but it has to be a particular uniform $g_c$. The nearest clean neighbor may not always improve the loss.


bad case: d-1 classifiers are the same. One bad classifier cuts one  cluster. The choice of $f_{1,c}$ is equal to all the other classifiers.

Our upper bound on difference in negative terms is:
\begin{align}
     &\leq 27*2^d \|B\|_\circ  + 2 \beta_2 (\ell \log(\ell+1) +1) \|B\|_\circ  \sum_{v \in \mathcal{H}_d} \|A_v\|_\circ (1 - \|A_v\|_\circ)^\ell  \nonumber \\
    &\quad + 8\ell \|B\|_\circ \sum_{v \in \mathcal{H}_d} \Vert  A_v\Vert_\circ   (1 - \Vert  A_v\Vert_\circ/2)^{\ell}  \nonumber \\
    &\quad \underbrace{\sum_{v\in \mathcal{H}_d} \chi\{A_v\cap B= \emptyset \} \mathbb{P}  \left[x \in A_v, x^+\in B\right] + \chi\{A_v\cap B\neq \emptyset \} \mathbb{P}  \left[x \in A_v \cap B, x^+ \notin B \right]}_{\text{area of shaded region}} \nonumber \\
    &\leq 27*2^d \|B\|_\circ  + 2 \beta_2 (\ell \log(\ell+1) +1) \|B\|_\circ  \frac{2^d}{\ell+1} \left(1 - \frac{1}{\ell+1}\right)^\ell \nonumber \\
    &\quad + 8\ell \|B\|_\circ \frac{2^{d+1}}{\ell+1}\left( 1 - \frac{1}{\ell+1} \right)^\ell  \nonumber \\
    &\quad \underbrace{\sum_{v\in \mathcal{H}_d} \chi\{A_v\cap B= \emptyset \} \mathbb{P}  \left[x \in A_v, x^+\in B\right] + \chi\{A_v\cap B\neq \emptyset \} \mathbb{P}  \left[x \in A_v \cap B, x^+ \notin B \right]}_{\text{area of shaded region}} \nonumber \\
    &\leq 27*2^d \|B\|_\circ  + 2 e \beta_2 2^{2d} d \log(d) \|B\|_\circ + 16 e  2^{2d}  \|B\|_\circ    \nonumber \\
    &\quad \underbrace{\sum_{v\in \mathcal{H}_d} \chi\{A_v\cap B= \emptyset \} \mathbb{P}  \left[x \in A_v, x^+\in B\right] + \chi\{A_v\cap B\neq \emptyset \} \mathbb{P}  \left[x \in A_v \cap B, x^+ \notin B \right]}_{\text{area of shaded region}} \nonumber 
\end{align}
$\implies$ choose $\beta_2 = o(1)$ and $\beta_1 = \Omega(4^d)$



{\color{red} but why should large $\ell, \beta$ lead to  clean representations???? large $\ell$ might make sense but it shouldn't be allowed to be infinitely large. What are we missing?

Intuition: by scaling up $\beta$ we make the log sum more like a max. Also, with large $\ell$ we are likely to have a negative sample in the same inverse set as $x$. so there is likely to be $e^{\beta d}$ terms in both log sums. So the negaitve loss  doens't change very much. Does this hold with continuous representations?

No....there is an error
}


{\color{red} the sums maybe large. the one problem term is from case 1b. i think the analysis there is tight...it seems like it doesn't work....

can we use that: all of the small sets must cut a cluster -- can we pick the nicest one for $g_c$?

if the Av's are uniform/close to uniform to begin with, then we have a result.


if the Av's are small, can we use this? no 1b analysis is tight

knowing the Av's are small, how can we choose a gc that encourages uniformity?

it should improve the negative loss overall, even though it gets worse if x in Av, but our bound is not capturing this...
}



% Ignoring second order and higher terms and summing over all $v$ we obtain
% \begin{align}
%   \sum_v   2 {\|B\|_\circ} ( 1 + \Vert A_v \cap B \Vert_\circ  )^\ell  \lesssim 2^{d+1} {\|B\|_\circ} + 2 \ell \|B\|_\circ^2 \label{nottru}
% \end{align}
% which implies that we need to choose $\beta \gg  \ell + 2^{d+1}$.

% Can we use that Av cap B not empty implies $x$ might be in $B$? 


% If $x\in A_v\cap B$, then the bound should be.... right, just need to be more careful with the binomial expansion, it can be fixed
% \begin{align}
%     &\mathbb{E}  \left[\chi \{x \in A_v,n_{1,v} > 0,n_2 > 0\}  \frac{2n_2}{n_{1,v}+1} \right] \nonumber \\
%     % &= \mathbb{P}(x \in A_v) \sum_{n_{1,v}=0}^\ell \sum_{n_{2}=0}^\ell \sum_{n_{3}=0}^\ell  \chi \{n_{1,v} > 0,n_2 > 0\}  \binom{l}{n_{1,v}~n_2~n_3} \Vert A_v\Vert_\circ^{n_{1,v}}\Vert B\Vert_\circ^{n_2}\Vert 1-A_v-B\Vert_\circ^{n_3}\frac{2n_2}{n_{1,v}+1} \\
%     % &= 2\mathbb{P}(x \in A_v)\sum_{n_{1,v}=1}^\ell \sum_{n_{2}=1}^\ell \sum_{n_{3}=0}^\ell   \binom{l}{n_{1,v}~n_2~n_3} \Vert A\Vert_\circ^{n_{1,v}}\Vert B\Vert_\circ^{n_2}\Vert 1-A_v-B\Vert_\circ^{n_3}\frac{n_2}{n_{1,v}+1} \\
%     % &= 2\mathbb{P}(x \in A_v) \frac{\|B\|_\circ}{\|A_v\|_\circ} \sum_{n_{1,v}=1}^\ell \sum_{n_{2}=1}^\ell \sum_{n_{3}=0}^\ell   \binom{l}{n_{1,v}+1~n_2-1~n_3} \Vert A_v\Vert_\circ^{n_{1,v}+1}\Vert B\Vert_\circ^{n_2-1}\Vert 1-A_v-B\Vert_\circ^{n_3} \\
%     % &\leq 2\mathbb{P}(x \in A_v) \frac{\|B\|_\circ}{\|A_v\|_\circ} \sum_{n_{1,v}+1=0}^\ell \sum_{n_{2}-1=0}^\ell \sum_{n_{3}=0}^\ell   \binom{l}{n_{1,v}+1~n_2-1~n_3} \Vert A_v\Vert_\circ^{n_{1,v}+1}\Vert B\Vert_\circ^{n_2-1}\Vert 1-A_v-B\Vert_\circ^{n_3} \\
%     % &= 2{\|B\|_\circ} ( \Vert A_v\Vert_\circ + \Vert B\Vert_\circ + \Vert 1-A_v-B\Vert_\circ)^\ell  \nonumber \\
%     % &= 2 {\|B\|_\circ} ( 1 + \Vert A_v \cap B \Vert_\circ  )^\ell  \nonumber 
% \end{align}

% also need to deal with second term

% }



% {\color{red}
% Now let's see if the result will hold with the overly optimistic bound in \eqref{nottru}. We have
% \begin{align}
%      &\sum_v   \mathbb{P}(x \in A_v \cap x^+ \in B) ( 2 \beta D_g(v)(1 - D_g(v) - \|B\|_0)^\ell + \log(2) D_g(v))\nonumber \\
%      &+ \sum_v  2 \beta \ell \log(\ell+1) D_g(v) (1 - D_g(v))^\ell  \mathbb{P} ( x_{1}^- \in B |  x_{1}^- \notin A_v) \nonumber \\
%      &+ {\color{gray}2^{d+1} {\|B\|_\circ} + 2 \ell \|B\|_\circ^2}
% \end{align}


% note that we only need to sum over vertices whose inverse sets are to the left of $g$
% }

% \item In the event that $\{x\in B\}$, we have 
% \begin{enumerate}
% \item if $n_1 = 0$, then $\tilde{L}_{\text{neg}}$ does not change. {\color{red} both the negative and positive inner products may increase. but we have already covered this case.}
% \item if $n_2 = 0, n_1>0$, then similarly to case $\circled{1b}$, the loss increases by at most $2\beta$. {\color{red} we have already covered this case}
% \item if $n_1, n_2 > 0$, similar to the case $\circled{1c}$, the loss increases by at most $\log\left(1+\frac{n_1}{n_2}\right)\le n_1$. Note that $n_2 > 0$ with probability no more than $l\Vert B\Vert_\circ$. {\color{red} we have already covered this case but our bound is loose.} Now we have
% \begin{align*}
% &=\sum_{n_1, n_2\ne 0, n_3} \binom{l}{n_1~n_2~n_3} \Vert A\Vert_\circ^{n_1}\Vert B\Vert_\circ^{n_2}\Vert 1-A-B\Vert_\circ^{n_3}\log\left(1+n_1\right)\\
% &\le\sum_{n_1\ne 0, n_2\ne 0, n_3} \binom{l}{n_1~n_2~n_3} \Vert A\Vert_\circ^{n_1}\Vert B\Vert_\circ^{n_2}\Vert 1-A-B\Vert_\circ^{n_3}n_1\\
% &\le \Vert A\Vert_\circ\sum_{n_1\ne l, n_2\ne 0, n_3} \binom{l}{n_1-1~n_2~n_3} \Vert A\Vert_\circ^{n_1-1}\Vert B\Vert_\circ^{n_2}\Vert 1-A-B\Vert_\circ^{n_3}\le  \Vert A\Vert_\circ
% \end{align*}
% \end{enumerate}
% This gives a total increase, conditioned on $\circled{2}$ of $2\beta (1-\Vert B\Vert_\circ)^l + 2\Vert A\Vert_\circ l\Vert B \Vert_\circ$.
% \item In the event that $\{x\in C\}$, the negative loss cannot possibly increase. This is because $h(g_c(x'), g_c(x)) \ge h(g(x'), g(x))$, so each of the terms in the argument can only decrease.
% \end{enumerate}
% Over all, we have
% \begin{align*}
% \tilde{L}_{\text{neg}}(g_c) -\tilde{L}_{\text{neg}}(g)
% &\le \Pr\left[\circled{1}\right] \left(2\beta \sum_{i\in \uH^d} D_g(i)\left(1-D_g(i)\right)^ll\delta + 2\frac{\Vert B\Vert_\circ}{\Vert A\Vert_\circ}\right)+ \Pr\left[\circled{2}\right]\left(2\beta (1-\Vert B\Vert_\circ)^l + 2\Vert A\Vert_\circ l\Vert B \Vert_\circ\right)\\
% &\le \Vert A\Vert_\circ \left(2\beta \sum_{i\in \uH^d} \frac{1}{2^d}e^{-2^dl}l\delta + 2\frac{\Vert B\Vert_\circ}{\Vert A\Vert_\circ}\right)+ \Vert B\Vert_\circ\left(2\beta (1-\Vert B\Vert_\circ)^l + 2\Vert A\Vert_\circ l\Vert B \Vert_\circ\right)\\
% &\le 2\beta \sum_{i\in \uH^d} \frac{1}{2^d}e^{-2^dl}l\delta + 2\Vert B\Vert_\circ+ 2\beta \Vert B\Vert_\circ(1-\Vert B\Vert_\circ)^l + 2\Vert A\Vert_\circ l\Vert B \Vert^2_\circ
% \end{align*}

% \end{proof}
% }
