# Supplementary material for: InfoNCE Loss Provably Learns Cluster-Preserving Representations
Source: arXiv:2302.07920 source file (2023-02-15)
Supplement: Supplementary file 10 [file old_Agnostic_largeR.tex]

\begin{proof}
For all $v \in \mathcal{H}_d$, define the sets $A_v := \{x \in \mathcal{D}_\circ \cup \mathcal{D} : g(x)=v, g'(x)=v \}$ and $B_v := \{x \in \mathcal{D}_\circ \cup \mathcal{D} : g(x)= v, g'(x)\neq v \}$. 
% $\bar{A}_{v} = \{j\mid g(x_j^-) = v\}$ with $n_{1,v} := |\bar{A}_v| $ (random), 
% Note that $\|A_v\|_\circ = D_g(v)$. 
Let  $A:=s \cup_v A_v$ and $B:= \cup_v B_v$.

Since $g= [f_1,\dots,f_d]$ is not clean, there exists $j\in [d]$ such that $f_j$ is not clean. WLOG let this $j=1$. Let $S$ denote one of the clusters that $f_1$ intersects. 
Construct $g' =[f_1',f_2,\dots,f_d]$ where $f_1'(x) = f_1(x)$ for all $ x \notin S$. 
Define the set 
 $B := \{x \in \mathcal{D}_\circ \cup \mathcal{D}: f_1(x) \neq f_1'(x) \} \subset S$. 
Let  $f_1'(x) = 1$ or $f_1'(x) = -1$ for all $x \in S$, 
whichever induces smaller $\|B\|_\circ$.

% Now for the negative terms. Consider a cluster corresponding to $v \in \uH^d$. 

% ($B$ is deterministic, $n_2$ is random). 
% Also note that here $A_v$  is totally unrelated  to the set $A$ in the picture.

We would like to show that $\mathcal{L}(g)- \mathcal{L}(g')>0$, where
\begin{align}
    \mathcal{L}(g)- \mathcal{L}(g') = \mathcal{L}_{\text{pos}}(g) - \mathcal{L}_{\text{pos}}(g') + \mathcal{L}_{\text{neg}}(g) - \mathcal{L}_{\text{neg}}(g').
\end{align}
For the positive losses, we have
\begin{align*}
\mathcal{L}_{\text{pos}}(g) - \mathcal{L}_{\text{pos}}(g') &= 
\beta \mathbb{E}_{x, x^+}\left[\left(g'(x)^\top g'(x^+) - g(x)^\top g(x^+)\right)\right] \nonumber \\
&= \beta \mathbb{E}_{x, x^+}\left[\left(f_1'(x) f_1'(x^+) - f_1(x) f_1(x^+)\right)\right] \nonumber \\
&= 2\beta \sum_{v \in \mathcal{A}_v}\left(\Pr\left[x\in A, x^+\in B\right]+\Pr\left[x\in B, x^+\in A\right]\right) 
\end{align*}
% Meanwhile 
% \begin{align*}
% \underset{x, x^+}{E}[\beta g'(x)g'(x^+)] &\le  \beta d \Pr[g(x)= g(x^+)] + \beta(d-2)\Pr[g(x)\ne g(x^+)] \\
% &= \beta(d-2) + 2\beta\left(1-\left(\Pr\left[x\in A, x^+\in B\right]+\Pr\left[x\in B, x^+\in A\right]\right)\right)
% \end{align*}
% The difference is
% \begin{align}
% \underset{x, x^+}{E}[\beta \left(g'(x)g'(x^+) - g(x)g(x^+)\right)] \le 2\beta\left(\Pr\left[x\in A, x^+\in B\right]+\Pr\left[x\in B, x^+\in A\right]\right) 
% &= 2\beta \Delta_f^{new}
% \end{align}{\color{red}(A and B are as in the picture), and $\Delta_f^{new}$ defined as the fraction of natural images whose augmentation sets are split by $f$.}

Now we consider the negative losses. For a batch of samples $\{x_{i}^-\}_{i=1}^\ell$ and a vertex $v\in \mathcal{H}_d$, let $n_{1,v}:= \sum_{i=1}^\ell \chi\{ x_{i}^- \in A_v \}$ and $n_{2}:= \sum_{i=1}^\ell \chi\{ x_{i}^- \in B \}$. Also let $n_{3,v}:= \sum_{i=1}^\ell \chi\{ x_{i}^- \in B_v \}$ and $n_{4}:= \sum_{i=1}^\ell \chi\{ x_{i}^- \in A \}$.

Recall that the negative loss is given by 
\begin{align*}
{L}_{\text{neg}}(g) 
&= \mathbb{E}_{x,x^+, \{x^-_i\}_{\ell}} \log\bigg({ e^{\beta g(x)^\top g(x^+)}\!+\!\sum_{i=1}^\ell e^{\beta g(x)^\top g(x^-_{i})}  } \bigg) \nonumber \\
&= \sum_{v \in \uH_{d}} \mathbb{E}_{x,x^+, \{x^-_i\}_{\ell}} \chi \{x \in A_v\}  \log\bigg({ e^{\beta g(x)^\top g(x^+)}\!+\!\sum_{i=1}^\ell e^{\beta g(x)^\top g(x^-_{i})}  } \bigg)  \nonumber \\
&\quad + \sum_{v \in \uH_{d}} \mathbb{E}_{x,x^+, \{x^-_i\}_{\ell}} \chi \{x \in B_v\}  \log\bigg({ e^{\beta g(x)^\top g(x^+)}\!+\!\sum_{i=1}^\ell e^{\beta g(x)^\top g(x^-_{i})}  } \bigg)  \nonumber \\
&= \sum_{v \in \uH_{d}} \mathcal{L}_{\text{neg},A_v}(g)  +  \mathcal{L}_{\text{neg},B_v}(g) 
\end{align*}
where $\mathcal{L}_{\text{neg},A_v}(g)  := \mathbb{E}_{x,x^+, \{x^-_i\}_{\ell}} \chi \{x \in A_v\}  \log\bigg({ e^{\beta g(x)^\top g(x^+)}\!+\!\sum_{i=1}^\ell e^{\beta g(x)^\top g(x^-_{i})}  } \bigg) $ and $\mathcal{L}_{\text{neg},B_v}(g)  := \mathbb{E}_{x,x^+, \{x^-_i\}_{\ell}} \chi \{x \in B_v\}  \log\bigg({ e^{\beta g(x)^\top g(x^+)}\!+\!\sum_{i=1}^\ell e^{\beta g(x)^\top g(x^-_{i})}  } \bigg) $.
We need to upper bound $\mathcal{L}_{\text{neg}}(g') - \mathcal{L}_{\text{neg}}(g)$. 
% \begin{enumerate}
% \item In the event that $\{x\in A_v\}$, we have 
Using the notation above, we have
\begin{align*}
\mathcal{L}_{\text{neg},A_v}(g) 
&= \mathbb{E}_{x,x^+, \{x^-_i\}_{\ell}}  \chi \{x \in A_v\}  \log\bigg({ e^{\beta g(x)^\top g(x^+)}\!+\!n_{1,v}e^{\beta d}+\sum_{x_i^{-}\not\in {A}_v} e^{\beta g(x)^\top g(x^-_{i})}  } \bigg) \\
&= \mathbb{E}_{x,x^+, \{x^-_i\}_{\ell}}  \chi \{x \in A_v\}  \log\bigg({ e^{\beta g(x)^\top g(x^+)}+n_{1,v}e^{\beta d}+ \sum_{x_i^{-} \in B}e^{\beta g(x)^\top g(x^-_{i})} 
 +\sum_{x_i^{-}\not\in {A}_v\cup B} e^{\beta g(x)^\top g(x^-_{i})}  } \bigg) \\
\end{align*}
\begin{align*}
\mathcal{L}_{\text{neg},A_v}(g') & = \mathbb{E}_{x,x^+, \{x^-_i\}_{\ell}}  \chi \{x \in A_v\}  \log\bigg({ e^{\beta g'(x)^\top g'(x^+)}+ n_{1,v}e^{\beta d}+\sum_{x_i^{-}\not\in {A}_v} e^{\beta g'(x)^\top g'(x^-_{i})}  } \bigg) \nonumber \\
& =  \mathbb{E}_{x,x^+, \{x^-_i\}_{\ell}}  \chi \{x \in A_v\} \log\bigg({ e^{\beta g'(x)^\top g'(x^+)}+ n_{1,v}e^{\beta d}+ \sum_{x_i^{-}\in  B} e^{\beta g'(x)^\top g'(x^-_{i})}  +\sum_{x_i^{-}\not\in {A}_v\cup B} e^{\beta g(x)^\top g(x^-_{i})}  } \bigg) \nonumber \\
% &=\mathbb{E}_{x,x^+, \{x^-_i\}_{\ell}}  \chi \{x \in A_v\} \log\bigg({ e^{\beta g'(x)^\top g'(x^+)}+ (n_{1,v} + n_2)e^{\beta d}+\sum_{x_i^{-}\not\in {A}_v\cup B} e^{\beta g(x)^\top g(x^-_{i})}  } \bigg)
\end{align*}
\begin{align*}
\mathcal{L}_{\text{neg},B_v}(g) 
&= \mathbb{E}_{x,x^+, \{x^-_i\}_{\ell}}  \chi \{x \in B_v\}  \log\bigg({ e^{\beta g(x)^\top g(x^+)}\!+\!n_{3,v}e^{\beta d}+\sum_{x_i^{-}\not\in {B}_v} e^{\beta g(x)^\top g(x^-_{i})}  } \bigg) \\
&= \mathbb{E}_{x,x^+, \{x^-_i\}_{\ell}}  \chi \{x \in B_v\}  \log\bigg({ e^{\beta g(x)^\top g(x^+)}+n_{3,v}e^{\beta d}+ \sum_{x_i^{-} \in A}e^{\beta g(x)^\top g(x^-_{i})} 
 +\sum_{x_i^{-}\not\in {B}_v\cup A} e^{\beta g(x)^\top g(x^-_{i})}  } \bigg) \\
\end{align*}
\begin{align*}
\mathcal{L}_{\text{neg},B_v}(g') & = \mathbb{E}_{x,x^+, \{x^-_i\}_{\ell}}  \chi \{x \in B_v\}  \log\bigg({ e^{\beta g'(x)^\top g'(x^+)}+ n_{3,v}e^{\beta d}+\sum_{x_i^{-}\not\in {B}_v} e^{\beta g'(x)^\top g'(x^-_{i})}  } \bigg) \nonumber \\
& =  \mathbb{E}_{x,x^+, \{x^-_i\}_{\ell}}  \chi \{x \in B_v\} \log\bigg({ e^{\beta g'(x)^\top g'(x^+)}+ n_{3,v}e^{\beta d}+ \sum_{x_i^{-}\in  A} e^{\beta g'(x)^\top g'(x^-_{i})}  +\sum_{x_i^{-}\not\in {B}_v\cup A} e^{\beta g(x)^\top g(x^-_{i})}  } \bigg) \nonumber \\
% &=\mathbb{E}_{x,x^+, \{x^-_i\}_{\ell}}  \chi \{x \in A_v\} \log\bigg({ e^{\beta g'(x)^\top g'(x^+)}+ (n_{1,v} + n_2)e^{\beta d}+\sum_{x_i^{-}\not\in {A}_v\cup B} e^{\beta g(x)^\top g(x^-_{i})}  } \bigg)
\end{align*}

For each $v \in \mathcal{H}_d$, we write
\begin{align}
    &\mathcal{L}_{\text{neg},v}(g') - \mathcal{L}_{\text{neg},v}(g) \nonumber \\
    &=  \mathbb{E}_{x,x^+, \{x^-_i\}_{\ell}}  \chi \{x \in A_v\}\chi\{n_2=0\} \log\bigg({ e^{\beta g'(x)^\top g'(x^+)}+ n_{1,v}e^{\beta d}+ \sum_{x_i^{-}\in  B} e^{\beta g'(x)^\top g'(x^-_{i})}  +\sum_{x_i^{-}\not\in {A}_v\cup B} e^{\beta g(x)^\top g(x^-_{i})}  } \bigg) \nonumber \\
    &\quad \quad  - \mathbb{E}_{x,x^+, \{x^-_i\}_{\ell}}  \chi \{x \in A_v\} \chi\{n_2=0\} \log\bigg({ e^{\beta g(x)^\top g(x^+)}+n_{1,v}e^{\beta d}+ \sum_{x_i^{-} \in B}e^{\beta g(x)^\top g(x^-_{i})} 
 +\sum_{x_i^{-}\not\in {A}_v\cup B} e^{\beta g(x)^\top g(x^-_{i})}  } \bigg) \nonumber \\
 &\quad +  \mathbb{E}_{x,x^+, \{x^-_i\}_{\ell}}  \chi \{x \in A_v\}\chi\{n_2>0,n_{1,v}=0\} \nonumber \\
 &\quad\quad\quad \log\bigg({ e^{\beta g'(x)^\top g'(x^+)}+ n_{1,v}e^{\beta d}+ \sum_{x_i^{-}\in  B} e^{\beta g'(x)^\top g'(x^-_{i})}  +\sum_{x_i^{-}\not\in {A}_v\cup B} e^{\beta g(x)^\top g(x^-_{i})}  } \bigg) \nonumber \\
    &\quad \quad  - \mathbb{E}_{x,x^+, \{x^-_i\}_{\ell}}  \chi \{x \in A_v\} \chi\{n_2>0,n_{1,v}=0\} \nonumber \\
    &\quad \quad \quad \log\bigg({ e^{\beta g(x)^\top g(x^+)}+n_{1,v}e^{\beta d}+ \sum_{x_i^{-} \in B}e^{\beta g(x)^\top g(x^-_{i})} 
 +\sum_{x_i^{-}\not\in {A}_v\cup B} e^{\beta g(x)^\top g(x^-_{i})}  } \bigg) \nonumber \\
 &\quad \quad +  \mathbb{E}_{x,x^+, \{x^-_i\}_{\ell}}  \chi \{x \in A_v\}\chi\{n_2>0,n_{1,v}>0\} \nonumber \\
 &\quad\quad \quad  \log\bigg({ e^{\beta g'(x)^\top g'(x^+)}+ n_{1,v}e^{\beta d}+ \sum_{x_i^{-}\in  B} e^{\beta g'(x)^\top g'(x^-_{i})}  +\sum_{x_i^{-}\not\in {A}_v\cup B} e^{\beta g(x)^\top g(x^-_{i})}  } \bigg) \nonumber \\
    &\quad \quad - \mathbb{E}_{x,x^+, \{x^-_i\}_{\ell}}  \chi \{x \in A_v\} \chi\{n_2>0,n_{1,v}>0\} \nonumber \\
    &\quad \quad \quad  \log\bigg({ e^{\beta g(x)^\top g(x^+)}+n_{1,v}e^{\beta d}+ \sum_{x_i^{-} \in B}e^{\beta g(x)^\top g(x^-_{i})} 
 +\sum_{x_i^{-}\not\in {A}_v\cup B} e^{\beta g(x)^\top g(x^-_{i})}  } \bigg) \nonumber \\
 &\quad+  \mathbb{E}_{x,x^+, \{x^-_i\}_{\ell}}  \chi \{x \in B_v\}\chi\{n_4=0\} \log\bigg({ e^{\beta g'(x)^\top g'(x^+)}+ n_{3,v}e^{\beta d}+ \sum_{x_i^{-}\in  A} e^{\beta g'(x)^\top g'(x^-_{i})}  +\sum_{x_i^{-}\not\in {B}_v\cup A} e^{\beta g(x)^\top g(x^-_{i})}  } \bigg) \nonumber \\
    &\quad \quad  - \mathbb{E}_{x,x^+, \{x^-_i\}_{\ell}}  \chi \{x \in B_v\} \chi\{n_4=0\} \log\bigg({ e^{\beta g(x)^\top g(x^+)}+n_{3,v}e^{\beta d}+ \sum_{x_i^{-} \in A}e^{\beta g(x)^\top g(x^-_{i})} 
 +\sum_{x_i^{-}\not\in {B}_v\cup A} e^{\beta g(x)^\top g(x^-_{i})}  } \bigg) \nonumber \\
 &\quad +  \mathbb{E}_{x,x^+, \{x^-_i\}_{\ell}}  \chi \{x \in B_v\}\chi\{n_4>0,n_{3,v}=0\} \nonumber \\
 &\quad\quad\quad \log\bigg({ e^{\beta g'(x)^\top g'(x^+)}+ n_{3,v}e^{\beta d}+ \sum_{x_i^{-}\in  A} e^{\beta g'(x)^\top g'(x^-_{i})}  +\sum_{x_i^{-}\not\in {B}_v\cup A} e^{\beta g(x)^\top g(x^-_{i})}  } \bigg) \nonumber \\
    &\quad \quad  - \mathbb{E}_{x,x^+, \{x^-_i\}_{\ell}}  \chi \{x \in B_v\} \chi\{n_4>0,n_{3,v}=0\} \nonumber \\
    &\quad \quad \quad \log\bigg({ e^{\beta g(x)^\top g(x^+)}+n_{3,v}e^{\beta d}+ \sum_{x_i^{-} \in A}e^{\beta g(x)^\top g(x^-_{i})} 
 +\sum_{x_i^{-}\not\in {B}_v\cup A} e^{\beta g(x)^\top g(x^-_{i})}  } \bigg) \nonumber \\
 &\quad \quad +  \mathbb{E}_{x,x^+, \{x^-_i\}_{\ell}}  \chi \{x \in A_v\}\chi\{n_2>0,n_{1,v}>0\} \nonumber \\
 &\quad\quad \quad  \log\bigg({ e^{\beta g'(x)^\top g'(x^+)}+ n_{3,v}e^{\beta d}+ \sum_{x_i^{-}\in  A} e^{\beta g'(x)^\top g'(x^-_{i})}  +\sum_{x_i^{-}\not\in {B}_v\cup A} e^{\beta g(x)^\top g(x^-_{i})}  } \bigg) \nonumber \\
    &\quad \quad - \mathbb{E}_{x,x^+, \{x^-_i\}_{\ell}}  \chi \{x \in B_v\} \chi\{n_2>0,n_{1,v}>0\} \nonumber \\
    &\quad \quad \quad  \log\bigg({ e^{\beta g(x)^\top g(x^+)}+n_{3,v}e^{\beta d}+ \sum_{x_i^{-} \in A}e^{\beta g(x)^\top g(x^-_{i})} 
 +\sum_{x_i^{-}\not\in {B}_v\cup A} e^{\beta g(x)^\top g(x^-_{i})}  } \bigg) \nonumber
\end{align}
and consider each of the six differences individually, starting with the three differences involving $A_v$. 
\begin{enumerate}
\item $n_2 = 0$. 

% increases by at most $2\beta $ due to positive pair, and that increase happens with total probability $\Delta_f^{new}$ after summing over all $v$. So we need to lower bound the other terms in the log. The bad case is if $n_{1,v}$ is zero, but this happens with small probability. Use:
In this case we have
\begin{align}
    % \tilde{L}_{\text{neg}}(g') -\tilde{L}_{\text{neg}}(g) 
    &\mathbb{E}_{x,x^+, \{x^-_i\}_{\ell}}  \chi \{x \in A_v\}\chi \{n_2 = 0\}  \log\bigg({ e^{\beta g'(x)^\top g'(x^+)}+ n_{1,v}e^{\beta d}  +\sum_{x_i^{-}\not\in {A}_v\cup B} e^{\beta g(x)^\top g(x^-_{i})}  } \bigg) \nonumber \\
    &\quad - \mathbb{E}_{x,x^+, \{x^-_i\}_{\ell}}  \chi \{x \in A_v\}\chi \{n_2 = 0\}   \log\bigg({ e^{\beta g(x)^\top g(x^+)}+n_{1,v}e^{\beta d}
 +\sum_{x_i^{-}\not\in {A}_v\cup B} e^{\beta g(x)^\top g(x^-_{i})}  } \bigg)  \label{dif1} \\
 &= \mathbb{E}_{x,x^+, \{x^-_i\}_{\ell}}  \chi \{x \in A_v\} \chi \{n_2 = 0\} \log\bigg({ e^{\beta g'(x)^\top g'(x^+)}+ n_{1,v}e^{\beta d}   } \bigg) \nonumber \\
 &\quad - \mathbb{E}_{x,x^+, \{x^-_i\}_{\ell}}  \chi \{x \in A_v\} \chi \{n_2 = 0\}  \log\bigg({ e^{\beta g(x)^\top g(x^+)}+n_{1,v}e^{\beta d}  } \bigg)  \label{subm} \\
  &= \mathbb{E}_{x,x^+, \{x^-_i\}_{\ell}}  \chi \{x \in A_v\}  \chi \{x^+ \in B\} \chi \{n_2 = 0\}  \log\bigg({ e^{2\beta }e^{\beta g(x)^\top g(x^+)}+ n_{1,v}e^{\beta d}   } \bigg) \nonumber \\
 &\quad - \mathbb{E}_{x,x^+, \{x^-_i\}_{\ell}}  \chi \{x \in A_v\} \chi \{x^+ \in B\} \chi \{n_2 = 0\} \log\bigg({ e^{\beta g(x)^\top g(x^+)}+n_{1,v}e^{\beta d}  } \bigg)  \nonumber \\
 &\leq \mathbb{E}_{x,x^+, \{x^-_i\}_{\ell}}  \chi \{x \in A_v\}\chi \{x^+ \in B\} \chi \{n_2 = 0\}  \log\bigg({ e^{\beta d}+ n_{1,v}e^{\beta d}   } \bigg) \nonumber \\
 &\quad - \mathbb{E}_{x,x^+, \{x^-_i\}_{\ell}}  \chi \{x \in A_v\} \chi \{x^+ \in B\} \chi \{n_2 = 0\}  \log\bigg({ e^{\beta (d-2)}+n_{1,v}e^{\beta d}  } \bigg) \label{hh} \\
 &= \mathbb{E}_{x,x^+, \{x^-_i\}_{\ell}}  \chi \{x \in A_v\} \chi \{x^+ \in B\} \chi \{n_2 = 0\}  \log\bigg(\frac{1+ n_{1,v}   }{e^{-2\beta }+n_{1,v}} \bigg) \nonumber \\
 &=  \mathbb{E}_{x,x^+, \{x^-_i\}_{\ell}}  \chi \{x \in A_v\} \chi \{x^+ \in B\} \chi \{n_2 = 0\}  \chi\{ n_{1,v}=0 \} \log\bigg(\frac{1+ n_{1,v}   }{e^{-2\beta }+n_{1,v}} \bigg) \nonumber \\
 &\quad + \mathbb{E}_{x,x^+, \{x^-_i\}_{\ell}}  \chi \{x \in A_v\} \chi \{x^+ \in B\} \chi \{n_2 = 0\}  \chi\{ n_{1,v}>0 \} \log\bigg(\frac{1+ n_{1,v}   }{e^{-2\beta }+n_{1,v}} \bigg) \nonumber \\
 &\leq 2 \beta \mathbb{E}_{x,x^+, \{x^-_i\}_{\ell}}  \chi \{x \in A_v\} \chi \{x^+ \in B\} \chi \{n_2 = 0\}  \chi\{ n_{1,v}=0 \} \nonumber \\
 &\quad + \log(2 ) \mathbb{E}_{x,x^+, \{x^-_i\}_{\ell}}  \chi \{x \in A_v\} \chi \{x^+ \in B\} \chi \{n_2 = 0\}  \chi\{ n_{1,v}>0 \}  \nonumber 
\end{align}
where \eqref{subm} follows by the submodularity of $\log$ and the fact that $g'(x)^\top g'(x^+)\geq g(x)^\top g(x^+)$ by construction of $g'$, and \eqref{hh} follows since $h(x):= \frac{yx+ c}{x+c}$ is monotonically increasing for $y> 1$.
Next, by the independence of $x_i^-$ from $x$ and $x^+$, 
\begin{align}
    &\mathbb{E}_{x,x^+, \{x^-_i\}_{\ell}}   \chi \{x \in A_v\} \chi \{x^+ \in B\}\chi \{n_2 = 0\} \chi\{ n_{1,v}=0 \}  \nonumber \\
    &=  \mathbb{P}(x \in A_v \cap x^+ \in B) \mathbb{P}(n_{1,v}=0) \\
    &= \mathbb{P}(x \in A_v \cap x^+ \in B) (1 - \|A_v\| - \|B\|)^\ell \\
    & \mathbb{E}_{x,x^+, \{x^-_i\}_{\ell}}  \chi \{x \in A_v\}\chi \{x^+ \in B\} \chi \{n_2 = 0\}  \chi\{ n_{1,v}>0 \} \nonumber \\
    &= \mathbb{P}(x \in A_v \cap x^+ \in B) \mathbb{P}(n_{1,v}>0|n_2=0)\mathbb{P}(n_2=0) \\
     &\leq \mathbb{P}(x \in A_v \cap x^+ \in B) \min(1, \frac{\ell \|A_v\|}{1-\|B\|}) (1- \|B\|)^\ell
\end{align}
So in total, \eqref{dif1} is upper bounded by
\begin{align}
        \mathbb{P}(x \in A_v \cap x^+ \in B) \left( 2 \beta (1 - \|A_v\| - \|B\|)^\ell + \log(2) \min(1, \frac{\ell \|A_v\|}{1-\|B\|}) (1- \|B\|)^\ell\right).
\end{align}
% which is fine.


\item $n_{1,v} = 0, n_2 > 0$ 

% then $\tilde{L}_{\text{neg}}$ increases by at most $2\beta$ (since each term in the argument of the $\log$ can increase by no more than a multiplicative factor of $2\beta$). This happens with probability $(1-D_g(i))^l l\Vert B\Vert_\circ$, that is, there is a probability $(1-D_g(i))^l$ that no negative sample is sampled from the same cluster, and a probability $l\delta$ that $n_2 > 0$.  

In this case we have:
    \begin{align}
    % \tilde{L}_{\text{neg}}(g') -\tilde{L}_{\text{neg}}(g) 
    &\mathbb{E}_{x,x^+, \{x^-_i\}_{\ell}}  \chi \{x \in A_v,n_{1,v} = 0,n_2 > 0\} \nonumber \\
    &\quad \log\bigg({ e^{\beta g'(x)^\top g'(x^+)}+ n_{1,v}e^{\beta d} + \sum_{x_i^{-} \in B}e^{\beta g'(x)^\top g'(x^-_{i})}  +\sum_{x_i^{-}\not\in {A}_v\cup B} e^{\beta g(x)^\top g(x^-_{i})}  } \bigg) \nonumber \\
    &\quad - \mathbb{E}_{x,x^+, \{x^-_i\}_{\ell}}  \chi \{x \in A_v,n_{1,v} = 0,n_2 > 0\}   \nonumber \\
    &\quad \quad \log\bigg({ e^{\beta g(x)^\top g(x^+)}+n_{1,v}e^{\beta d}
+ \sum_{x_i^{-} \in B}e^{\beta g(x)^\top g(x^-_{i})}  +\sum_{x_i^{-}\not\in {A}_v\cup B} e^{\beta g(x)^\top g(x^-_{i})}  } \bigg)  \label{dif2} \\
 &=  \mathbb{E}_{x,x^+, \{x^-_i\}_{\ell}}  \chi \{x \in A_v,n_{1,v} = 0,n_2 > 0\}  \log\bigg({ e^{\beta g'(x)^\top g'(x^+)} + \sum_{x_i^{-} \in B}e^{\beta g'(x)^\top g'(x^-_{i})} +\sum_{x_i^{-}\not\in {A}_v\cup B} e^{\beta g(x)^\top g(x^-_{i})}  } \bigg) \nonumber \\
    &\quad - \mathbb{E}_{x,x^+, \{x^-_i\}_{\ell}}  \chi \{x \in A_v,n_{1,v} = 0,n_2 > 0\}   \log\bigg({ e^{\beta g(x)^\top g(x^+)}
 + \sum_{x_i^{-} \in B}e^{\beta g(x)^\top g(x^-_{i})} +\sum_{x_i^{-}\not\in {A}_v\cup B} e^{\beta g(x)^\top g(x^-_{i})}  } \bigg)  \\
  &\leq  \mathbb{E}_{x,x^+, \{x^-_i\}_{\ell}}  \chi \{x \in A_v,n_{1,v} = 0,n_2 > 0\}  \log\bigg({ e^{\beta g'(x)^\top g'(x^+)} + \sum_{x_i^{-} \in B}e^{\beta g'(x)^\top g'(x^-_{i})} } \bigg) \nonumber \\
    &\quad - \mathbb{E}_{x,x^+, \{x^-_i\}_{\ell}}  \chi \{x \in A_v,n_{1,v} = 0,n_2 > 0\}   \log\bigg({ e^{\beta g(x)^\top g(x^+)}
 + \sum_{x_i^{-} \in B}e^{\beta g(x)^\top g(x^-_{i})}  } \bigg)  \\
 &\leq 2 \beta  \mathbb{P}(x \in A_v) \mathbb{E}_{ \{x^-_i\}_{\ell}}  [\chi \{n_{1,v} = 0\}\chi \{n_2 > 0\}] \nonumber \\
 &= 2 \beta  \mathbb{P}(x \in A_v) \mathbb{E}_{ \{x^-_i\}_{\ell}} [ \chi \{\cap_i x_{i}^- \notin A_v\}\chi \{\cup_i x_{i}^- \in B\} ] \nonumber \\
 &=  2 \beta \mathbb{P}(x \in A_v) \mathbb{P} ( \cup_i x_{i}^- \in B | \cap_i x_{i}^- \notin A_v)\mathbb{P}(\cap_i x_{i}^- \notin A_v) \nonumber \\
 &\leq 2 \beta  \mathbb{P}(x \in A_v) \mathbb{P}(\cap_i x_{i}^- \notin A_v) \min\left( 1, \sum_i \mathbb{P} ( x_{i}^- \in B |  x_{i}^- \notin A_v) \right) \nonumber \\
 &= 2 \beta  \|A_v\|_\circ (1 - \|A_v\|)^\ell \min\left(1, \frac{\ell \|B\|}{1- \|A_v\|}\right) \nonumber 
 % &= 2 \beta \ell  \log(\ell+1)  \|B\| \|A_v\|_\circ (1 - \|A_v\|)^{\ell-1} .
\end{align}
% where \eqref{}

\item $n_1, n_2 > 0$.
% We denote the conditional expectation under this case using the notation $\E\left[\cdot | \circled{1c}\right]$. Then $\tilde{L}_{\text{neg}}$ increases by at most 
% \begin{align*}
% &\mathbb{E}_{x,x^+, \{x^-_i\}_{\ell}} \log\bigg({ e^{\beta g(x)^\top g(x^+)}\!+\!(n_1+n_2)e^{\beta d}+\sum_{i\not\in A\cup B} e^{\beta g(x)^\top g(x^-_{i})}  } \bigg) \\
% &\quad\quad- \log\bigg({ e^{\beta g(x)^\top g(x^+)}\!+\!n_1e^{\beta d}+\sum_{i\not\in A} e^{\beta g(x)^\top g(x^-_{i})}  } \bigg)|\circled{1c}\\
% &\leq \mathbb{E}_{x,x^+, \{x^-_i\}_{\ell}} \log\bigg({ e^{\beta g(x)^\top g(x^+)}\!+\!(n_1+n_2)e^{\beta d}+\sum_{i\not\in A\cup B} e^{\beta g(x)^\top g(x^-_{i})}  } \bigg) \\
% &\quad\quad- \log\bigg({ e^{\beta g(x)^\top g(x^+)}\!+\!n_1e^{\beta d}+\sum_{i\not\in A\cup B} e^{\beta g(x)^\top g(x^-_{i})}  } \bigg)|\circled{1c}\\
% &\quad\le  \mathbb{E}_{x,x^+, \{x^-_i\}_{\ell}} \left[\log\bigg((n_1+n_2)e^{\beta d} \bigg) - \mathbb{E}_{x,x^+, \{x^-_i\}_{\ell}} \log\bigg( n_1e^{\beta d}\bigg)\mid \circled{1c}\right]\\
% &\quad\le \E_{x, x^+, \{x^-_i\}_l}\left[\log\left(1+\frac{n_2}{n_1}\right)\mid \circled{1c}\right]\\
% &=\quad\sum_{n_1, n_2\ne 0, n_3} \binom{l}{n_1~n_2~n_3} \Vert A\Vert_\circ^{n_1}\Vert B\Vert_\circ^{n_2}\Vert 1-A-B\Vert_\circ^{n_3}\log\left(1+\frac{n_2}{n_1}\right)\\
% &\le\sum_{n_1\ne 0, n_2\ne 0, n_3} \binom{l}{n_1~n_2~n_3} \Vert A\Vert_\circ^{n_1}\Vert B\Vert_\circ^{n_2}\Vert 1-A-B\Vert_\circ^{n_3}\frac{2n_2}{n_1+1}\\
% &\le 2\frac{\Vert B\Vert_\circ}{\Vert A\Vert_\circ}\sum_{n_1, n_2, n_3} \binom{l}{n_1+1~n_2-1~n_3} \Vert A\Vert_\circ^{n_1+1}\Vert B\Vert_\circ^{n_2-1}\Vert 1-A-B\Vert_\circ^{n_3}\le  2\frac{\Vert B\Vert_\circ}{\Vert A\Vert_\circ}
% \end{align*}


% \end{enumerate}


We have
\begin{align}
&\mathbb{E}  \bigg[\chi \{x \in A_v,n_{1,v} > 0,n_2 > 0\} \nonumber \\
&\quad \quad \quad \log\bigg({ e^{\beta g'(x)^\top g'(x^+)}+ n_{1,v}e^{\beta d} + \sum_{x_i^{-} \in B}e^{\beta g'(x)^\top g'(x^-_{i})}  +\sum_{x_i^{-}\not\in {A}_v\cup B} e^{\beta g(x)^\top g(x^-_{i})}  } \bigg) \bigg]\nonumber \\
    &\quad - \mathbb{E} \bigg[\chi \{x \in A_v,n_{1,v} > 0,n_2 > 0\} \nonumber \\
    &\quad \quad\quad \log\bigg({ e^{\beta g(x)^\top g(x^+)}+n_{1,v}e^{\beta d}
+ \sum_{x_i^{-} \in B}e^{\beta g(x)^\top g(x^-_{i})}  +\sum_{x_i^{-}\not\in {A}_v\cup B} e^{\beta g(x)^\top g(x^-_{i})}  } \bigg) \bigg] \label{dif3} \\
&\leq \mathbb{E}  \left[\chi \{x \in A_v,n_{1,v} > 0,n_2 > 0\}  \log\bigg({ e^{\beta g'(x)^\top g'(x^+)}+ n_{1,v}e^{\beta d} + \sum_{x_i^{-} \in B}e^{\beta g'(x)^\top g'(x^-_{i})}   } \bigg) \right]\nonumber \\
    &\quad - \mathbb{E} \left[\chi \{x \in A_v,n_{1,v} > 0,n_2 > 0\}   \log\bigg({ e^{\beta g(x)^\top g(x^+)}+n_{1,v}e^{\beta d}
+ \sum_{x_i^{-} \in B}e^{\beta g(x)^\top g(x^-_{i})}    } \bigg) \right] \\
&\leq \mathbb{E}  \left[\chi \{x \in A_v,n_{1,v} > 0,n_2 > 0\}  \log\bigg({ e^{\beta g'(x)^\top g'(x^+)}+ (n_{1,v}+n_2)e^{\beta d}  } \bigg) \right]\nonumber \\
    &\quad - \mathbb{E} \left[\chi \{x \in A_v,n_{1,v} > 0,n_2 > 0\}   \log\bigg({ e^{\beta g(x)^\top g(x^+)}+n_{1,v}e^{\beta d} + n_2e^{\beta (d-2)}
  } \bigg) \right] \\
  &= \mathbb{E}  \left[\chi \{x \in A_v,n_{1,v} > 0,n_2 > 0,  g'(x)^\top g'(x^+) =  g(x)^\top g(x^+) \}  \log\bigg({ e^{\beta g'(x)^\top g'(x^+)}+ (n_{1,v}+n_2)e^{\beta d}  } \bigg) \right]\nonumber \\
    &\quad - \mathbb{E} \left[\chi \{x \in A_v,n_{1,v} > 0,n_2 > 0,  g'(x)^\top g'(x^+) =  g(x)^\top g(x^+)\} \nonumber \\
    &\quad \quad \log\bigg({ e^{\beta g(x)^\top g(x^+)}+n_{1,v}e^{\beta d} + n_2e^{\beta (d-2)}
  } \bigg) \right] \\
  &\quad +  \mathbb{E}  \left[\chi \{x \in A_v,n_{1,v} > 0,n_2 > 0,  g'(x)^\top g'(x^+) \neq  g(x)^\top g(x^+) \} \nonumber \\
  &\quad \quad \log\bigg({ e^{\beta g'(x)^\top g'(x^+)}+ (n_{1,v}+n_2)e^{\beta d}  } \bigg) \right]\nonumber \\
    &\quad - \mathbb{E} \left[\chi \{x \in A_v,n_{1,v} > 0,n_2 > 0,  g'(x)^\top g'(x^+) \neq   g(x)^\top g(x^+)\}  \nonumber \\
    &\quad \quad \log\bigg({ e^{\beta g(x)^\top g(x^+)}+n_{1,v}e^{\beta d} + n_2e^{\beta (d-2)}
  } \bigg) \right] 
  \end{align}
  Denote by $(*)$ the expression in \eqref{dif3}. Continuing from above, we have
  \begin{align}
  (*) &\leq \mathbb{E}  \left[\chi \{x \in A_v,n_{1,v} > 0,n_2 > 0,  g'(x)^\top g'(x^+) =  g(x)^\top g(x^+) \}  \log\bigg({  \frac{n_{1,v}+n_2}{n_{1,v}} } \bigg) \right]\nonumber \\
    % &\quad - \mathbb{E} \left[\chi \{x \in A_v,n_{1,v} > 0,n_2 > 0,  g'(x)^\top g'(x^+) =  g(x)^\top g(x^+)\}   \log\bigg({ n_{1,v}e^{\beta d} + n_2e^{\beta (d-2)}
  % } \bigg) \right] \\
  &\quad +  \mathbb{E}  \left[\chi \{x \in A_v,n_{1,v} > 0,n_2 > 0,  g'(x)^\top g'(x^+) \neq  g(x)^\top g(x^+) \}  \log\bigg(\frac{  n_{1,v}+n_2+1  }{n_{1,v} } \bigg) \right]\nonumber \\
  &\leq  \mathbb{E}  \left[\chi \{x \in A_v,n_{1,v} > 0,n_2 > 0,  g'(x)^\top g'(x^+) =  g(x)^\top g(x^+) \}  \frac{2n_2}{n_{1,v}+1} \right]\nonumber \\
    % &\quad - \mathbb{E} \left[\chi \{x \in A_v,n_{1,v} > 0,n_2 > 0,  g'(x)^\top g'(x^+) =  g(x)^\top g(x^+)\}   \log\bigg({ n_{1,v}e^{\beta d} + n_2e^{\beta (d-2)}
  % } \bigg) \right] \\
  &\quad +  \mathbb{E}  \left[\chi \{x \in A_v,n_{1,v} > 0,n_2 > 0,  g'(x)^\top g'(x^+) \neq  g(x)^\top g(x^+) \}  \frac{  2n_2+2  }{n_{1,v}+1 } \right]\nonumber \\
  &= \mathbb{E}  \left[\chi \{x \in A_v,n_{1,v} > 0,n_2 > 0\}  \frac{2n_2}{n_{1,v}+1}  \right]\nonumber \\
    % &\quad - \mathbb{E} \left[\chi \{x \in A_v,n_{1,v} > 0,n_2 > 0,  g'(x)^\top g'(x^+) =  g(x)^\top g(x^+)\}   \log\bigg({ n_{1,v}e^{\beta d} + n_2e^{\beta (d-2)}
  % } \bigg) \right] \\
  &\quad +  \mathbb{E}  \left[\chi \{x \in A_v,n_{1,v} > 0,n_2 > 0,  g'(x)^\top g'(x^+) \neq  g(x)^\top g(x^+) \}  \frac{  2  }{n_{1,v}+1 } \right]\nonumber \\
  &= \mathbb{E}  \left[\chi \{x \in A_v,n_{1,v} > 0,n_2 > 0\}  \frac{2n_2}{n_{1,v}+1}  \right]\nonumber \\
  % &\quad + \mathbb{E}  \left[\chi \{x \in A_v,n_{1,v} > 0,n_2 > 0, A_v\cap B\neq \emptyset \}  \frac{2n_2}{n_{1,v}+1}  \right]\nonumber \\
  &\quad +  \mathbb{E}  \left[\chi \{x \in A_v,n_{1,v} > 0,n_2 > 0,  g'(x)^\top g'(x^+) \neq  g(x)^\top g(x^+) \}  \frac{  2  }{n_{1,v}+1 } \right]\label{4terms}
  % &\quad +  \mathbb{E}  \left[\chi \{x \in A_v,n_{1,v} > 0,n_2 > 0,  g'(x)^\top g'(x^+) \neq  g(x)^\top g(x^+), A_v\cap B\neq \emptyset \}  \frac{  2  }{n_{1,v}+1 } \right]\label{4terms}
\end{align}
where the second inequality follows using the inequality $\log(1+x)\leq x$. 
Thus we are left with two terms in \eqref{4terms}.
For the first term  we have (there is notation overload: after the first line, $n_{1,v}$ and $n_2$ change from random variables to dummy variables):
% For the first term ,
\begin{align}
    &\mathbb{E}  \left[\chi \{x \in A_v,n_{1,v} > 0,n_2 > 0,A_v\cap B= \emptyset \}  \frac{2n_2}{n_{1,v}+1} \right] \nonumber \\
    &= \mathbb{P}(x \in A_v) \sum_{n_{1,v},n_2: n_{1,v}+n_2\leq \ell }  \chi \{n_{1,v} > 0,n_2 > 0\} \binom{l}{n_{1,v}~n_2~1\!-\!n_{1,v}\!-\!n_2} \nonumber \\
    &\quad \quad \quad \quad  \Vert A_v\Vert^{n_{1,v}}\Vert B\Vert^{n_2}\Vert 1-A_v-B\Vert^{1-n_{1,v}-n_2}\frac{2n_2}{n_{1,v}+1} \\
    &= 2\mathbb{P}(x \in A_v)\sum_{n_{1,v},n_2: n_{1,v},n_2>0, n_{1,v}+n_2\leq \ell}  \binom{l}{n_{1,v}~n_2~1\!-\!n_{1,v}\!-\!n_2} \nonumber \\
    &\quad \quad \quad \quad \Vert A_v\Vert^{n_{1,v}}\Vert B\Vert^{n_2}\Vert 1-A_v-B\Vert^{1-n_{1,v}-n_2}\frac{n_2}{n_{1,v}+1} \\
    &= 2 D_g(v) \frac{\|B\|}{\|A_v\|} \sum_{n_{1,v},n_2: n_{1,v},n_2>0, n_{1,v}+n_2\leq \ell}    \binom{l}{n_{1,v}+1~n_2-1~1\!-\!n_{1,v}\!-\!n_2} \nonumber \\
    &\quad \quad \quad \quad \Vert A_v\Vert^{n_{1,v}+1}\Vert B\Vert^{n_2-1}\Vert 1-A_v-B\Vert^{1- n_{1,v}-n_2} \\
    &\leq 2 D_g(v) \frac{\|B\|}{\|A_v\|} \!\sum_{n_{1,v}\!+\!1,n_2\!-\!1: n_{1,v}\!+\!1,n_2-\!1\!\geq\!0, n_{1,v}+1\!+\!n_2-1\!\leq\! \ell}   \binom{l}{n_{1,v}\!+\!1~n_2\!-\!1~1\!-(n_{1,v}\!+\!1) \!-\! (n_2\!-\!1)}\nonumber \\
    &\quad \quad \quad \quad \quad \quad \quad \quad \quad \quad \quad\quad \quad \quad \quad  \quad \quad \quad \quad  \quad \quad \quad \Vert A_v\Vert^{n_{1,v}\!+\!1}\Vert B\Vert^{n_2\!-\!1}\Vert 1\!-\!A_v\!-\!B\Vert^{1 \!-\! (n_{1,v}\!+\!1)\! -\! (n_2\!-\!1)}  \label{sq}\\
    &= 2{\|B\|} ( \Vert A_v\Vert + \Vert B\Vert + \Vert 1-A_v-B\Vert)^\ell  \nonumber \\
    &= {2 {\|B\|}}   \nonumber 
\end{align}
where in \eqref{sq} we have added terms to the sum to complete the trinomial expansion, and the last equality follows since $A_v$ and $B$ are disjoint.

Now we need to consider the last term in \eqref{4terms}, which correspond to the case wherein the positive inner products are not equal for $g$ and $g'$. For this term, we simply have
{\begin{align}
&\mathbb{E}  \left[\chi \{x \in A_v,n_{1,v} > 0,n_2 > 0,  g'(x)^\top g'(x^+) \neq  g(x)^\top g(x^+)\}  \frac{  2  }{n_{1,v}+1 } \right]\nonumber \\
  &\leq \mathbb{P}  \left[x \in A_v, x^+\in B\right]
\end{align}
}

In total, for the case $n_{1,v}>0,n_2>0$ and $x\in A_v$, we have
\begin{align}
    &\mathbb{E}  \bigg[\chi \{x \in A_v,n_{1,v} > 0,n_2 > 0\} \nonumber \\
    &\quad \quad \bigg( \log\bigg({ e^{\beta g'(x)^\top g'(x^+)}+ n_{1,v}e^{\beta d} + \sum_{x_i^{-} \in B}e^{\beta g'(x)^\top g'(x^-_{i})}  +\sum_{x_i^{-}\not\in {A}_v\cup B} e^{\beta g(x)^\top g(x^-_{i})}  } \bigg) \nonumber \\
    &\quad \quad - \log\bigg({ e^{\beta g(x)^\top g(x^+)}+n_{1,v}e^{\beta d}
+ \sum_{x_i^{-} \in B}e^{\beta g(x)^\top g(x^-_{i})}  +\sum_{x_i^{-}\not\in {A}_v\cup B} e^{\beta g(x)^\top g(x^-_{i})}  } \bigg)\bigg) \bigg] \nonumber \\
&\leq  2 \|B\| +   \mathbb{P}  \left[x \in A_v, x^+\in B\right]
% 2 \|B\|_\circ \chi\{ A_v\cap B = \emptyset \} + 2 \chi\{\|A_v\!\setminus\! B\|_\circ \geq \|A_v\|_\circ/2\}({\Vert A_v\cap B\Vert_\circ+ 2\Vert B\setminus A_v\Vert_\circ }) \nonumber \\
%     &\quad +  4 \chi\{\|A_v\!\setminus\! B\|_\circ \geq \|A_v\|_\circ/2\}\frac{\Vert A_v\cap B\Vert_\circ^2 + 2 \Vert A_v\cap B\Vert_\circ\Vert B\setminus A_v\Vert_\circ}{\Vert A_v\Vert_\circ} \nonumber \\
%     &\quad + 8 \ell \Vert  A_v\cap B\Vert_\circ {\Vert B\setminus A_v\Vert_\circ}  (1 - \Vert  A_v\Vert_\circ/2)^{\ell} \chi \{ \|A_v\!\cap\! B\|_\circ \geq \|A_v\|_\circ/2\} \nonumber \\
%     &\quad +4 \|A_v\cap B\|_\circ \left(2\frac{\Vert B\setminus A_v\Vert_\circ}{\Vert A_v\Vert_\circ}+1\right)\chi \{\|A_v\!\cap\! B\|_\circ \geq \|A_v\|_\circ/2\} \nonumber \\
%     &\quad + \chi\{A_v\cap B= \emptyset \} \mathbb{P}  \left[x \in A_v, x^+\in B\right] + \chi\{A_v\cap B\neq \emptyset \} \mathbb{P}  \left[x \in A_v \cap B, x^+ \notin B \right] 
\end{align}
% All of these terms are $O(\|B\|_\circ)$ and do not depend on $\beta$ so we can make $\beta$ large enough to dominate them.

\item $n_4 = 0$.

We argue similarly as in Case 1.
\begin{align}
   ((4))&:=   \mathbb{E}_{x,x^+, \{x^-_i\}_{\ell}}  \chi \{x \in B_v\}\chi\{n_4=0\} \nonumber \\
   &\quad \log\bigg({ e^{\beta g'(x)^\top g'(x^+)}+ n_{3,v}e^{\beta d}+ \sum_{x_i^{-}\in  A} e^{\beta g'(x)^\top g'(x^-_{i})}  +\sum_{x_i^{-}\not\in {B}_v\cup A} e^{\beta g(x)^\top g(x^-_{i})}  } \bigg) \nonumber \\
    &\quad  - \mathbb{E}_{x,x^+, \{x^-_i\}_{\ell}}  \chi \{x \in B_v\} \chi\{n_4=0\} \nonumber \\
    &\quad \quad \log\bigg({ e^{\beta g(x)^\top g(x^+)}+n_{3,v}e^{\beta d}+ \sum_{x_i^{-} \in A}e^{\beta g(x)^\top g(x^-_{i})} 
 +\sum_{x_i^{-}\not\in {B}_v\cup A} e^{\beta g(x)^\top g(x^-_{i})}  } \bigg) \nonumber \\
    &= \mathbb{E}_{x,x^+, \{x^-_i\}_{\ell}}  \chi \{x \in B_v\}\chi\{n_4=0\} \log\bigg({ e^{\beta g'(x)^\top g'(x^+)}+ n_{3,v}e^{\beta d} +\sum_{x_i^{-}\not\in {B}_v\cup A} e^{\beta g(x)^\top g(x^-_{i})}  } \bigg) \nonumber \\
    &\quad \quad  - \mathbb{E}_{x,x^+, \{x^-_i\}_{\ell}}  \chi \{x \in B_v\} \chi\{n_4=0\} \log\bigg({ e^{\beta g(x)^\top g(x^+)}+n_{3,v}e^{\beta d}+\sum_{x_i^{-}\not\in {B}_v\cup A} e^{\beta g(x)^\top g(x^-_{i})}  } \bigg) \nonumber \\
    &\leq \mathbb{E}_{x,x^+, \{x^-_i\}_{\ell}}  \chi \{x \in B_v\}\chi\{n_4=0\} \log\bigg({ e^{\beta g'(x)^\top g'(x^+)}+ n_{3,v}e^{\beta d}   } \bigg) \nonumber \\
    &\quad \quad  - \mathbb{E}_{x,x^+, \{x^-_i\}_{\ell}}  \chi \{x \in B_v\} \chi\{n_4=0\} \log\bigg( e^{\beta g(x)^\top g(x^+)}+n_{3,v}e^{\beta d} \bigg) \label{bb}
\end{align}
where \eqref{bb} follows since $ {g'(x)^\top g'(x^+)} \geq { g(x)^\top g(x^+)}$. Next we split on $x^+\in A$, obtaining
\begin{align}
    ((4)) &\leq  \mathbb{E}_{x,x^+, \{x^-_i\}_{\ell}}  \chi \{x \in B_v, n_4=0, x^+ \in A\} \log\bigg({ e^{\beta g'(x)^\top g'(x^+)}+ n_{3,v}e^{\beta d}   } \bigg) \nonumber \\
    &\quad \quad  - \mathbb{E}_{x,x^+, \{x^-_i\}_{\ell}}  \chi \{x \in B_v,n_4=0, x^+\in A\} \log\bigg( e^{\beta g(x)^\top g(x^+)}+n_{3,v}e^{\beta d} \bigg) \nonumber \\
    &\quad +  \mathbb{E}_{x,x^+, \{x^-_i\}_{\ell}}  \chi \{x \in B_v, n_4=0, x^+ \notin A\} \log\bigg({ e^{\beta g'(x)^\top g'(x^+)}+ n_{3,v}e^{\beta d}   } \bigg) \nonumber \\
    &\quad \quad  - \mathbb{E}_{x,x^+, \{x^-_i\}_{\ell}}  \chi \{x \in B_v,n_4=0, x^+\notin A\} \log\bigg( e^{\beta g(x)^\top g(x^+)}+n_{3,v}e^{\beta d} \bigg) \nonumber \\
    &= \mathbb{E}_{x,x^+, \{x^-_i\}_{\ell}}  \chi \{x \in B_v, n_4=0, x^+ \in A\} \log\bigg({ e^{2 \beta} e^{\beta g(x)^\top g(x^+)}+ n_{3,v}e^{\beta d}   } \bigg) \nonumber \\
    &\quad \quad  - \mathbb{E}_{x,x^+, \{x^-_i\}_{\ell}}  \chi \{x \in B_v,n_4=0, x^+\in A\} \log\bigg( e^{\beta g(x)^\top g(x^+)}+n_{3,v}e^{\beta d} \bigg) \nonumber \\
    &\leq \mathbb{E}_{x,x^+, \{x^-_i\}_{\ell}}  \chi \{x \in B_v, n_4=0, x^+ \in A\} \log\bigg({ e^{\beta d} + n_{3,v}e^{\beta d}   } \bigg) \nonumber \\
    &\quad \quad  - \mathbb{E}_{x,x^+, \{x^-_i\}_{\ell}}  \chi \{x \in B_v,n_4=0, x^+\in A\} \log\bigg( e^{\beta (d-2)}+n_{3,v}e^{\beta d} \bigg)  \nonumber \\
    &= \mathbb{E}_{x,x^+, \{x^-_i\}_{\ell}}  \chi \{x \in B_v, n_4=0, x^+ \in A\} \log\bigg(\frac{ 1 + n_{3,v}  }{e^{-2\beta} + n_{3,v}} \bigg) \nonumber \\
    &\leq 2\beta \mathbb{E}_{x,x^+, \{x^-_i\}_{\ell}}  \chi \{x \in B_v, n_4=0, x^+ \in A, n_{3,v}=0\}  \nonumber \\
    &+ \log( 2) \mathbb{E}_{x,x^+, \{x^-_i\}_{\ell}}  \chi \{x \in B_v,n_4=0, x^+\in A,n_{3,v}>0\} 
\end{align}
where
\begin{align}
    &\mathbb{E}_{x,x^+, \{x^-_i\}_{\ell}}  \chi \{x \in B_v, n_4=0, x^+ \in A, n_{3,v}=0\}  \nonumber \\
    &=  \mathbb{P}(x \in B_v \cap x^+ \in A) \mathbb{P}(n_{3,v}=0, n_4=0) \\
    &= \mathbb{P}(x \in B_v \cap x^+ \in A) (1 - \|B_v\| - \|A\|)^\ell 
    % \\
    % & \mathbb{E}_{x,x^+, \{x^-_i\}_{\ell}}  \chi \{x \in A_v\}\chi \{x^+ \in B\} \chi \{n_2 = 0\}  \chi\{ n_{1,v}>0 \} 
    % \nonumber \\
    % &= \mathbb{P}(x \in A_v \cap x^+ \in B) \mathbb{P}(n_{3,v}>0) \\
    %  &\leq \mathbb{P}(x \in A_v \cap x^+ \in B) D_g(v)
\end{align}
\begin{align}
    &\mathbb{E}_{x,x^+, \{x^-_i\}_{\ell}}  \chi \{x \in B_v,n_4=0, x^+\in A,n_{3,v}>0\} \nonumber \\
    &= \mathbb{P}(x \in B_v \cap x^+ \in A)  \mathbb{P}(n_{3,v} >0, n_4=0)  \nonumber \\
    &\leq \mathbb{P}(x \in B_v \cap x^+ \in A) \min( 1, \frac{\ell \|B_v\|}{1 - \|A\|})  (1 - \|A\|)^\ell
\end{align}
so in total for this case we have 
\begin{align}
    ((4)) &\leq \mathbb{P}(x \in B_v \cap x^+ \in A)\left(2\beta (1 - \|B_v\| - \|A\|)^\ell  + \log(2)\min( 1, \frac{\ell \|B_v\|}{1 - \|A\|})  (1 - \|A\|)^\ell\right)
\end{align}



\item $n_4>0, n_{3,v} = 0$.

Define $C := \{x: f_1'(x) = f_1(x), f_1'(x)\neq f_1'(B) \}\subseteq A$. Let $n_{5}:= \sum_{i=1}^\ell \chi\{ x_{i}^- \in A\setminus C\}$, $n_{6}:= \sum_{i=1}^\ell \chi\{ x_{i}^- \in C\}$. 

We have 
\begin{align}
    ((5)) &=  \mathbb{E}_{x,x^+, \{x^-_i\}_{\ell}}  \chi \{x \in B_v,n_4>0,n_{3,v}=0\}\nonumber \\
    &\quad \log\bigg({ e^{\beta g'(x)^\top g'(x^+)}+ n_{3,v}e^{\beta d}+ \sum_{x_i^{-}\in  A} e^{\beta g'(x)^\top g'(x^-_{i})}  +\sum_{x_i^{-}\not\in {B}_v\cup A} e^{\beta g(x)^\top g(x^-_{i})}  } \bigg) \nonumber \\
    &\quad  - \mathbb{E}_{x,x^+, \{x^-_i\}_{\ell}}  \chi \{x \in B_v,n_4>0,n_{3,v}=0\} \nonumber \\
    &\quad \quad \log\bigg({ e^{\beta g(x)^\top g(x^+)}+n_{3,v}e^{\beta d}+ \sum_{x_i^{-} \in A}e^{\beta g(x)^\top g(x^-_{i})} 
 +\sum_{x_i^{-}\not\in {B}_v\cup A} e^{\beta g(x)^\top g(x^-_{i})}  } \bigg) \nonumber \\
 &= \mathbb{E}_{x,x^+, \{x^-_i\}_{\ell}}  \chi \{x \in B_v,n_4>0,n_{3,v}=0\}\nonumber \\
 &\quad \log\bigg({ e^{\beta g'(x)^\top g'(x^+)}+  e^{2\beta }\sum_{x_i^{-} \in A\setminus C}e^{\beta g(x)^\top g(x^-_{i})} +e^{-2\beta }\sum_{x_i^{-} \in  C}e^{\beta g(x)^\top g(x^-_{i})} +\sum_{x_i^{-}\not\in {B}_v\cup A} e^{\beta g(x)^\top g(x^-_{i})}  } \bigg) \nonumber \\
    &\quad \quad  - \mathbb{E}_{x,x^+, \{x^-_i\}_{\ell}}  \chi \{x \in B_v,n_4>0,n_{3,v}=0\} \nonumber \\
    &\quad \log\bigg({ e^{\beta g(x)^\top g(x^+)}+\sum_{x_i^{-} \in A\setminus C}e^{\beta g(x)^\top g(x^-_{i})} +\sum_{x_i^{-} \in  C}e^{\beta g(x)^\top g(x^-_{i})} 
 +\sum_{x_i^{-}\not\in {B}_v\cup A} e^{\beta g(x)^\top g(x^-_{i})}  } \bigg) \nonumber \\
 &\leq \mathbb{E}_{x,x^+, \{x^-_i\}_{\ell}}  \chi \{x \in B_v,n_4>0,n_{3,v}=0\}\nonumber \\
 &\quad \log\bigg({ e^{\beta g'(x)^\top g'(x^+)}+  n_{5}e^{\beta d }+ n_{6}e^{-\beta d } +\sum_{x_i^{-}\not\in {B}_v\cup A} e^{\beta g(x)^\top g(x^-_{i})}  } \bigg) \nonumber \\
    &\quad \quad  - \mathbb{E}_{x,x^+, \{x^-_i\}_{\ell}}  \chi \{x \in B_v,n_4>0,n_{3,v}=0\} \nonumber \\
    &\quad \log\bigg({ e^{\beta g(x)^\top g(x^+)}+n_5 e^{\beta(d-2)} +n_6 e^{-\beta(d-2)}
 +\sum_{x_i^{-}\not\in {B}_v\cup A} e^{\beta g(x)^\top g(x^-_{i})}  } \bigg) \nonumber \\
  &\leq   \mathbb{E}_{x,x^+, \{x^-_i\}_{\ell}}  \chi \{x \in B_v,n_4>0,n_{3,v}=0, x^+ \in A\}\nonumber \\
 &\quad \quad \bigg(\log\bigg({  (n_{5}+1)e^{\beta d }+ n_{6}e^{-\beta d } +\sum_{x_i^{-}\not\in {B}_v\cup A} e^{\beta g(x)^\top g(x^-_{i})}  } \bigg) \nonumber \\
    % &\quad \quad  - \mathbb{E}_{x,x^+, \{x^-_i\}_{\ell}}  \chi \{x \in B_v,n_4>0,n_{3,v}=0, x^+ \in A\} \nonumber \\
    &\quad\quad \quad - \log\bigg({  (n_5+1) e^{\beta(d-2)} +n_6 e^{-\beta(d-2)}
 +\sum_{x_i^{-}\not\in {B}_v\cup A} e^{\beta g(x)^\top g(x^-_{i})}  } \bigg)\bigg) \nonumber \\
 &\quad + \mathbb{E}_{x,x^+, \{x^-_i\}_{\ell}}  \chi \{x \in B_v,n_4>0,n_{3,v}=0, x^+ \notin A\}\nonumber \\
 &\quad \quad \bigg( \log\bigg({  n_{5}e^{\beta d }+ (n_{6}+1)e^{-\beta d } +\sum_{x_i^{-}\not\in {B}_v\cup A} e^{\beta g(x)^\top g(x^-_{i})}  } \bigg) \nonumber \\
    % &\quad \quad  - \mathbb{E}_{x,x^+, \{x^-_i\}_{\ell}}  \chi \{x \in B_v,n_4>0,n_{3,v}=0, x^+ \notin A\} \nonumber \\
    &\quad \quad \quad - \log\bigg({  n_5 e^{\beta(d-2)} +(n_6+1) e^{-\beta(d-2)}
 +\sum_{x_i^{-}\not\in {B}_v\cup A} e^{\beta g(x)^\top g(x^-_{i})}  } \bigg)\bigg) \label{ff} 
 % \\
 % &\leq
\end{align}
We have two terms above. 
Let $\mathcal{C}$ denote the event that $(n_{5}+1)e^{\beta d }+ n_{6}e^{-\beta d } \geq  (n_5+1) e^{\beta(d-2)} +n_6 e^{-\beta(d-2)}$.
We split the first term in \eqref{ff} on $\mathcal{C}$.
\begin{align}
   &  \mathbb{E}_{x,x^+, \{x^-_i\}_{\ell}}  \chi \{x \in B_v,n_4>0,n_{3,v}=0, x^+ \in A\}\nonumber \\
 &\quad \quad \bigg(\log\bigg({  (n_{5}+1)e^{\beta d }+ n_{6}e^{-\beta d } +\sum_{x_i^{-}\not\in {B}_v\cup A} e^{\beta g(x)^\top g(x^-_{i})}  } \bigg) \nonumber \\
    % &\quad \quad  - \mathbb{E}_{x,x^+, \{x^-_i\}_{\ell}}  \chi \{x \in B_v,n_4>0,n_{3,v}=0, x^+ \in A\} \nonumber \\
    &\quad\quad \quad - \log\bigg({  (n_5+1) e^{\beta(d-2)} +n_6 e^{-\beta(d-2)}
 +\sum_{x_i^{-}\not\in {B}_v\cup A} e^{\beta g(x)^\top g(x^-_{i})}  } \bigg)\bigg) \nonumber \\
 &=  \mathbb{E}_{x,x^+, \{x^-_i\}_{\ell}}  \chi \{x \in B_v,n_4>0,n_{3,v}=0, x^+ \in A, \mathcal{C}\}\nonumber \\
 &\quad \quad \bigg(\log\bigg({  (n_{5}+1)e^{\beta d }+ n_{6}e^{-\beta d } +\sum_{x_i^{-}\not\in {B}_v \cup A} e^{\beta g(x)^\top g(x^-_{i})}  } \bigg) \nonumber \\
    &\quad\quad \quad - \log\bigg({  (n_5+1) e^{\beta(d-2)} +n_6 e^{-\beta(d-2)}
 +\sum_{x_i^{-}\not\in {B}_v\cup A} e^{\beta g(x)^\top g(x^-_{i})}  } \bigg)\bigg) \nonumber \\
 &\quad +\mathbb{E}_{x,x^+, \{x^-_i\}_{\ell}}  \chi \{x \in B_v,n_4>0,n_{3,v}=0, x^+ \in A, \mathcal{C}^c\}\nonumber \\
 &\quad \quad \bigg(\log\bigg({  (n_{5}+1)e^{\beta d }+ n_{6}e^{-\beta d } +\sum_{x_i^{-}\not\in {B}_v \cup A} e^{\beta g(x)^\top g(x^-_{i})}  } \bigg) \nonumber \\
    &\quad\quad \quad - \log\bigg({  (n_5+1) e^{\beta(d-2)} +n_6 e^{-\beta(d-2)}
 +\sum_{x_i^{-}\not\in {B}_v\cup A} e^{\beta g(x)^\top g(x^-_{i})}  } \bigg)\bigg) \nonumber \\
  &\leq   \mathbb{E}_{x,x^+, \{x^-_i\}_{\ell}}  \chi \{x \in B_v,n_4>0,n_{3,v}=0, x^+ \in A, \mathcal{C}\}\nonumber \\
 &\quad \quad \bigg(\log\bigg({  (n_{5}+1)e^{\beta d } + ( n_6 + \ell - n_{3,v} - n_4) e^{-\beta d} } \bigg) \nonumber \\
    &\quad\quad \quad - \log\bigg({  (n_5+1) e^{\beta(d-2)} + n_6 e^{-\beta(d-2)} + (\ell - n_{3,v} - n_4) e^{-\beta d}  } \bigg)\bigg) \nonumber \\
 &\quad +\mathbb{E}_{x,x^+, \{x^-_i\}_{\ell}}  \chi \{x \in B_v,n_4>0,n_{3,v}=0, x^+ \in A, \mathcal{C}^c\}\nonumber \\
 &\quad \quad \bigg(\log\bigg({   n_{6}e^{-\beta d } + (n_{5}+1+ \ell - n_{3,v} - n_4) e^{\beta d}  } \bigg) \nonumber \\
    &\quad\quad \quad - \log\bigg({  n_6 e^{-\beta(d-2)}+ (n_5+1) e^{\beta(d-2)} 
 + (\ell - n_{3,v} - n_4) e^{\beta d}  } \bigg)\bigg) \nonumber \\
 &-------------\nonumber \\
 &\leq  \mathbb{E}_{x,x^+, \{x^-_i\}_{\ell}}  \chi \{x \in B_v,n_4>0,n_{3,v}=0, x^+ \in A, \mathcal{C}\} \bigg(\log\bigg({  (n_{5}+1)e^{\beta d }  } \bigg)  - \log\bigg({  (n_5+1) e^{\beta(d-2)}  } \bigg)\bigg) \nonumber \\
  &\leq  2\beta  \mathbb{E}_{x,x^+, \{x^-_i\}_{\ell}}  \chi \{x \in B_v,n_4>0,n_{3,v}=0, x^+ \in A\}  \nonumber 
\end{align}
Similarly, for the second term in \eqref{ff}, we have
\begin{align}
   & \mathbb{E}_{x,x^+, \{x^-_i\}_{\ell}}  \chi \{x \in B_v,n_4>0,n_{3,v}=0, x^+ \notin A\}\nonumber \\
 &\quad \quad \bigg( \log\bigg({  n_{5}e^{\beta d }+ (n_{6}+1)e^{-\beta d } +\sum_{x_i^{-}\not\in {B}_v\cup A} e^{\beta g(x)^\top g(x^-_{i})}  } \bigg) \nonumber \\
    % &\quad \quad  - \mathbb{E}_{x,x^+, \{x^-_i\}_{\ell}}  \chi \{x \in B_v,n_4>0,n_{3,v}=0, x^+ \notin A\} \nonumber \\
    &\quad \quad \quad - \log\bigg({  n_5 e^{\beta(d-2)} +(n_6+1) e^{-\beta(d-2)}
 +\sum_{x_i^{-}\not\in {B}_v\cup A} e^{\beta g(x)^\top g(x^-_{i})}  } \bigg)\bigg) \nonumber \\
 &\leq 2\beta  \mathbb{E}_{x,x^+, \{x^-_i\}_{\ell}}  \chi \{x \in B_v,n_4>0,n_{3,v}=0, x^+ \notin A,\mathcal{C}'\}\nonumber \\ %\\
 % &\quad \quad \bigg( \log\bigg({  n_{5}e^{\beta d }} \bigg) \nonumber \\
 %    % &\quad \quad  - \mathbb{E}_{x,x^+, \{x^-_i\}_{\ell}}  \chi \{x \in B_v,n_4>0,n_{3,v}=0, x^+ \notin A\} \nonumber \\
 %    &\quad \quad \quad - \log\bigg({  n_5 e^{\beta(d-2)}  } \bigg)\bigg) \nonumber \\
  &\leq 2\beta  \mathbb{E}_{x,x^+, \{x^-_i\}_{\ell}}  \chi \{x \in B_v,n_4>0,n_{3,v}=0, x^+ \notin A,n_5 >0\}\nonumber %\\
\end{align}
By summing the upper bounds on the two terms in \eqref{ff}, we obtain
\begin{align}
    ((5)) &\leq 2 \beta \mathbb{P}(x \in B_v)\mathbb{P}(n_4>0, n_{3,v}=0) \nonumber \\
    &= 2 \beta \|B_v\|_\circ (1 - \|B_v\|)^\ell \min(1,\ell \|A\|/(1 - \|B_v\|)).
\end{align}




\item $n_4>0, n_{3,v} > 0$.

We have
\begin{align}
     ((6))&= \mathbb{E}_{x,x^+, \{x^-_i\}_{\ell}}  \chi \{x \in B_v,n_4>0, n_{3,v}>0\} \nonumber \\
     &\quad \bigg( \log\bigg({ e^{\beta g'(x)^\top g'(x^+)}+ n_{3,v}e^{\beta d}+ \sum_{x_i^{-}\in  A} e^{\beta g'(x)^\top g'(x^-_{i})}  +\sum_{x_i^{-}\not\in {B}_v\cup A} e^{\beta g(x)^\top g(x^-_{i})}  } \bigg) \nonumber \\
    &\quad \quad  - \log\bigg({ e^{\beta g(x)^\top g(x^+)}+n_{3,v}e^{\beta d}+ \sum_{x_i^{-} \in A}e^{\beta g(x)^\top g(x^-_{i})} 
 +\sum_{x_i^{-}\not\in {B}_v\cup A} e^{\beta g(x)^\top g(x^-_{i})}  } \bigg)\bigg) \nonumber \\
 &\leq \mathbb{E}_{x,x^+, \{x^-_i\}_{\ell}}  \chi \{x \in B_v,n_4>0, n_{3,v}>0\}  \nonumber \\
 &\quad \bigg(\log\bigg({ e^{\beta g'(x)^\top g'(x^+)}+ n_{3,v}e^{\beta d}+ e^{2\beta }\sum_{x_i^{-}\in  A \setminus C} e^{\beta g(x)^\top g(x^-_{i})}  +\sum_{x_i^{-}\not\in {B}_v\cup A} e^{\beta g(x)^\top g(x^-_{i})}  } \bigg) \nonumber \\
    &\quad \quad  -  \log\bigg({ e^{\beta g(x)^\top g(x^+)}+n_{3,v}e^{\beta d}+ \sum_{x_i^{-} \in A\setminus C}e^{\beta g(x)^\top g(x^-_{i})} 
 +\sum_{x_i^{-}\not\in {B}_v\cup A} e^{\beta g(x)^\top g(x^-_{i})}  } \bigg) \bigg) \nonumber \\
 &\leq  \mathbb{E}_{x,x^+, \{x^-_i\}_{\ell}}  \chi \{x \in B_v,n_4>0, n_{3,v}>0\} \nonumber \\
 &\quad \quad  \bigg(\log\bigg({ e^{\beta g'(x)^\top g'(x^+)}+ (n_{3,v}+n_5)e^{\beta d}\bigg)  -\log\bigg({ e^{\beta g(x)^\top g(x^+)}+n_{3,v}e^{\beta d} + n_{5}e^{\beta (d-2)} } }\bigg)\bigg) %\nonumber 
 % \\
    % &\leq 
\end{align}
Next we split on $x^+\in A$. We have
\begin{align}
    ((6)) &\leq \mathbb{E}_{x,x^+, \{x^-_i\}_{\ell}}  \chi \{x \in B_v,n_4>0, n_{3,v}>0\} \nonumber \\
 &\quad \quad  \bigg(\log\bigg({ e^{\beta g'(x)^\top g'(x^+)}+ (n_{3,v}+n_5)e^{\beta d}\bigg)  -\log\bigg({ e^{\beta g(x)^\top g(x^+)}+n_{3,v}e^{\beta d} + n_{5}e^{\beta (d-2)} } }\bigg)\bigg) \nonumber \\
 &\leq \mathbb{E}_{x,x^+, \{x^-_i\}_{\ell}}  \chi \{x \in B_v,n_4>0, n_{3,v}>0,x^+\in A\}\log(\frac{n_{3,v}+n_5 + 1}{n_{3,v}}) \nonumber \\
 % &\quad \quad  \bigg(\log\bigg({  (n_{3,v}+n_5 + 1)e^{\beta d}\bigg)  -\log\bigg({  (n_{5}+1)e^{\beta (d-2)} } }\bigg)\bigg) \nonumber \\
  &\quad +\mathbb{E}_{x,x^+, \{x^-_i\}_{\ell}}  \chi \{x \in B_v,n_4>0, n_{3,v}>0,x^+\notin A\} \log(\frac{n_{3,v}+n_5}{n_{3,v}})\nonumber \\
 % &\quad \quad  \bigg(\log\bigg({  (n_{3,v}+n_5)e^{2\beta }\bigg)  -\log\bigg({  n_{5} } }\bigg)\bigg) \nonumber \\
 &\leq 2\mathbb{E}_{x,x^+, \{x^-_i\}_{\ell}}  \chi \{x \in B_v,n_4>0, n_{3,v}>0,x^+\in A\}\frac{n_{5}+ 1}{n_{3,v}+1} \nonumber \\
  &\quad +2\mathbb{E}_{x,x^+, \{x^-_i\}_{\ell}}  \chi \{x \in B_v,n_4>0, n_{3,v}>0,x^+\notin A\} \frac{n_{5}}{n_{3,5}+1}\nonumber \\
  &= 2\mathbb{E}_{x,x^+, \{x^-_i\}_{\ell}}  \chi \{x \in B_v,n_4>0, n_{3,v}>0\}\frac{n_5}{n_{3,v}+1} \nonumber \\
  &\quad +2\mathbb{E}_{x,x^+, \{x^-_i\}_{\ell}}  \chi \{x \in B_v,n_4>0, n_{3,v}>0,x^+\in A\} \frac{1}{n_{3,v}+1}\label{gg}
  % \\
  %  &\leq 2\mathbb{E}_{x,x^+, \{x^-_i\}_{\ell}}  \chi \{x \in B_v, n_{3,v}>0\}\frac{n_{3,v}}{n_5+1} \nonumber \\
  % &\quad +2\mathbb{E}_{x,x^+, \{x^-_i\}_{\ell}}  \chi \{x \in B_v,n_{3,v}>0,x^+\in A\} \frac{1}{n_5+1}\nonumber 
\end{align}
For the first term, we have (recall $n_4=n_5+n_6$)
\begin{align}
    &2\mathbb{E}_{x,x^+, \{x^-_i\}_{\ell}}  \chi \{x \in B_v,n_4>0, n_{3,v}>0\}\frac{n_{5}}{n_{3,v}+1} \nonumber \\
    &= 2\| B_v\|_\circ \sum_{n_{3,v},n_5,n_6: n_{3,v}+n_5+ n_6\leq \ell }  \chi \{n_{3,v} > 0, n_5 > 0\} \binom{\ell}{n_{3,v}~n_5~n_6~1\!-\!n_{3,v}\!-\!n_5\!-\!n_6} \nonumber \\
    &\quad \quad \quad \quad  \Vert B_v\Vert^{n_{3,v}} \Vert A\setminus C\Vert^{n_5} \Vert A\cap C\Vert^{n_6} (1 - \Vert A\cup B_v\Vert)^{1-n_{3,v}-n_5 - n_6}\frac{n_5}{n_{3,v}+1} \label{one}\\
    &\leq 2{\|A\setminus C\|}\sum_{0 \leq n_{3,v}+1 \leq \ell,0\leq n_5-1\leq \ell,0\leq n_6\leq \ell}  \binom{\ell}{n_{3,v}+1~n_5-1~n_6~1\!-\!n_{3,v}\!-\!n_5\!-\!n_6} \nonumber \\
    &\quad \quad \quad \quad  \Vert B_v\Vert^{n_{3,v}+1} \Vert A\setminus C\Vert^{n_5-1} \Vert A\cap C\Vert^{n_6} (1 - \Vert A\cup B_v\Vert)^{1-n_{3,v}-n_5 - n_6} \label{two}\\
    % &= 2\mathbb{P}(x \in A_v)\sum_{n_{1,v},n_2: n_{1,v},n_2>0, n_{1,v}+n_2\leq \ell}  \binom{l}{n_{1,v}~n_2~1\!-\!n_{1,v}\!-\!n_2} \nonumber \\
    % &\quad \quad \quad \quad \Vert A_v\Vert_\circ^{n_{1,v}}\Vert B\Vert_\circ^{n_2}\Vert 1-A_v-B\Vert_\circ^{1-n_{1,v}-n_2}\frac{n_2}{n_{1,v}+1} \\
    % &= 2 D_g(v) \frac{\|B\|_\circ}{\|A_v\|_\circ} \sum_{n_{1,v},n_2: n_{1,v},n_2>0, n_{1,v}+n_2\leq \ell}    \binom{l}{n_{1,v}+1~n_2-1~1\!-\!n_{1,v}\!-\!n_2} \nonumber \\
    % &\quad \quad \quad \quad \Vert A_v\Vert_\circ^{n_{1,v}+1}\Vert B\Vert_\circ^{n_2-1}\Vert 1-A_v-B\Vert_\circ^{1- n_{1,v}-n_2} \\
    % &\leq 2 D_g(v) \frac{\|B\|_\circ}{\|A_v\|_\circ} \!\sum_{n_{1,v}\!+\!1,n_2\!-\!1: n_{1,v}\!+\!1,n_2-\!1\!\geq\!0, n_{1,v}+1\!+\!n_2-1\!\leq\! \ell}   \binom{l}{n_{1,v}\!+\!1~n_2\!-\!1~1\!-(n_{1,v}\!+\!1) \!-\! (n_2\!-\!1)}\nonumber \\
    % &\quad \quad \quad \quad \quad \quad \quad \quad \quad \quad \quad\quad \quad \quad \quad  \quad \quad \quad \quad  \quad \quad \quad \Vert A_v\Vert_\circ^{n_{1,v}\!+\!1}\Vert B\Vert_\circ^{n_2\!-\!1}\Vert 1\!-\!A_v\!-\!B\Vert_\circ^{1 \!-\! (n_{1,v}\!+\!1)\! -\! (n_2\!-\!1)}  \label{sq}\\
    % &= 2{\|B\|_\circ} ( \Vert A_v\Vert_\circ + \Vert B\Vert_\circ + \Vert 1-A_v-B\Vert_\circ)^\ell  \nonumber \\
    % &= {2 {\|B\|_\circ}}   \nonumber 
    &= 2{\|A\setminus C\|}
\end{align}
where \eqref{two} follows {\color{blue} assuming $\|B_v\|_\circ = \|B_v\|$, or $x$ and $x_i^-$ are drawn from the same distribution.}
Note that since $n_5>0$ for all nonzero terms, we are not subtracting a term with $n_{3,v}=\ell$ to go from \eqref{one} to \eqref{two}. % (nor are we subtracting a term with $n_5=0$).
For the second term in \eqref{gg}, we have 
\begin{align}
    &2\mathbb{E}_{x,x^+, \{x^-_i\}_{\ell}}  \chi \{x \in B_v,n_4>0, n_{3,v}>0,x^+\in A\} \frac{1}{n_{3,v}+1} \nonumber \\
    &\leq \mathbb{E}_{x,x^+, \{x^-_i\}_{\ell}}  \chi \{x \in B_v,n_4>0, n_{3,v}>0,x^+\in A\} \nonumber \\
    &\leq \mathbb{P}(x\in B_v, x^+\in A)
\end{align}
So in total for this case, we have
\begin{align}
    ((6)) &\leq 2{\|A\setminus C\|} +\mathbb{P}(x\in B_v, x^+\in A)
\end{align}



\end{enumerate}




























Combining all three cases and summing over $v\in \mathcal{H}_d$ yields [{\color{red}note: the analysis above can be tightened if $\beta$ is small}]

\begin{align*}
&\mathcal{L}_{\text{neg}}(g') -\mathcal{L}_{\text{neg}}(g)\nonumber \\
&\le \sum_{v \in \mathcal{H}_d} \mathbb{P}(x \in A_v \cap x^+ \in B) \left( 2 \beta (1 - \|A_v\| - \|B\|)^\ell + \log(2) \min(1, \frac{\ell \|A_v\|}{1-\|B\|}) (1- \|B\|)^\ell\right)\nonumber\\
&\quad + 2 \beta   \|A_v\|_\circ (1 - \|A_v\|)^\ell \min\left(1, \frac{\ell \|B\|}{1- \|A_v\|}\right) \nonumber \\
&\quad + 2 \|B\| +   \mathbb{P}  \left[x \in A_v, x^+\in B\right] \nonumber \\
&\quad + \mathbb{P}(x \in B_v \cap x^+ \in A)\left(2\beta (1 - \|B_v\| - \|A\|)^\ell  + \log(2)\min( 1, \frac{\ell \|B_v\|}{1 - \|A\|})  (1 - \|A\|)^\ell\right)\nonumber \\
&\quad + 2 \beta \|B_v\|_\circ (1 - \|B_v\|)^\ell \min(1,\ell \|A\|/(1 - \|B_v\|))\nonumber \\
&\quad + 2{\|A\setminus C\|} +\mathbb{P}(x\in B_v, x^+\in A) \nonumber \\
&= \|R\| + 2^{d+1} (\|B\|+\|A\setminus C\|) \nonumber \\
&\quad + \sum_{v \in \mathcal{H}_d} \bigg(\mathbb{P}(x \in A_v \cap x^+ \in B)\left( 2 \beta (1 - \|A_v\| - \|B\|)^\ell + \log(2) \min(1, \frac{\ell \|A_v\|}{1-\|B\|}) (1- \|B\|)^\ell\right)\nonumber\\
&\quad + 2 \beta \|A_v\|_\circ (1 - \|A_v\|)^\ell \min\left(1, \frac{\ell \|B\|}{1- \|A_v\|}\right) \nonumber \\
&\quad + \mathbb{P}(x \in B_v \cap x^+ \in A)\left(2\beta (1 - \|B_v\| - \|A\|)^\ell  + \log(2)\min( 1, \frac{\ell \|B_v\|}{1 - \|A\|})  (1 - \|A\|)^\ell\right)\nonumber \\
&\quad + 2 \beta \|B_v\|_\circ (1 - \|B_v\|)^\ell \min(1,\ell \|A\|/(1 - \|B_v\|))\bigg) \nonumber \\
&\leq 2\|R\| + 2^{d+1} (\|B\|+\|A\setminus C\|) \nonumber \\
&\quad + 2 \beta \sum_{v \in \mathcal{H}_d} \bigg(\mathbb{P}(x \in A_v \cap x^+ \in B) (1 - \|A_v\| - \|B\|)^\ell+ \mathbb{P}(x \in B_v \cap x^+ \in A) (1 - \|B_v\| - \|A\|)^\ell \nonumber\\
&\quad +  \|A_v\|_\circ (1 - \|A_v\|)^\ell \min\left(1, \frac{\ell \|B\|}{1- \|A_v\|}\right) +  \|B_v\|_\circ (1 - \|B_v\|)^\ell \min(1,\ell \|A\|/(1 - \|B_v\|))\bigg) \nonumber \\
\end{align*}
If $\|R\|$ is a constant then we are done. in general we need $\beta$ and $\ell$ to scale inversely with $\|R\|$.

If $\beta$ is small, then we can tighten the above bound. The first line is most important (from cases 3 and 6). 









----------------------------


% \begin{align*}
% \mathcal{L}_{\text{neg}}(g') -\mathcal{L}_{\text{neg}}(g)
% &\le \sum_{v \in \mathcal{H}_d}  \mathbb{P}(x \in A_v,x^+ \in B) \bigg( 2 \beta \|A_v\|_\circ(1 - \|A_v\|_\circ - \|B\|_\circ)^\ell + \log(2) \|A_v\|_\circ\bigg) \nonumber \\
% &\quad + 2 \beta \ell \log(\ell+1) \|A_v\|_\circ (1 - \|A_v\|_\circ)^\ell  \mathbb{P} ( x_{1}^- \in B |  x_{1}^- \notin A_v) \nonumber \\
% &\quad + 2 \|B\|_\circ \chi\{ A_v\cap B = \emptyset \} + 2 \chi\{\|A_v\!\setminus\! B\|_\circ \geq \|A_v\|_\circ/2\}({\Vert A_v\cap B\Vert_\circ+ 2\Vert B\setminus A_v\Vert_\circ }) \nonumber \\
%     &\quad +  4 \chi\{\|A_v\!\setminus\! B\|_\circ \geq \|A_v\|_\circ/2\}\frac{\Vert A_v\cap B\Vert_\circ^2 + 2 \Vert A_v\cap B\Vert_\circ\Vert B\setminus A_v\Vert_\circ}{\Vert A_v\Vert_\circ} \nonumber \\
%     &\quad + 8 \ell \Vert  A_v\cap B\Vert_\circ {\Vert B\setminus A_v\Vert_\circ}  (1 - \Vert  A_v\Vert_\circ/2)^{\ell} \chi \{ \|A_v\!\cap\! B\|_\circ \geq \|A_v\|_\circ/2\} \nonumber \\
%     &\quad +4 \|A_v\cap B\|_\circ \left(2\frac{\Vert B\setminus A_v\Vert_\circ}{\Vert A_v\Vert_\circ}+1\right)\chi \{\|A_v\!\cap\! B\|_\circ \geq \|A_v\|_\circ/2\} \nonumber \\
%     &\quad + \chi\{A_v\cap B= \emptyset \} \mathbb{P}  \left[x \in A_v, x^+\in B\right] + \chi\{A_v\cap B\neq \emptyset \} \mathbb{P}  \left[x \in A_v \cap B, x^+ \notin B \right] \nonumber \\
%     &\leq  \sum_{v \in \mathcal{H}_d}  \|A_v \cap B\|_\circ \|A_v\|_\circ\bigg( 2 \beta (1 - \|A_v\|_\circ - \|B\|_\circ)^\ell + \log(2) \bigg) \nonumber \\
% &\quad + 2 \beta \ell \log(\ell+1)  \sum_{v \in \mathcal{H}_d} \|A_v\|_\circ (1 - \|A_v\|_\circ)^\ell  \mathbb{P} ( x_{1}^- \in B |  x_{1}^- \notin A_v) \nonumber \\
%     &\quad + (2*2^{d} + 4*2^{d} + 4*2*2^d) \|B\|_\circ\nonumber \\
%     &\quad + 8\ell \sum_{v \in \mathcal{H}_d} \Vert  A_v\cap B\Vert_\circ {\Vert B\setminus A_v\Vert_\circ}  (1 - \Vert  A_v\Vert_\circ/2)^{\ell} \chi\{\|A_v\!\cap\! B\|_\circ \geq \|A_v\|_\circ/2 \} \nonumber \\
%     &\quad + 8 \sum_{v \in \mathcal{H}_d} \Vert B\setminus A_v\Vert_\circ \chi \{\|A_v\!\cap\! B\|_\circ \geq \|A_v\|_\circ/2\} \nonumber \\
%     &\quad + 4 \sum_{v \in \mathcal{H}_d} \Vert  A_v \cap B\Vert_\circ \chi \{\|A_v\!\cap\! B\|_\circ \geq \|A_v\|_\circ/2\} \nonumber \\
%     &\quad \sum_{v\in \mathcal{H}_d} \chi\{A_v\cap B= \emptyset \} \mathbb{P}  \left[x \in A_v, x^+\in B\right] + \chi\{A_v\cap B\neq \emptyset \} \mathbb{P}  \left[x \in A_v \cap B, x^+ \notin B \right] \nonumber \\
%     &\leq 27*2^d \|B\|_\circ  + 2 \beta (\ell \log(\ell+1) +1) \|B\|_\circ  \sum_{v \in \mathcal{H}_d} \|A_v\|_\circ (1 - \|A_v\|_\circ)^\ell  \nonumber \\
%     &\quad + 8\ell \|B\|_\circ \sum_{v \in \mathcal{H}_d} \Vert  A_v\Vert_\circ   (1 - \Vert  A_v\Vert_\circ/2)^{\ell}  \nonumber \\
%     &\quad \underbrace{\sum_{v\in \mathcal{H}_d} \chi\{A_v\cap B= \emptyset \} \mathbb{P}  \left[x \in A_v, x^+\in B\right] + \chi\{A_v\cap B\neq \emptyset \} \mathbb{P}  \left[x \in A_v \cap B, x^+ \notin B \right]}_{\text{area of shaded region}} \nonumber %\\
%     % &\leq 
%     % \sum_{v \in \mathcal{H}_d}\chi\{\Vert B\setminus A_v\Vert_\circ \}
%     % &\leq 27*2^d \|B\|_\circ  + 2 \beta (\ell \log(\ell+1) +1)  e^{-\ell 2^{-d} } \|B\|_\circ   + 8\ell  e^{-\ell 2^{-d-1} }  \|B\|_\circ \nonumber \\
%     % &\quad \underbrace{\sum_{v\in \mathcal{H}_d} \chi\{A_v\cap B= \emptyset \} \mathbb{P}  \left[x \in A_v, x^+\in B\right] + \chi\{A_v\cap B\neq \emptyset \} \mathbb{P}  \left[x \in A_v \cap B, x^+ \notin B \right]}_{\text{area of shaded region}} \nonumber \\
% \end{align*}

% If all $\|A_v\|_\circ \geq c 2^{-d}$ then:

We are done if we set  $\beta = \Omega(2^d)$, $\ell = \Omega(d 2^d)$, and upper bound $\|B_\circ\|$ in terms of shaded region.


Note that we cannot do the latter by some property of the closest $g'$ to $g$, since we have used a $g'$ that is not necessarily closest to $g$. Let $R$ be the shaded region.
Suppose that 
% $\|B\|_\circ \leq 2 \|S\| $. 
% Then the upper bound on the negative term is
% \begin{align}
%   \tilde{L}_{\text{neg}}(g') -\tilde{L}_{\text{neg}}(g)
% &\le   55*2^d \|S\|  + 4 \beta (\ell \log(\ell+1) +1)  e^{-\ell 2^{-d} } \|S\|   + 8\ell  e^{-\ell 2^{-d-1} }  \|S\| \nonumber 
% \end{align}
%  Suppose $\ell = C d 2^d$ and $\beta = 110 * 2^d$. Then 
%  \begin{align}
%   \tilde{L}_{\text{neg}}(g') -\tilde{L}_{\text{neg}}(g)
% &\le   55*2^d \|S\|  + 8 \beta Cd^2  \log(Cd)  e^{-(C-1)d } \|S\|   + 8Cd 2^d  e^{-Cd/2 }  \|S\| \nonumber \\
% &\leq \beta \|S\| \left( \frac{1}{2}  + 8  Cd^2  \log(Cd)  e^{-(C-1)d }    + \frac{1}{11} Cd  e^{-Cd/2 } \right) \nonumber \\
% &\stackrel{*}{\leq} \beta \|S\|  \nonumber
% \end{align}
% where $*$ holds iff
% \begin{align}
%     &8  Cd^2  \log(Cd)  e^{-(C-1)d }    + \frac{1}{11} Cd  e^{-Cd/2 } \leq 1/2 \nonumber
% \end{align}
% Worst case is $d=1$. Then
% \begin{align}
%     &8  C  \log(C)  e^{-(C-1) }    + \frac{1}{11} C  e^{-C/2 } \leq 1/2 \nonumber \\ 
% \end{align}
% One can check that $C\geq 6$ is sufficient. 
% For
$\|B\|_\circ \leq \eta \|R\| $ for some $\eta>0$\footnote{Need to formalize this assumption}. Then if $\|A_v\|_\circ = 2^{-d}$ for all $v$, the upper bound on the difference of negative terms is
\begin{align}
  \mathcal{L}_{\text{neg}}(g') -\mathcal{L}_{\text{neg}}(g)
&\le   (27\eta*2^d+1) \|R\|  + 2 \beta \eta (\ell \log(\ell+1) +1)  e^{-\ell 2^{-d} } \|R\|   + 4\eta \ell  e^{-\ell 2^{-d-1} }  \|R\| \nonumber 
\end{align}
 Let $\ell = C d 2^d$ and $\beta = 4*28*\eta * 2^d$. Then 
 \begin{align}
  \mathcal{L}_{\text{neg}}(g') -\mathcal{L}_{\text{neg}}(g)
&\le  (27\eta*2^d+1) \|R\|   + 4\eta  \beta Cd^2  \log(Cd)  e^{-(C-1)d } \|R\|   + 4\eta Cd 2^d  e^{-Cd/2 }  \|R\| \nonumber \\
&\leq \beta \|R\| \left( \frac{1}{2}  + 4\eta   Cd^2  \log(Cd)  e^{-(C-1)d }    + \frac{\eta}{28} Cd  e^{-Cd/2 } \right) \nonumber \\
&\stackrel{*}{\leq} \beta \|R\|  \nonumber
\end{align}
where $*$ holds iff
\begin{align}
    &4\eta   Cd^2  \log(Cd)  e^{-(C-1)d }    + \frac{\eta}{28} Cd  e^{-Cd/2 }\leq 1/2 \nonumber
\end{align}
The worst case is $d=1$. Then
\begin{align}
    &4\eta   C  \log(C)  e^{-(C-1) }    + \frac{\eta}{28} C e^{-C/2 }\leq 1/2 \nonumber \\ 
\end{align}
One can check that $C\geq 6\log(\eta)$ is sufficient. 

Recall that for the positive gain we have $\mathcal{L}_{\text{pos}}(g') -\mathcal{L}_{\text{pos}}(g)\leq -2\beta \|R\|$, completing the proof.

{\color{blue}
The key is upper bounding $\sum_{v \in \mathcal{H}_d} \|A_v\|_\circ (1 - \|A_v\|_\circ)^\ell $.
The largest term scales as $\beta \ell \log(\ell)\sum_{v \in \mathcal{H}_d} \|A_v\|_\circ (1 - \|A_v\|_\circ)^\ell $, corresponding to the case $n_{1,v}=0$ and $n_2>0$.
As long as $\|A_v\|_\circ > \frac{\log(d)}{cd2^d}$ or $\|A_v\|_\circ \leq \frac{\log(d)}{C d^2 2^{2d}}$ for all $v\in \mathcal{H}_d$,\footnote{Corresponding to the cases that $A_v$ is large enough such that there are likely other $e^{\beta d}$ terms in the log to offset terms that may go from $e^{\beta(d-2)}$ to $e^{\beta d}$ for $x_{i}^-$, or $A_v$ is small enough such that it is highly unlikely that $x \in A_v$.} then $\sum_{v \in \mathcal{H}_d} \|A_v\|_\circ (1 - \|A_v\|_\circ)^\ell $ is sufficiently small, for some numerical constants $C,c$. Otherwise, there exists a scenario in which both of the two possible $f_1'$ adjacent to $f_1$ result in $g'$ that has larger loss than $g$. In this case the representation can be improved, but not by substituting one of two adjacent cleaner classifiers. The challenge is formalizing which $g'$ one should pick in all cases...

Alternatively, we can choose $\beta_2 = o(1)$ and $\beta_2 = \Omega(4^d)$ to show that the positive difference is larger than the negative difference. 
But this is not aligned with practice...
}

% Overall, for case $\circled{1}$, this gives a total 
% \begin{align*}
% 0\cdot\Pr[\circled{1a}]+2\beta \Pr[\circled{1b}] + \frac{\Vert B\Vert_\circ}{\Vert A\Vert_\circ} \Pr[\circled{1c}]=2\beta \sum_{i\in \uH^d} D_g(i)\left(1-D_g(i)\right)^ll\delta + 2\frac{\Vert B\Vert_\circ}{\Vert A\Vert_\circ}
% \end{align*}








\end{proof}
